# Supplementary material for: A Contrast Based Feature Selection Algorithm for High-dimensional Data set in Machine Learning
Source: arXiv:2401.07482 source file (2024-01-15)
Supplement: Supplementary file 1 [file appendix.tex]

\appendix 

\part*{Appendix}
In this section, we report the experiment results when execute ContrastFS on benchmark data sets.

\section{Time consuming}
Although we have shown the great advantages of our approach in terms of operational efficiency in the text, it makes sense to describe it from more angles.

As shown in the text, our method runs really fast meanwhile achieves good performance, that means the unit performance gain of our method is much higher than other methods.

\section{Accuracy}

\subsection{when ExtremeTree and RandomForest as Classifier}
We implement experiments on several benchmark datasets to inspect the effectiveness of our method. We select feature subset from each dataset then feed them into consequent classifiers, we have shown the best accuracy achieved by XGBoost and 1-hidden-layer neural network trained on features selected by our methods in main body. 

Here we shown the results according to the rest two classifiers, ExtremeTrees and RandomForest in figure \ref{the_highest_accuracy_xtreerf}.
To achieve this performance, we try to split datasets uniformly in statistical sense, e.g., try to control the distributional difference between train and test set.
\begin{remark}
It equals to report the best result in multiple runs, as we obtain the most uniform train set and test set from random split.
\end{remark}

\begin{figure}[!h]
	\centering
	%\vspace{-2cm}
	%\hspace{-2cm}
	\begin{subfigure}[b]{0.48\textwidth}
		\includegraphics[width=\textwidth]{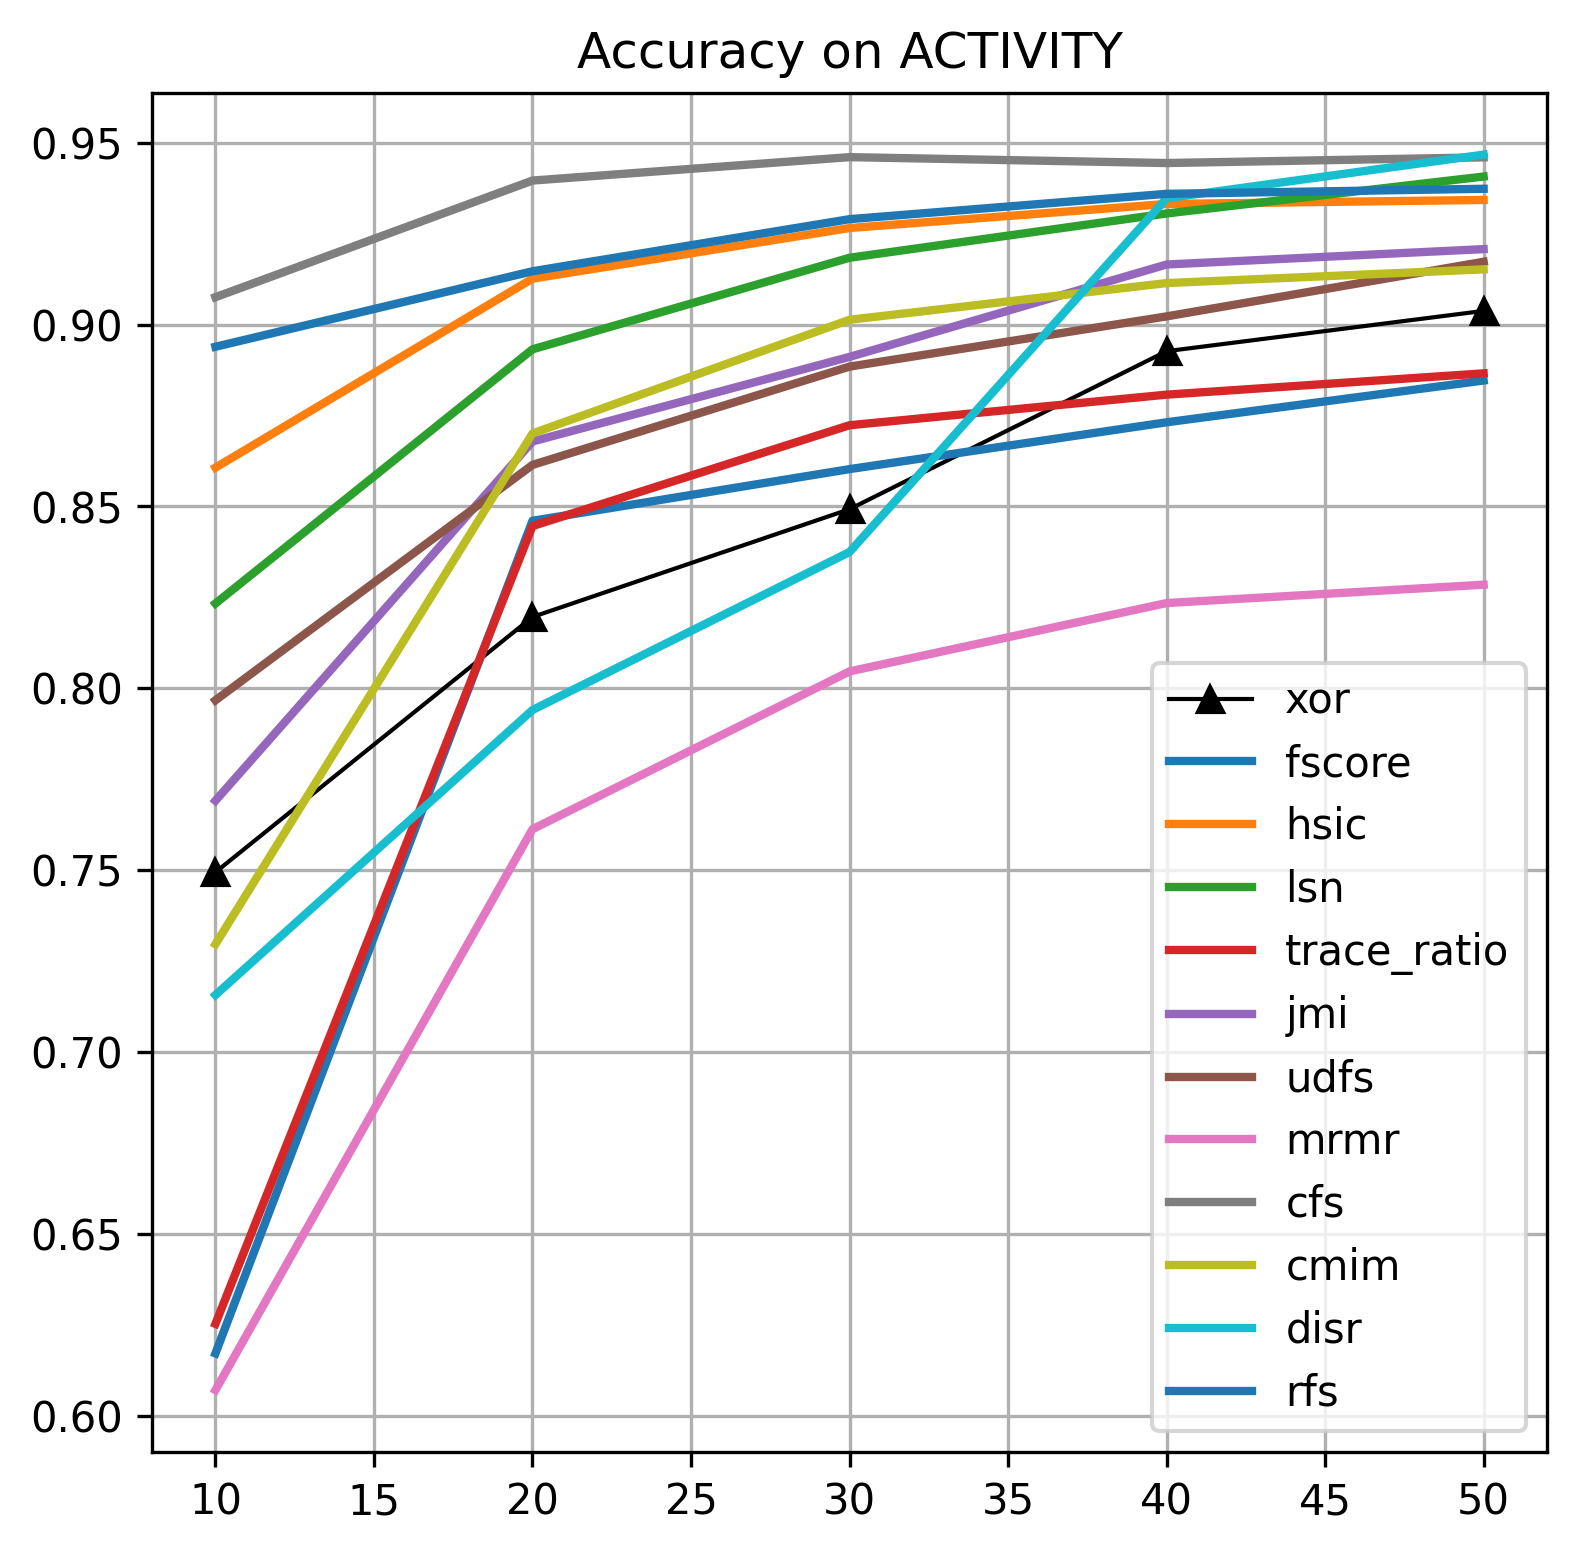} 
		\caption{}

	\end{subfigure}
	\begin{subfigure}[b]{0.48\textwidth}
		\includegraphics[width=\textwidth]{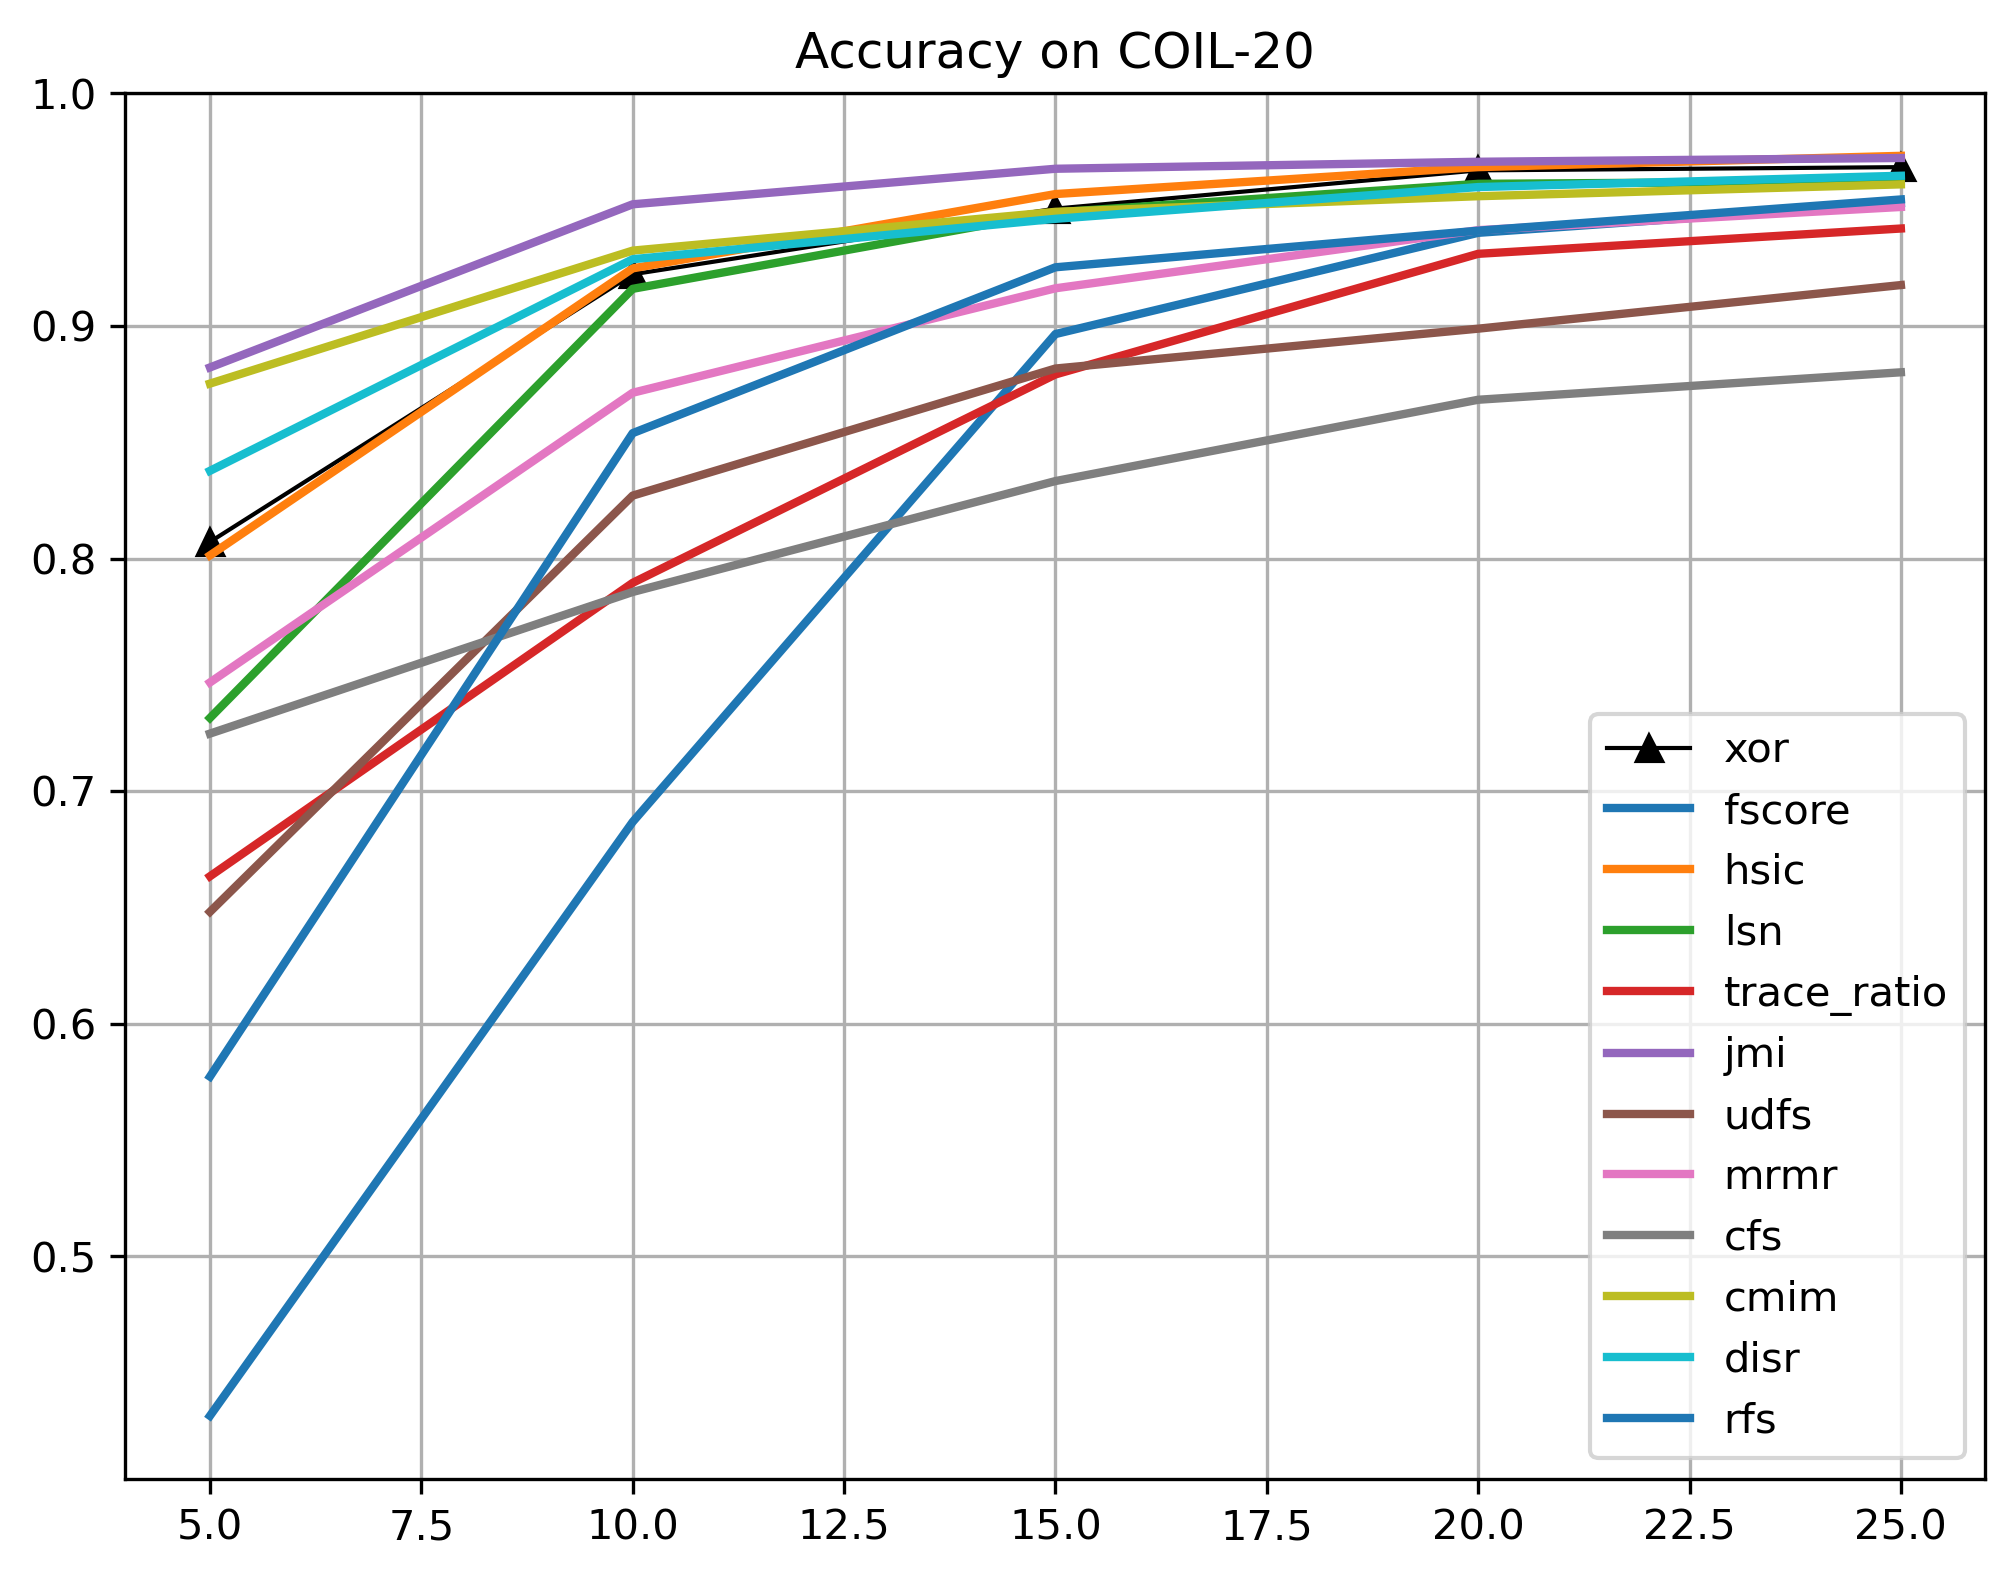}
		\caption{}

	\end{subfigure}
	\begin{subfigure}[b]{0.48\textwidth}
		\includegraphics[width=\textwidth]{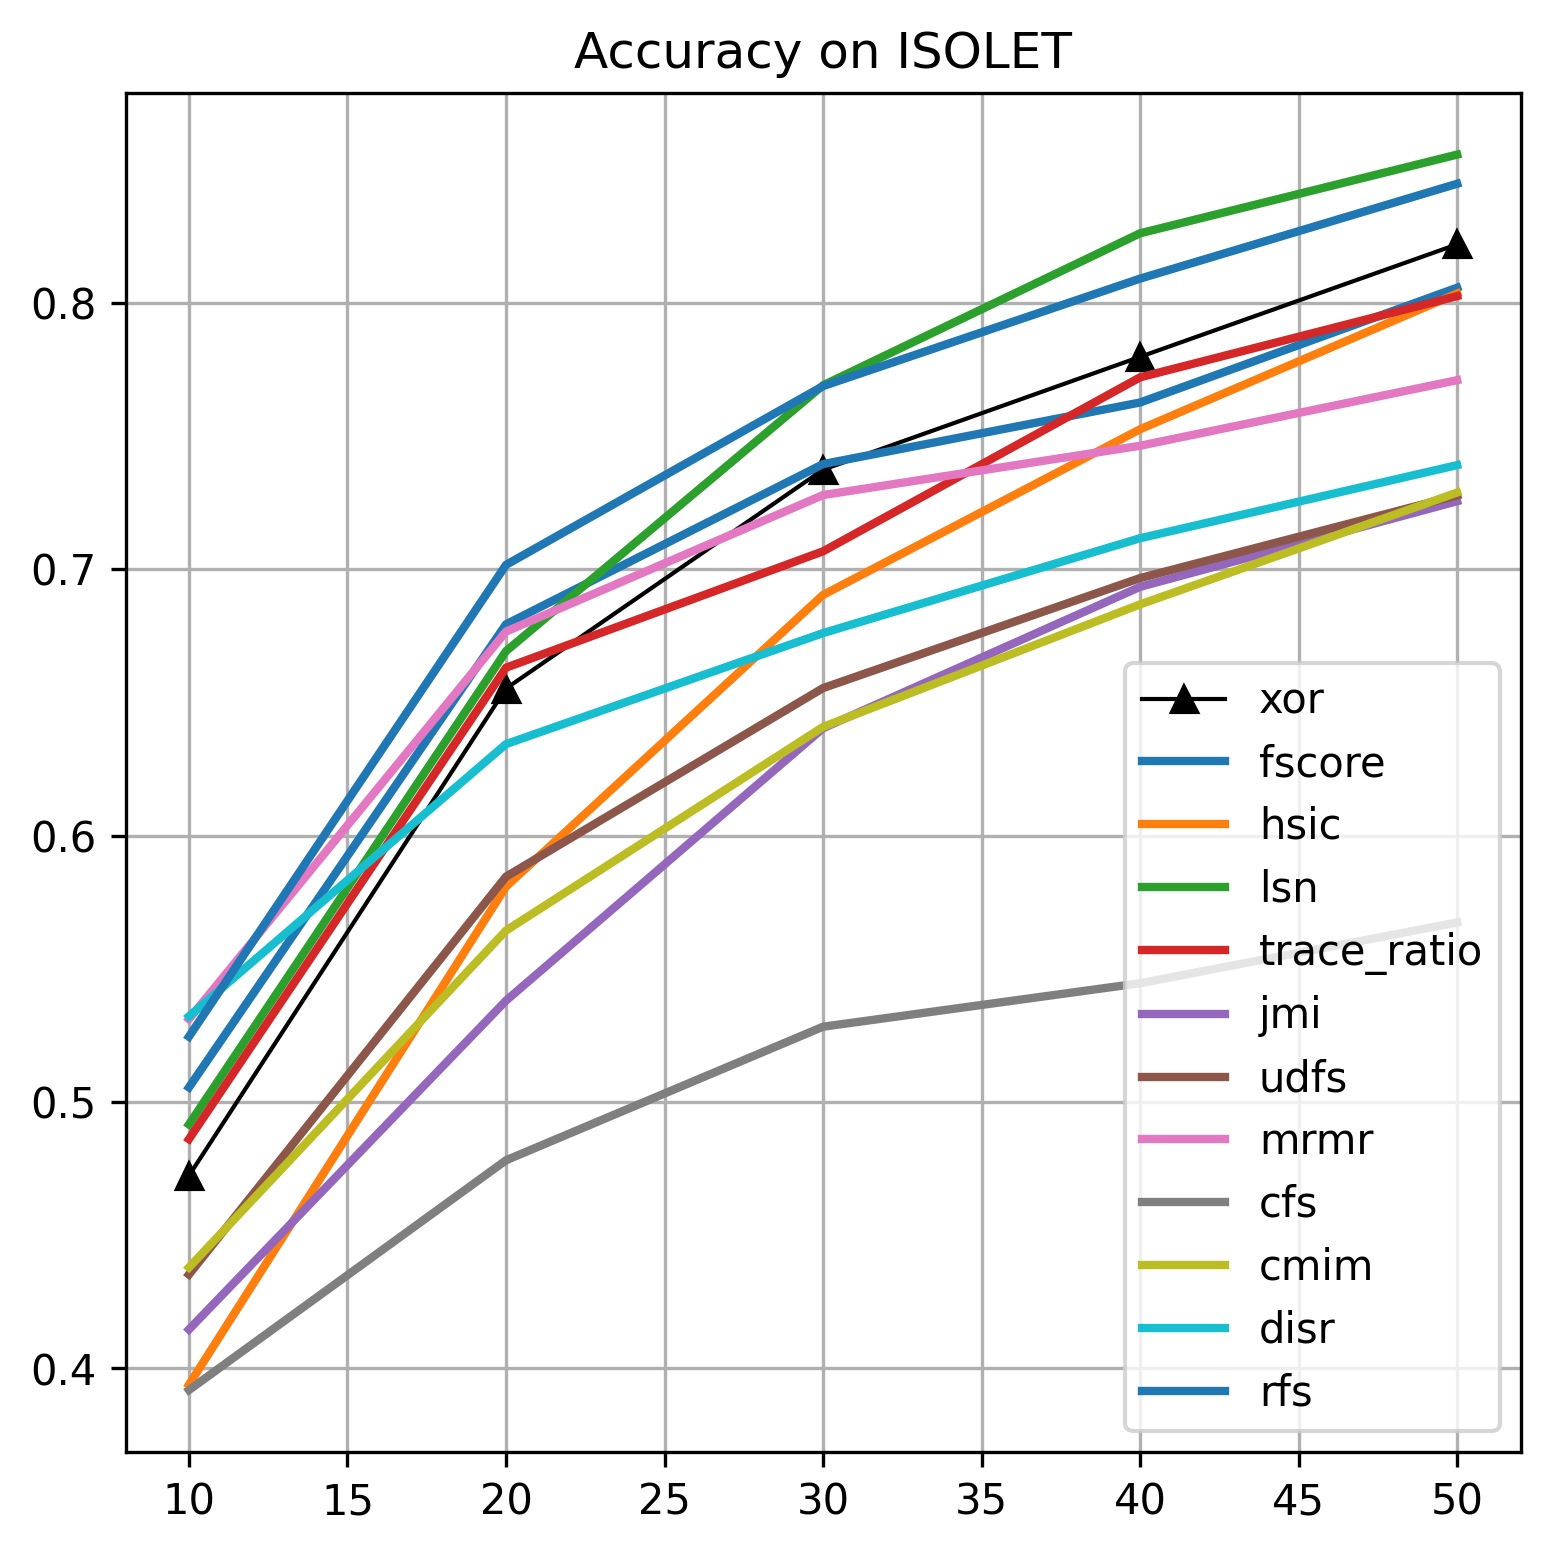}
		\caption{}

	\end{subfigure}
	~ %add desired spacing between images, e. g. ~, \quad, \qquad, \hfill etc.
	% set the trim={0 0 0 1cm},clip in \includegraphics{imagefile}[options] options
	%(or a blank line to force the subfigure onto a new line)
	\begin{subfigure}[b]{0.48\textwidth}
		\includegraphics[width=\textwidth]{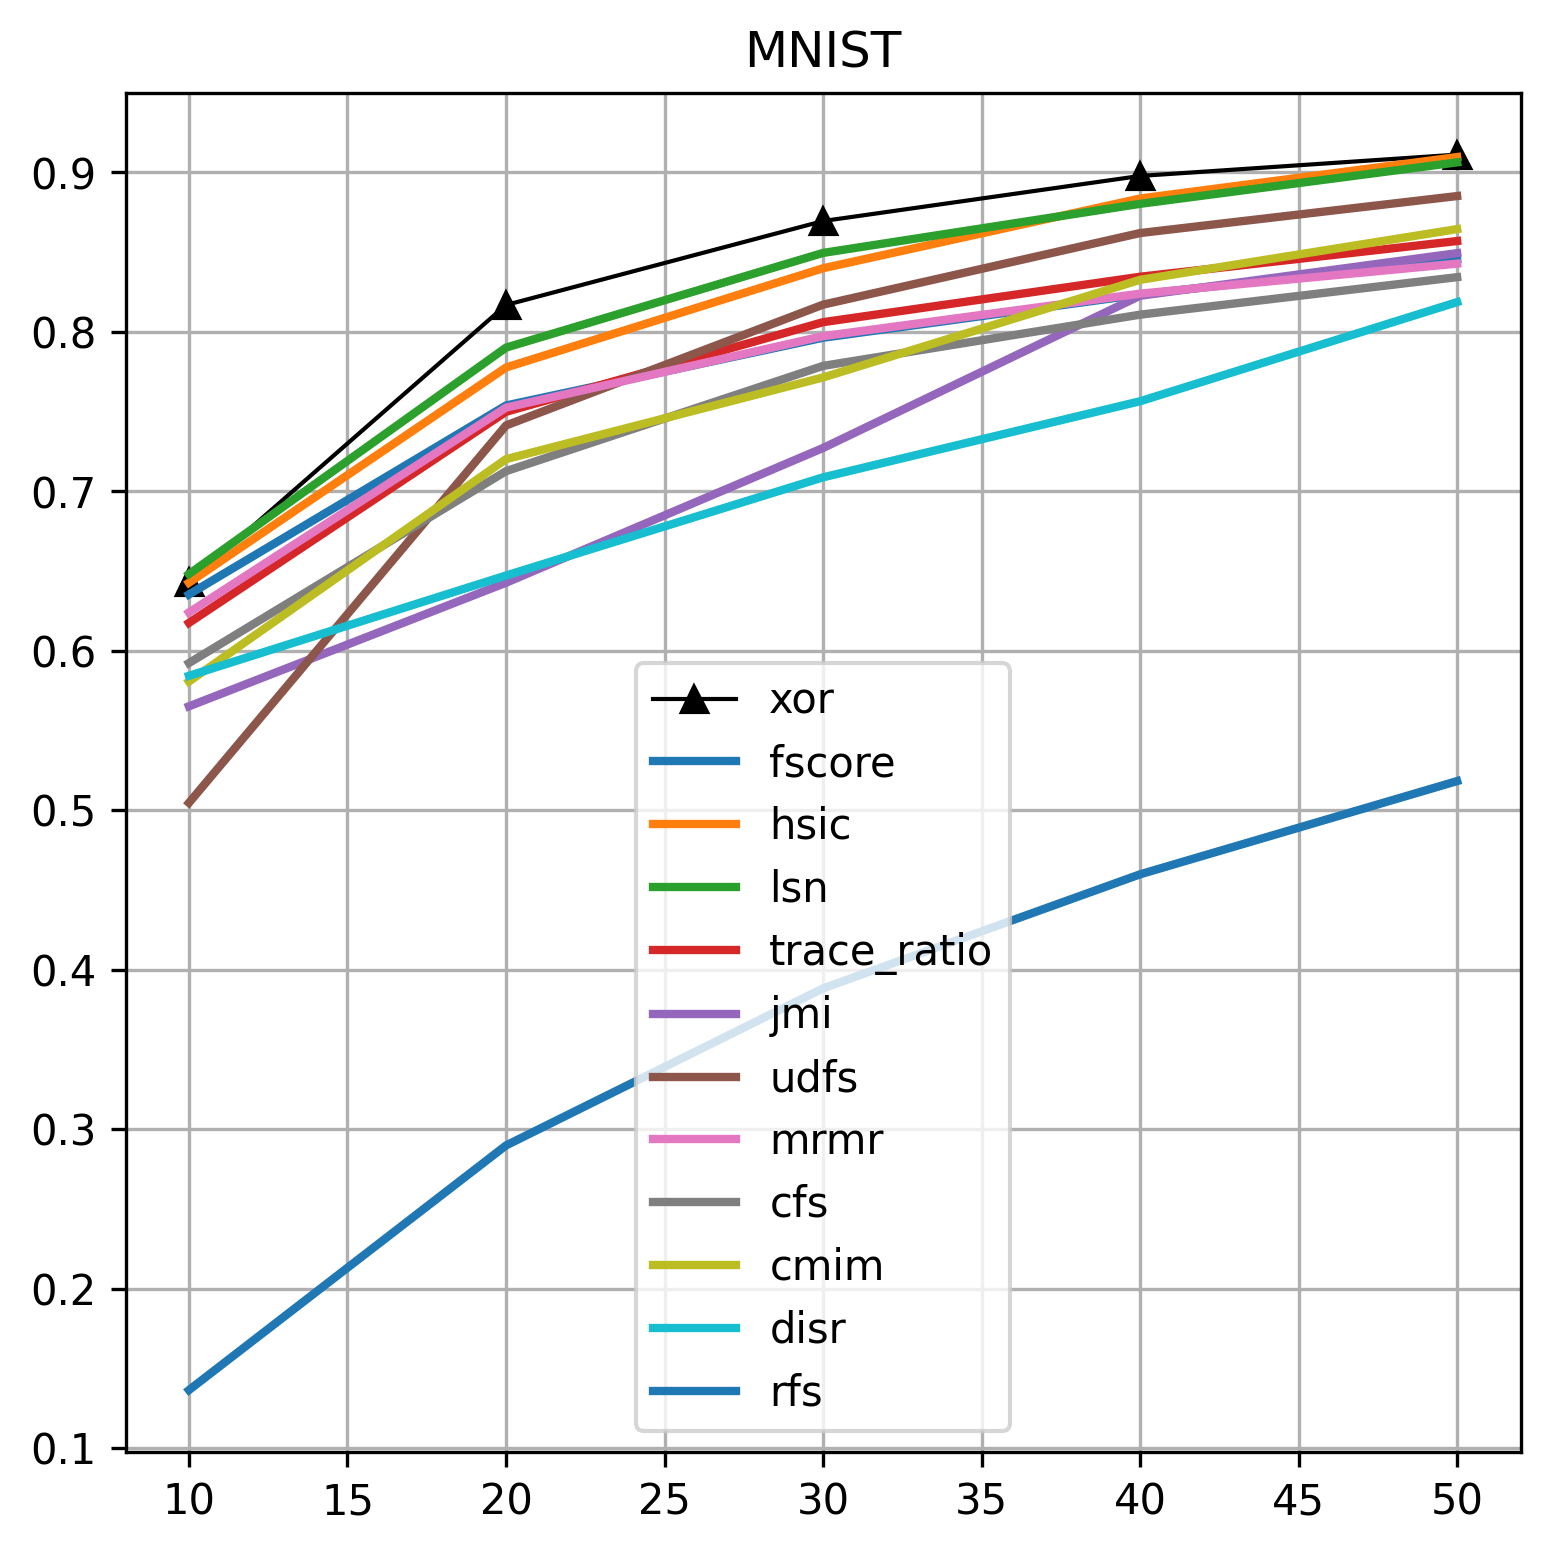}
		\caption{}

	\end{subfigure}
	\begin{subfigure}[b]{0.48\textwidth}
		\includegraphics[width=\textwidth]{pic/mnist_acc_xgb.png}
		\caption{}

	\end{subfigure}
	\begin{subfigure}[b]{0.48\textwidth}
		\includegraphics[width=\textwidth]{pic/mnist_acc_xgb.png}
		\caption{}

	\end{subfigure}
	
	\caption{The highest accuracy when ExtreemTrees and RandomForest as classifier.}
	\label{the_highest_accuracy_xtreerf}
\end{figure}

Our method shows excellent trade-off on accuracy and running time, we show this advantage here for ExtremeTree and RandomForest as classifier in figure \ref{the_highest_accuracy_time_xtreerf}.

\begin{figure}[!h]
	\centering
	%\vspace{-2cm}
	%\hspace{-2cm}
	\begin{subfigure}[b]{0.48\textwidth}
		\includegraphics[width=\textwidth]{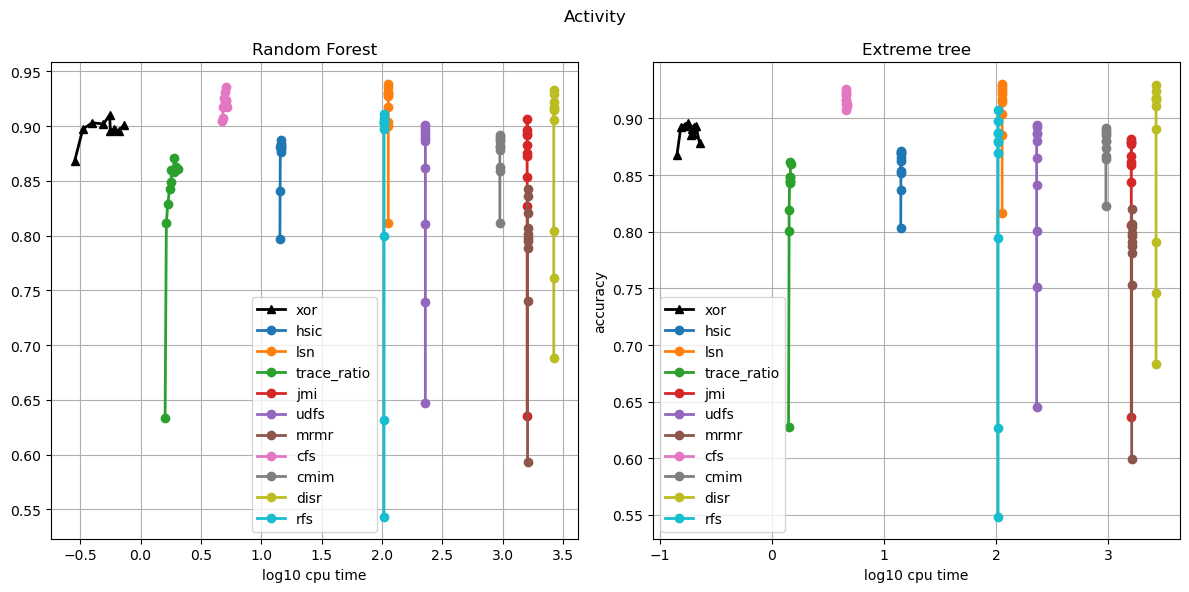} 
		\caption{}
		
	\end{subfigure}
	\begin{subfigure}[b]{0.48\textwidth}
		\includegraphics[width=\textwidth]{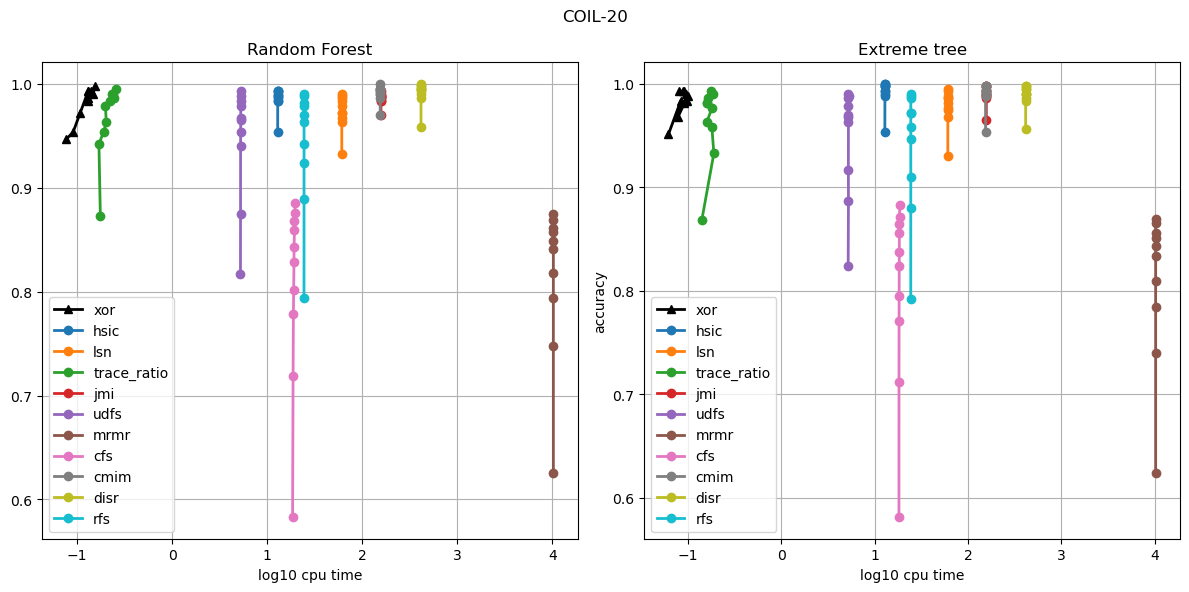}
		\caption{}
		
	\end{subfigure}
	\begin{subfigure}[b]{0.48\textwidth}
		\includegraphics[width=\textwidth]{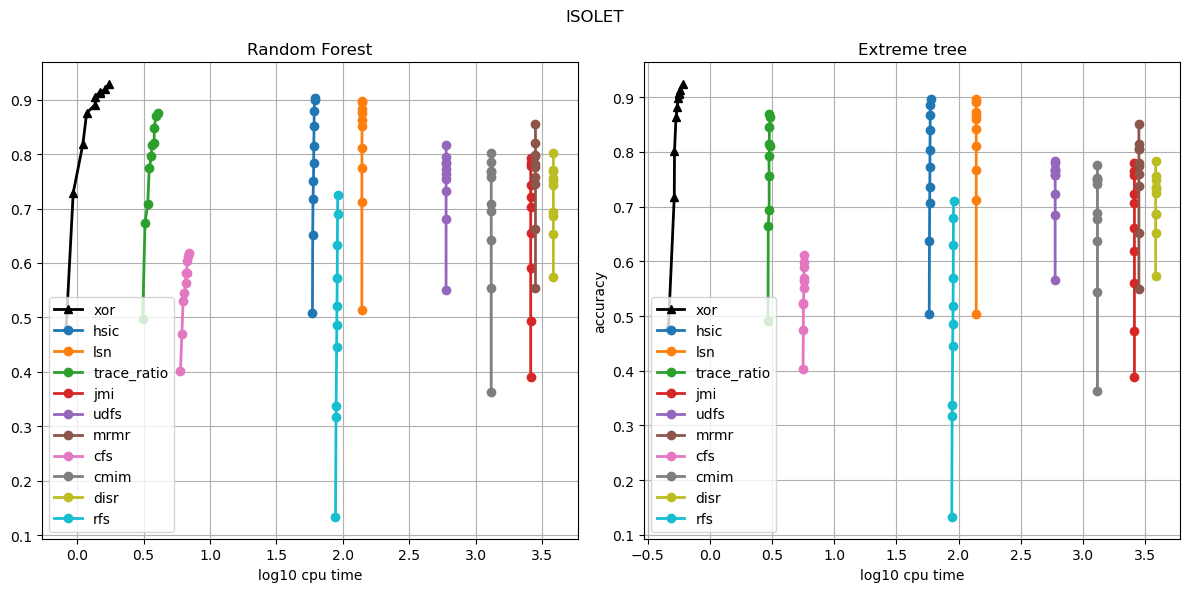}
		\caption{}
		
	\end{subfigure}
	~ %add desired spacing between images, e. g. ~, \quad, \qquad, \hfill etc.
	% set the trim={0 0 0 1cm},clip in \includegraphics{imagefile}[options] options
	%(or a blank line to force the subfigure onto a new line)
	\begin{subfigure}[b]{0.48\textwidth}
		\includegraphics[width=\textwidth]{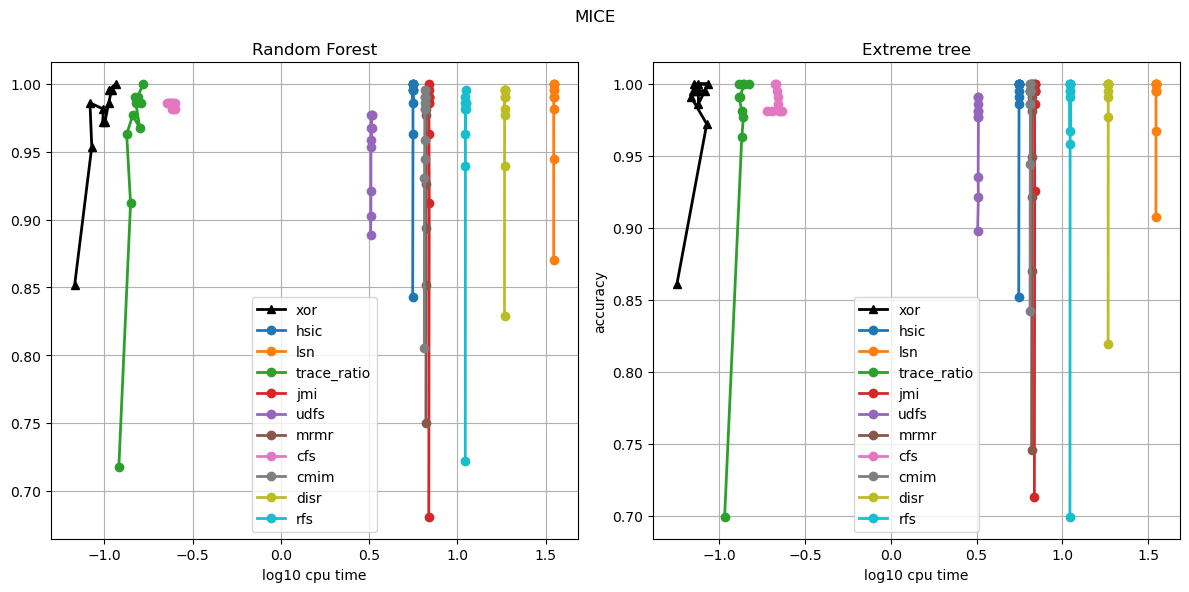}
		\caption{}
		
	\end{subfigure}
	\begin{subfigure}[b]{0.48\textwidth}
		\includegraphics[width=\textwidth]{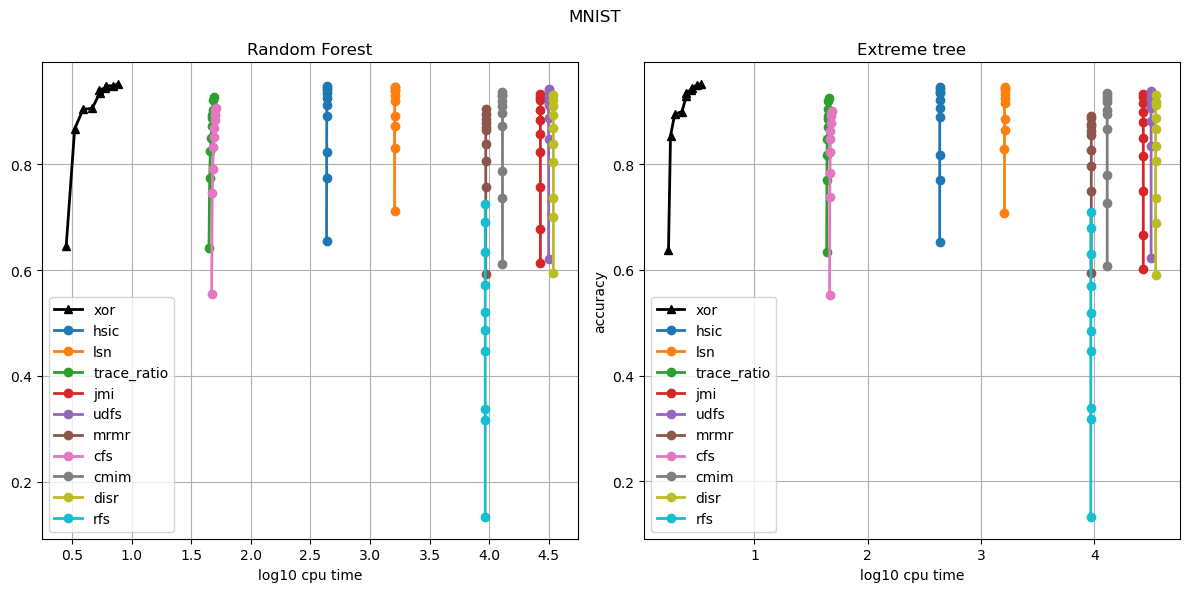}
		\caption{}
		
	\end{subfigure}
	\begin{subfigure}[b]{0.48\textwidth}
		\includegraphics[width=\textwidth]{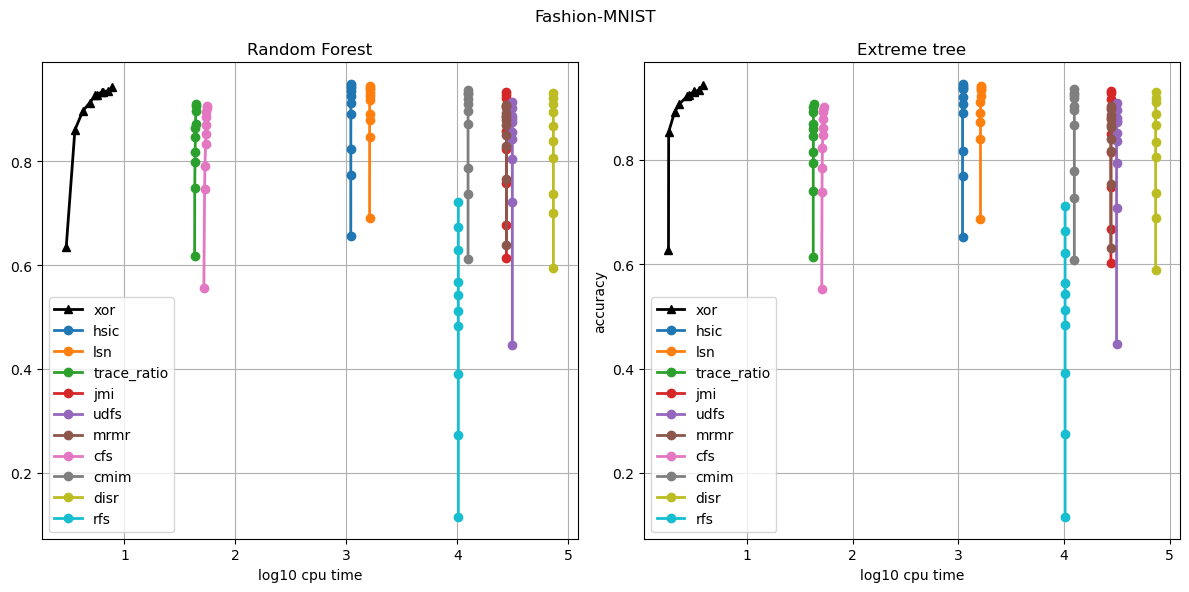}
		\caption{}
		
	\end{subfigure}
	
	\caption{The highest accuracy vs. time consuming when ExtreemTrees and RandomForest as classifier. }
	\label{the_highest_accuracy_time_xtreerf}
\end{figure}

\subsection{When Neural Network as the classifier}
We validate the effectiveness of features selected by our method on several datasets and different classifiers.
As Neural networks and Tree-based class classifiers are prevalent and differ in nature, to train and predict by Neural Networks could be useful to show that the features selected by our method are informative inherently.

\section{On the Stability}

\section{More about surrogate representation}
The key idea of our methods is that we can study the behavior of features through a lens of surrogate representation of each class in dataset.
At the core of it is the construction of surrogate representations, which summarize classes into a synthetic data point in the original feature space.
There are some typical idea to do so, such as barycenter, average of samples, average of normalized data, etc.
However, this is by no means a trivial thing, for the goal is to propose a feature selection method which is applicable to a wide range of datasets.

We conduct dozens of low-order moments based methods to find the most proper one empirically.

\begin{figure}[!h]
	\centering
	%\vspace{-2cm}
	%\hspace{-2cm}
	\begin{subfigure}[b]{0.48\textwidth}	%1
		\includegraphics[width=\textwidth]{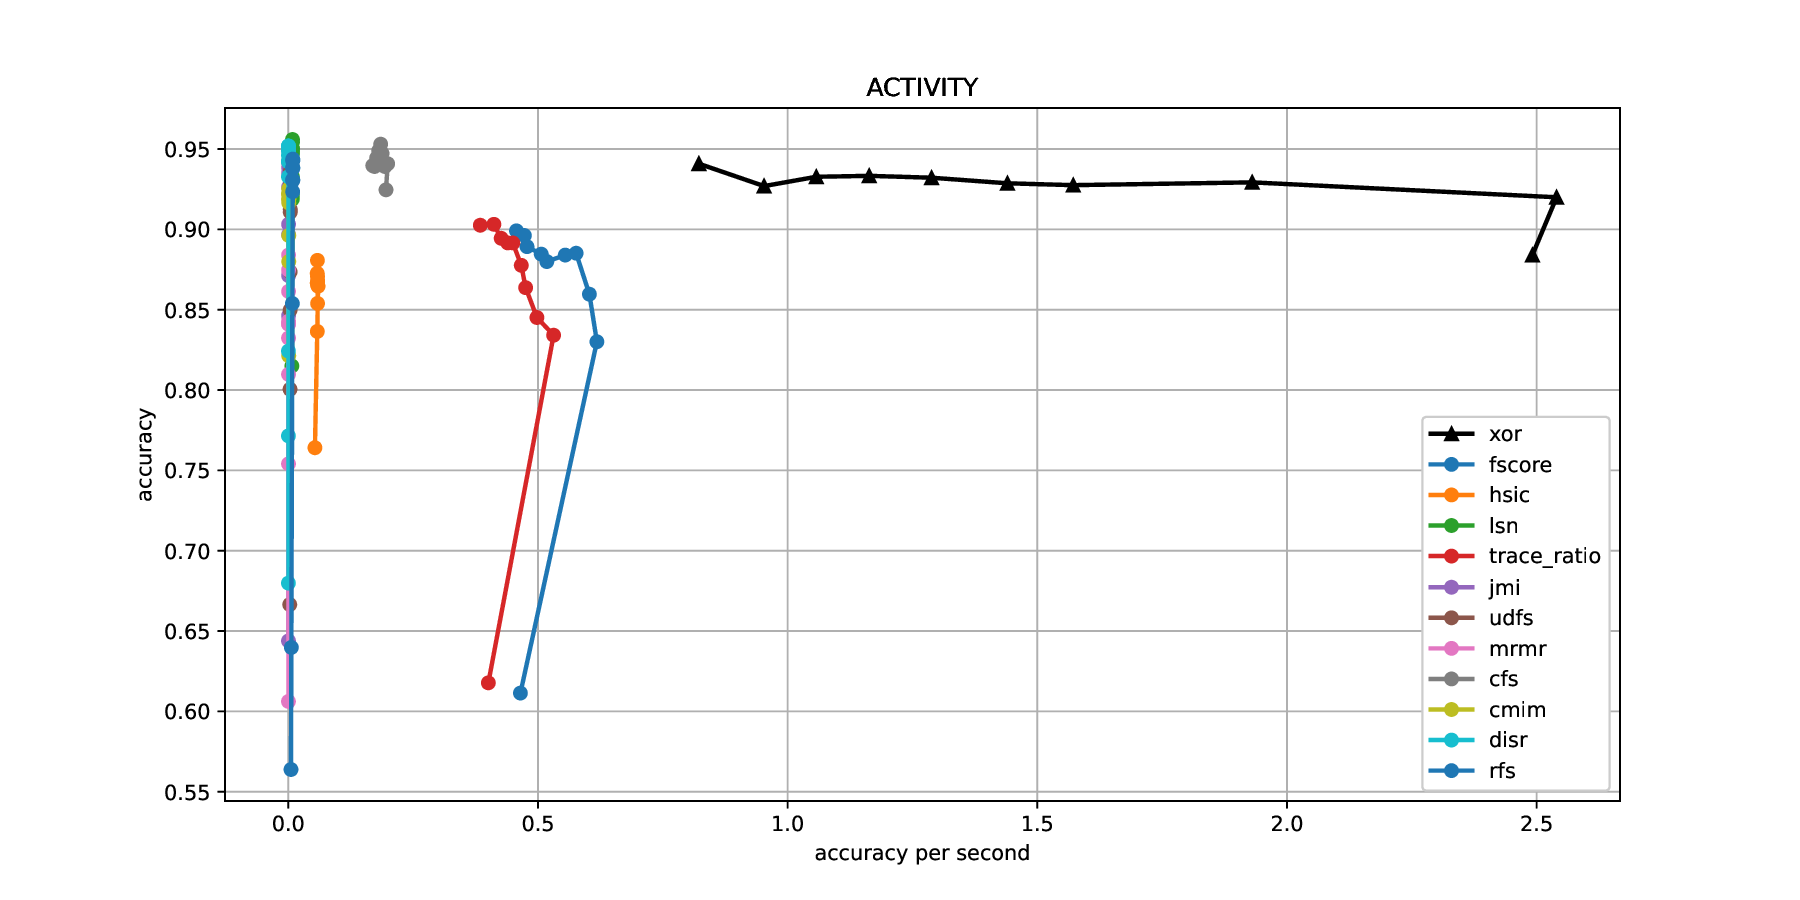} 
		\caption{}
	\end{subfigure}
	\begin{subfigure}[b]{0.48\textwidth}%2
		\includegraphics[width=\textwidth]{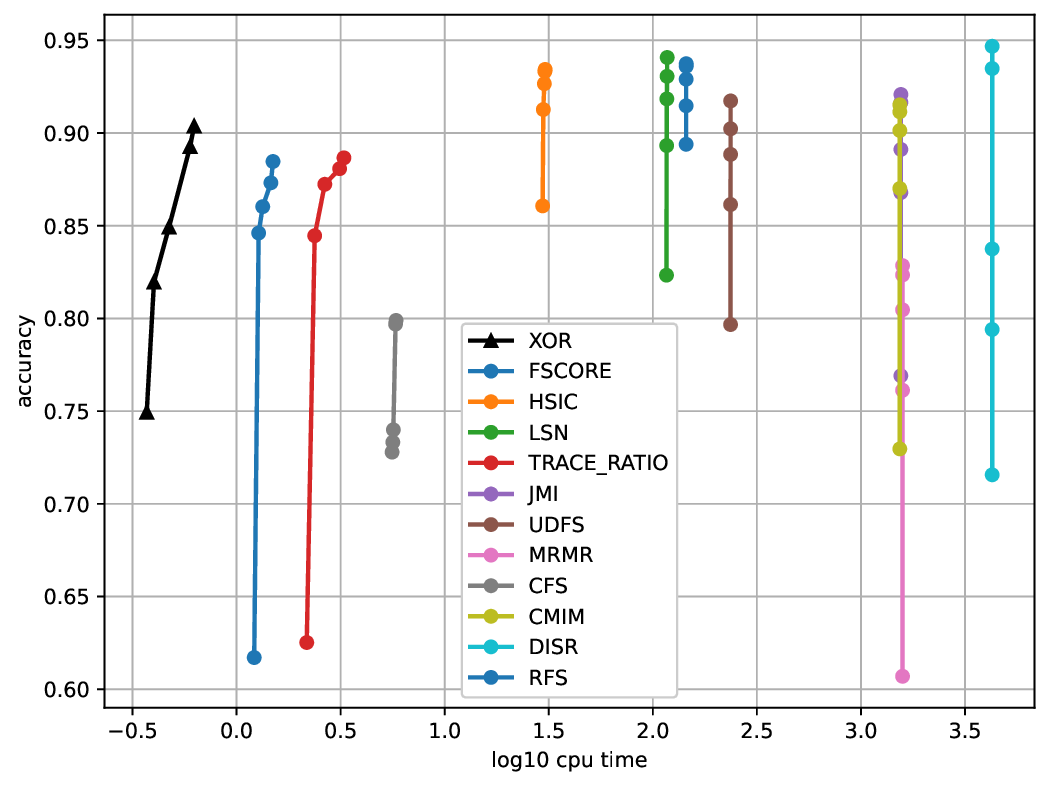}
		\caption{}
	\end{subfigure}

	\begin{subfigure}[b]{0.48\textwidth}	%3
	\includegraphics[width=\textwidth]{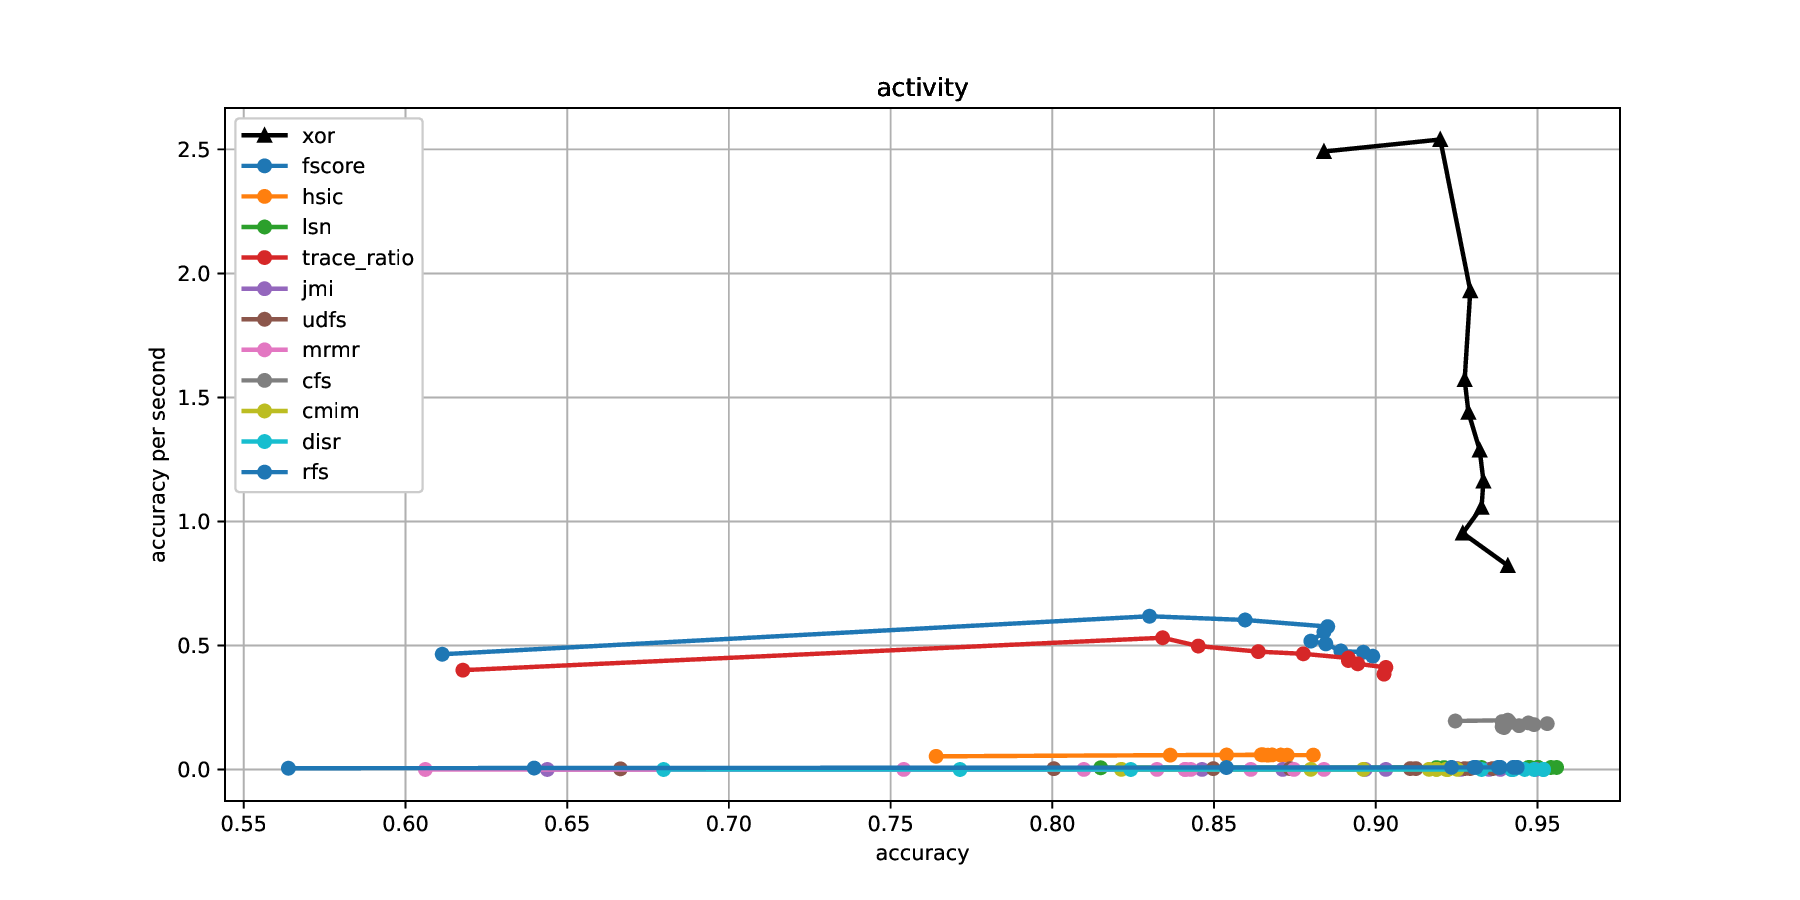}
	\caption{}
	\end{subfigure}
	\begin{subfigure}[b]{0.48\textwidth}	%4
		\includegraphics[width=\textwidth]{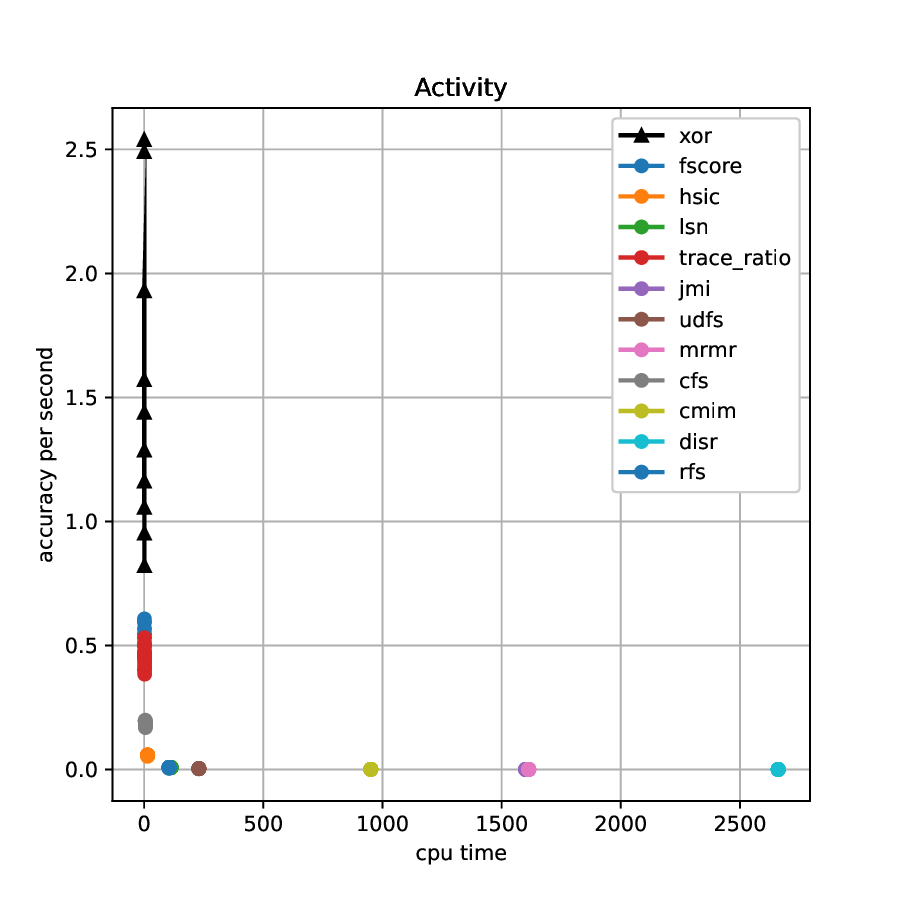}
		\caption{}
	\end{subfigure}

	\begin{subfigure}[b]{0.48\textwidth}%5
		\includegraphics[width=\textwidth]{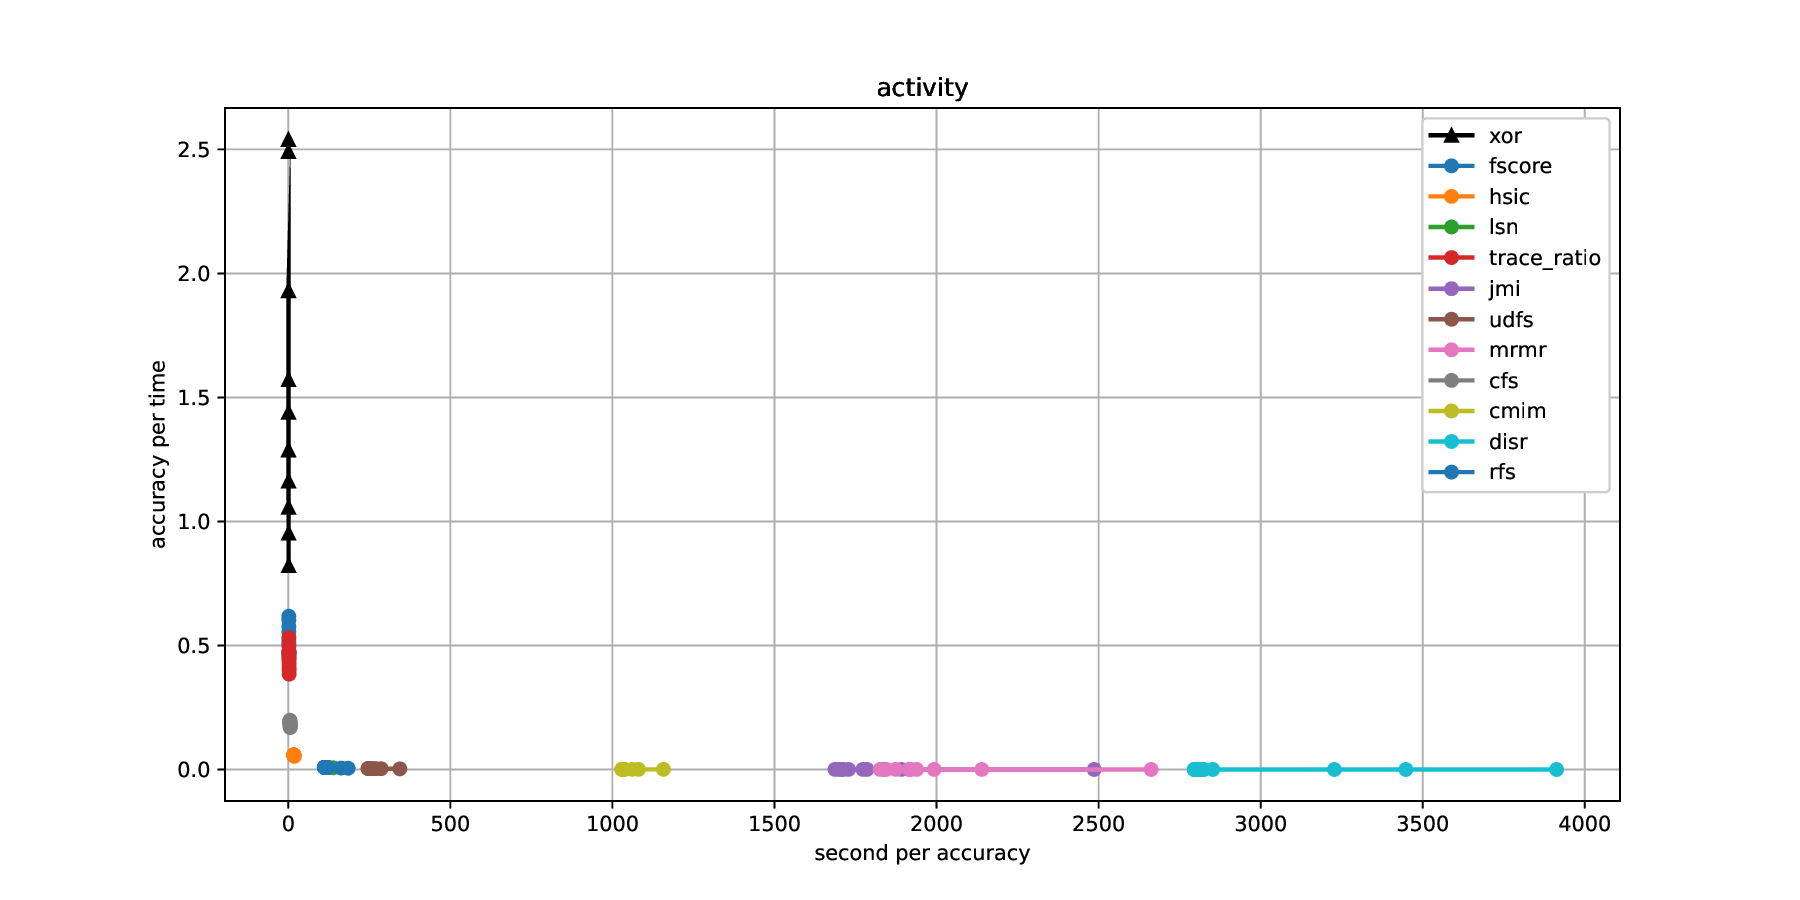}
		\caption{}
	\end{subfigure}
	\begin{subfigure}[b]{0.48\textwidth}	%6
		\includegraphics[width=\textwidth]{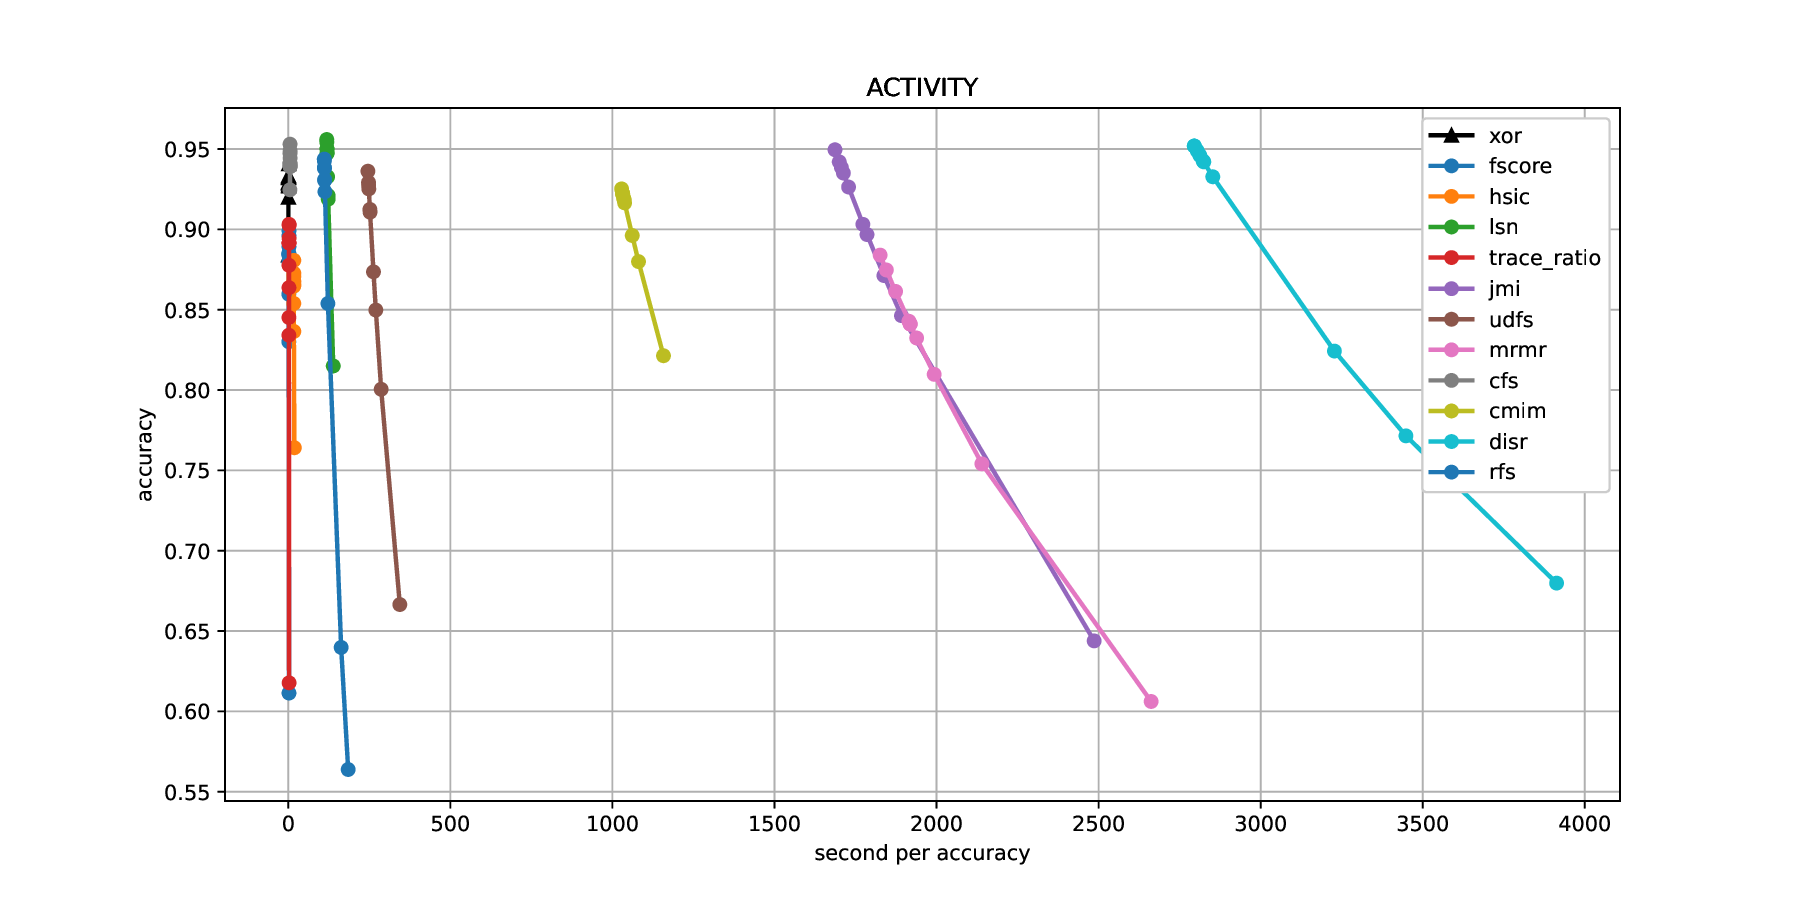}
		\caption{}	
	\end{subfigure}

	\begin{subfigure}[b]{0.48\textwidth}	%7
		\includegraphics[width=\textwidth]{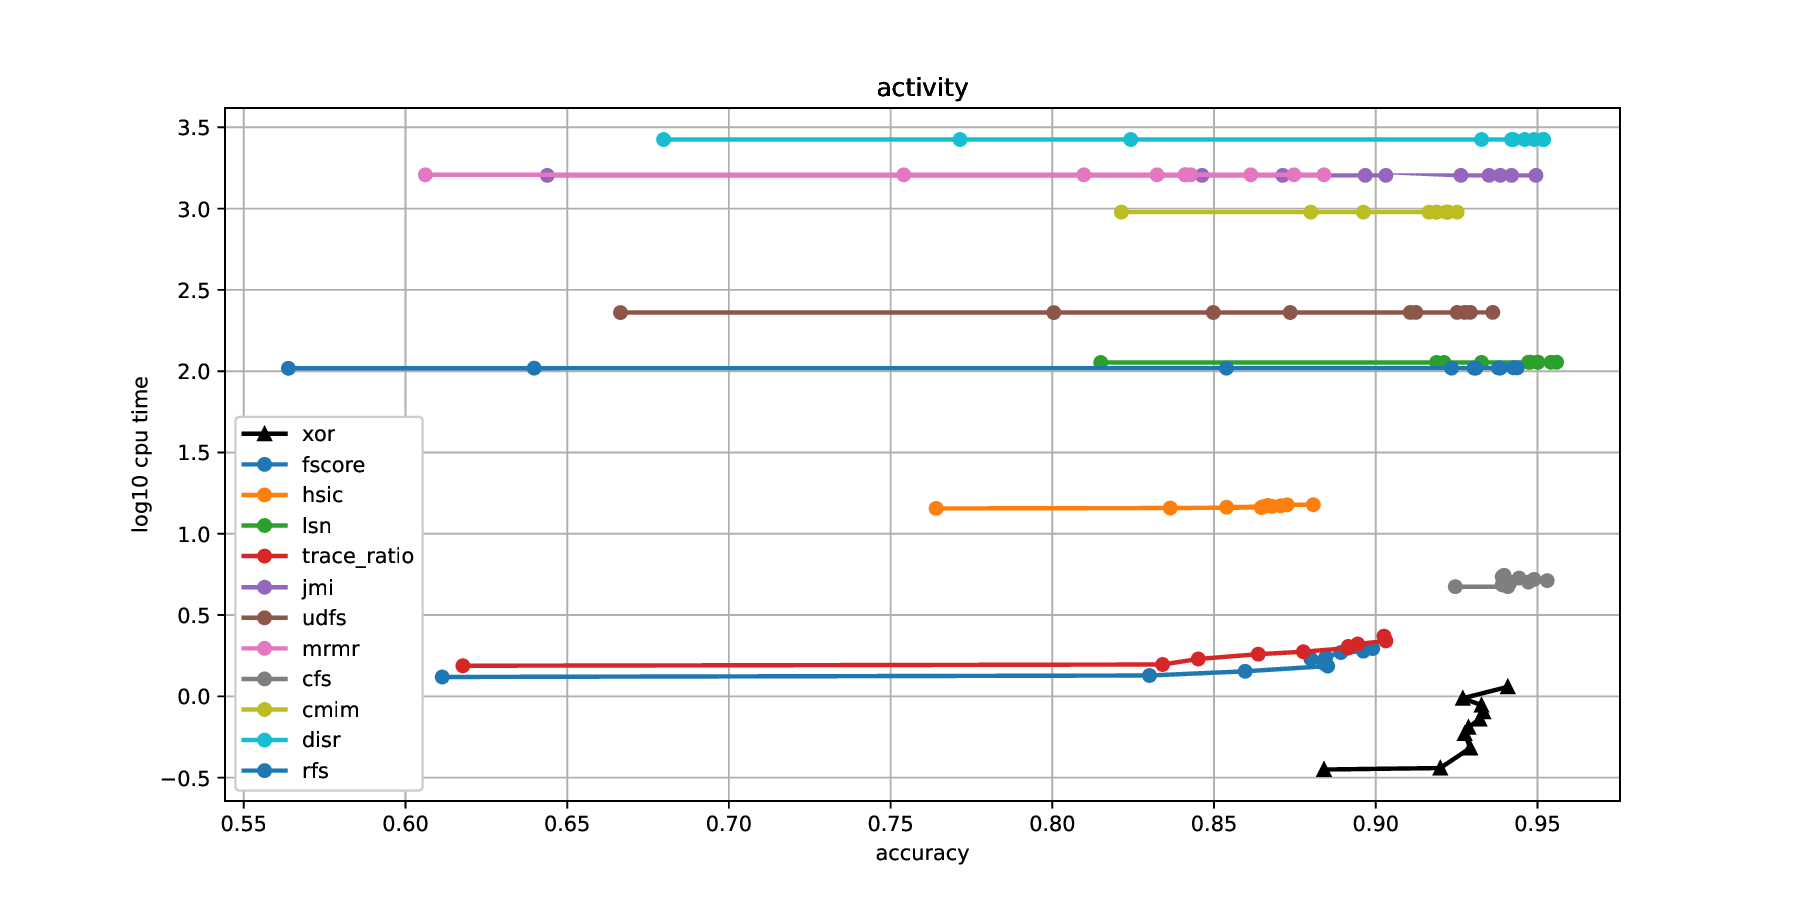}
		\caption{}
	\end{subfigure}
	\begin{subfigure}[b]{0.48\textwidth}	%8
		\includegraphics[width=\textwidth]{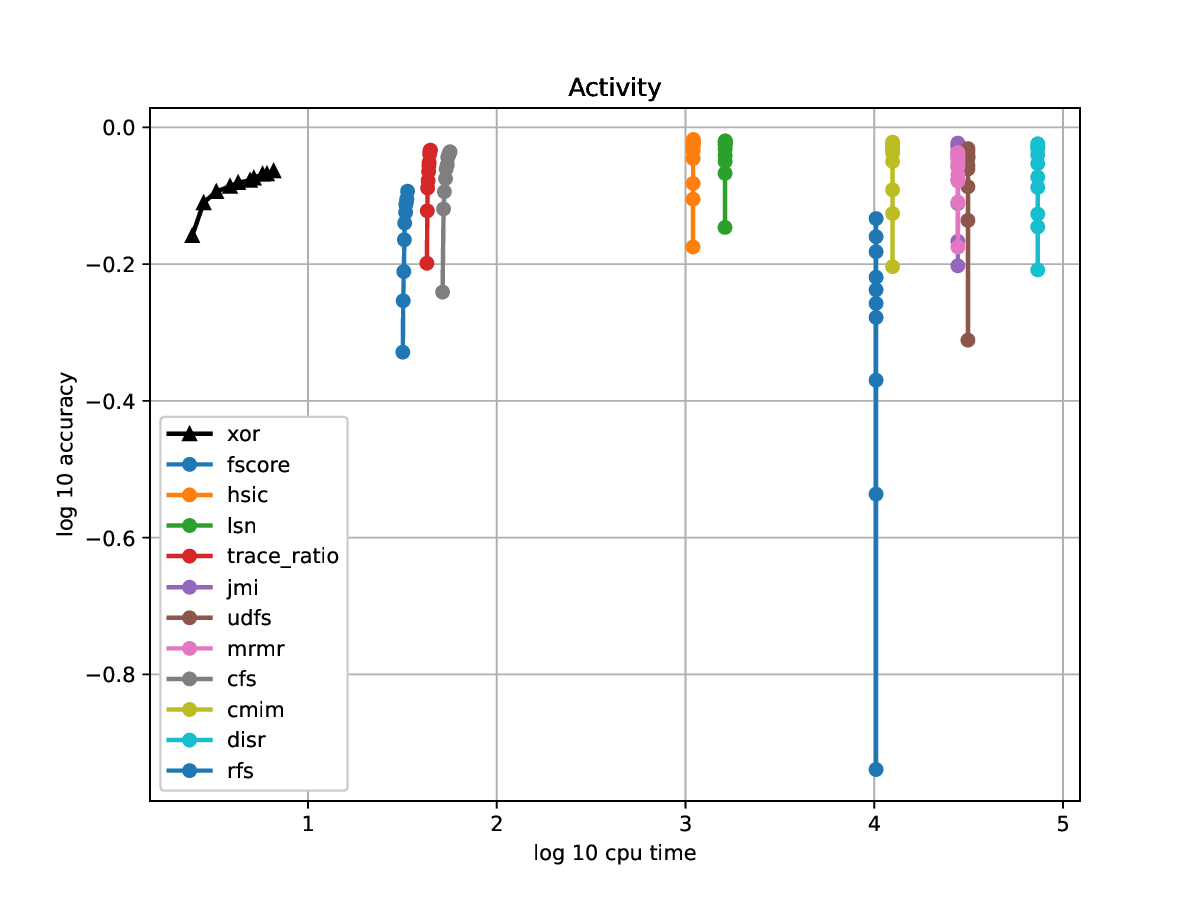}
		\caption{}
	\end{subfigure}
		
	\begin{subfigure}[b]{0.48\textwidth}	%9
		\includegraphics[width=\textwidth]{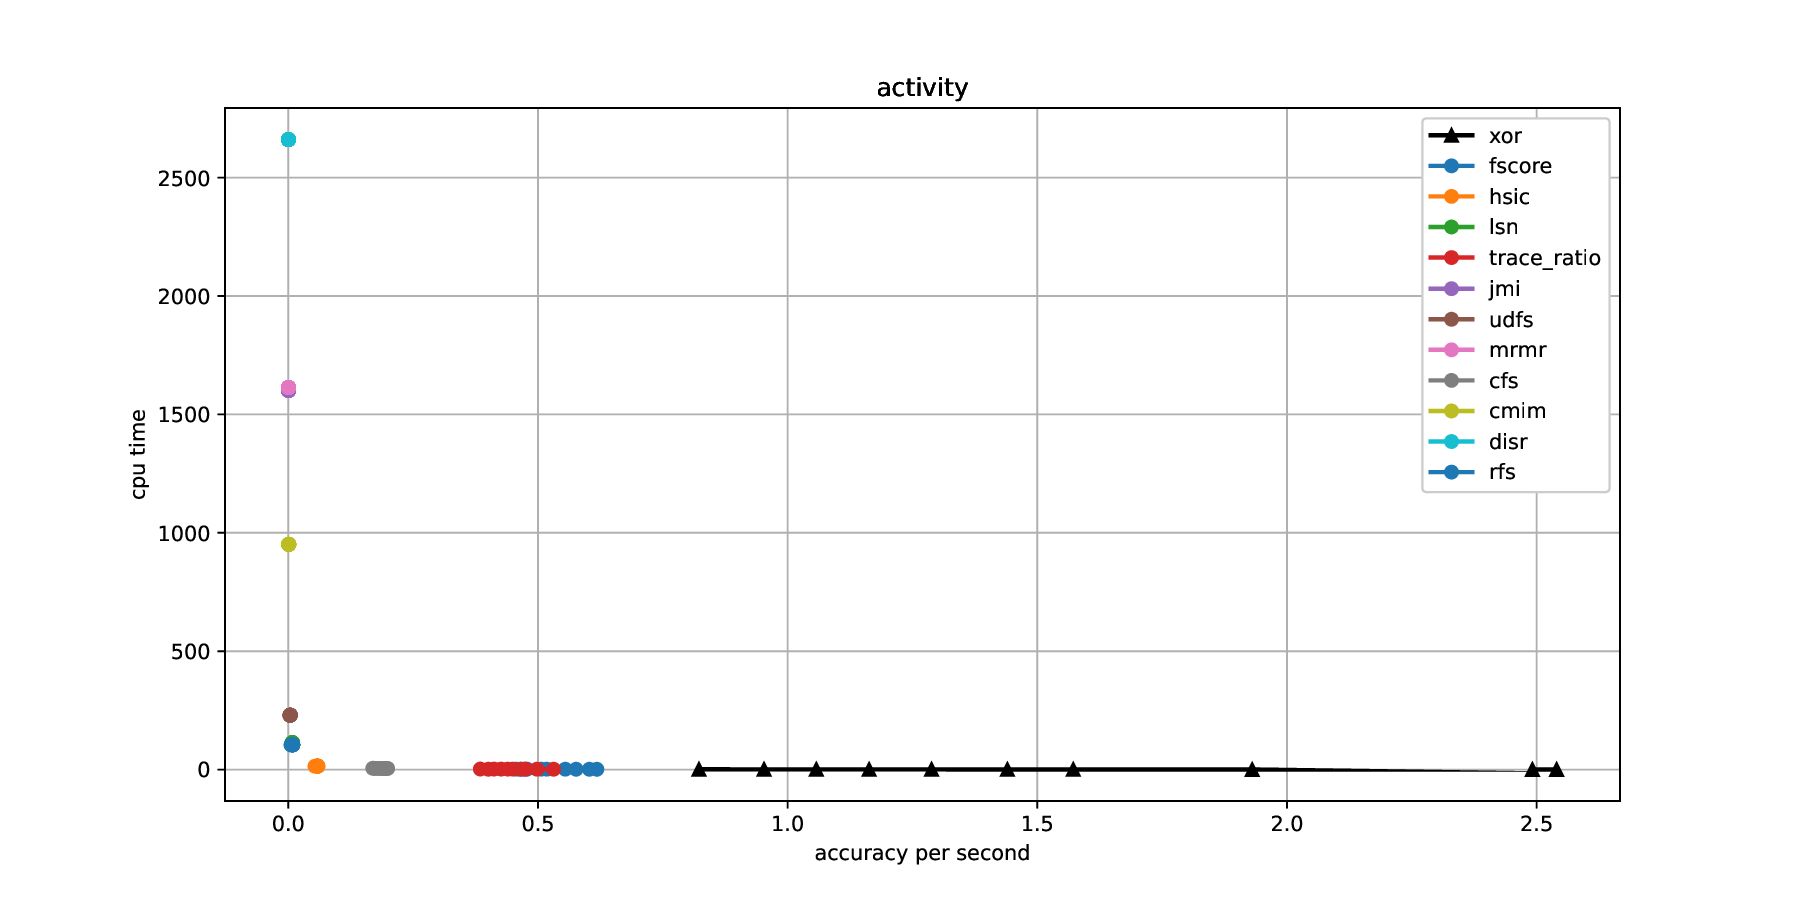}
		\caption{}
	\end{subfigure}
	\begin{subfigure}[b]{0.48\textwidth}	%10
		\includegraphics[width=\textwidth]{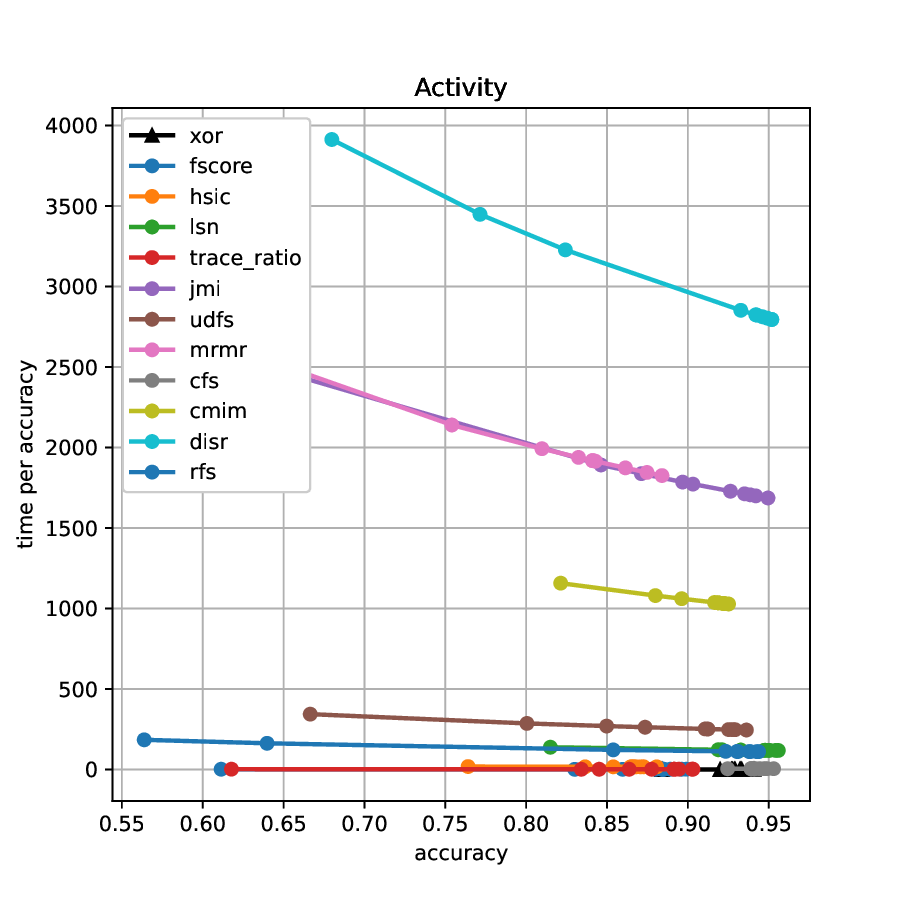}
		\caption{}
	\end{subfigure}

	\caption{Time consuming results on ACTIVITY dataset.}
	\label{time_consuming_comparison_activity}
\end{figure}

\begin{figure}[!h]
	\centering
	%\vspace{-2cm}
	%\hspace{-2cm}
	\begin{subfigure}[b]{0.48\textwidth}	%1
		\includegraphics[width=\textwidth]{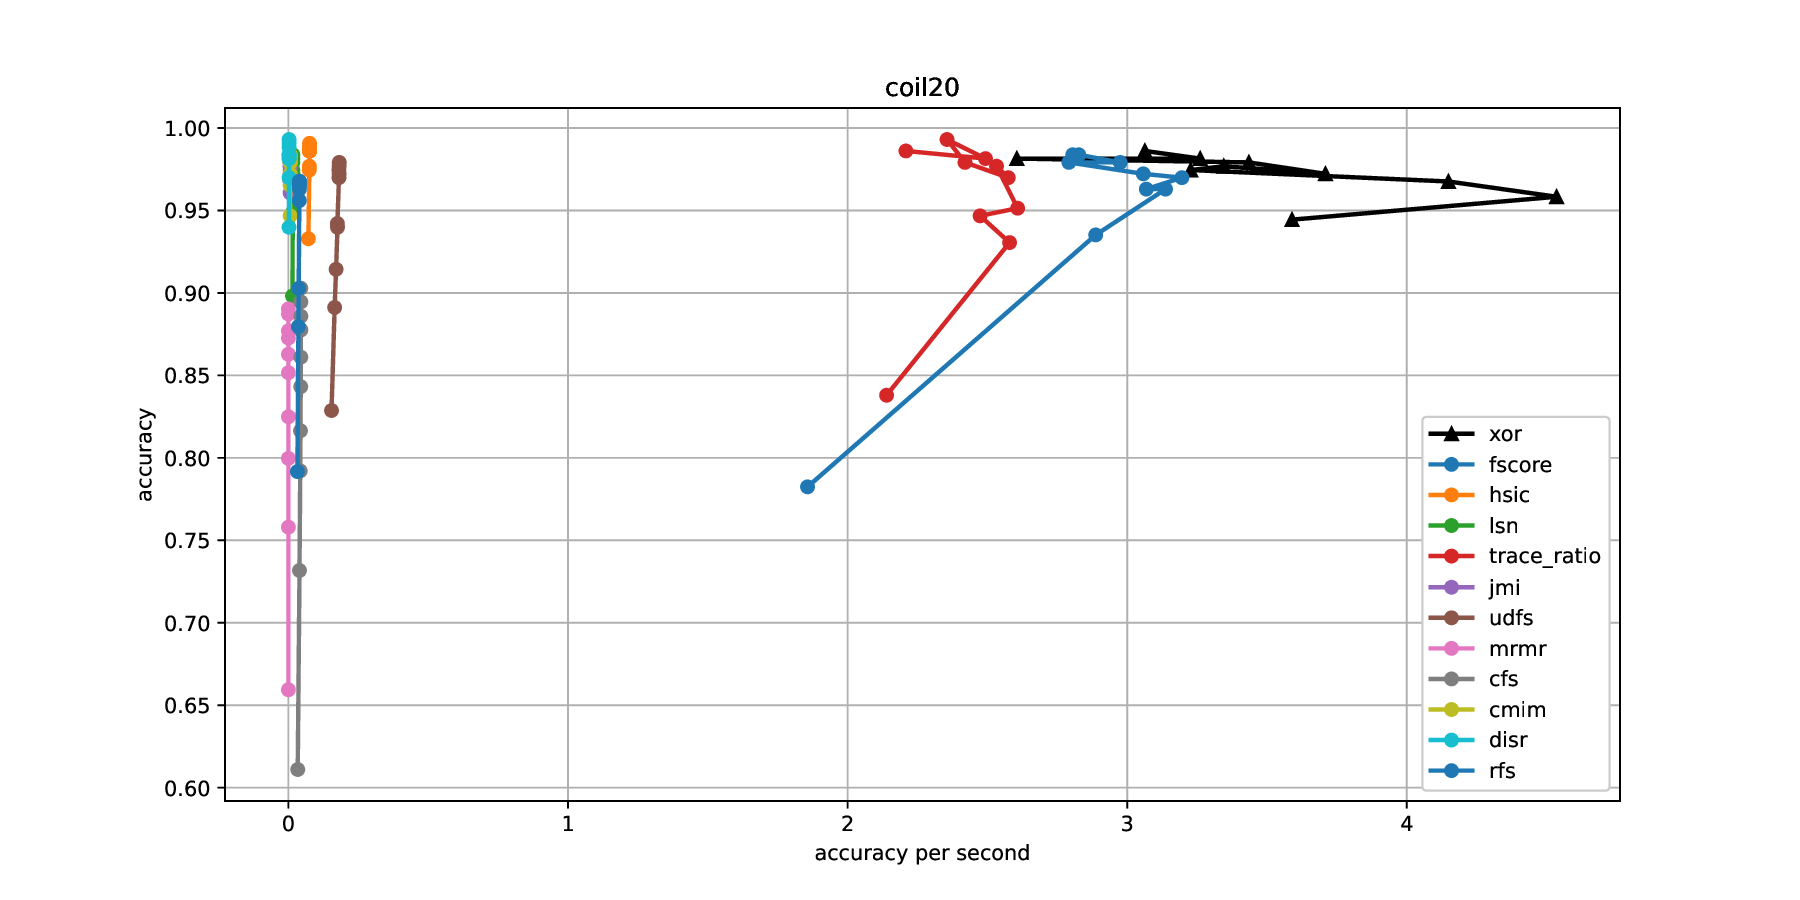} 
		\caption{}
	\end{subfigure}
	\begin{subfigure}[b]{0.48\textwidth}%2
		\includegraphics[width=\textwidth]{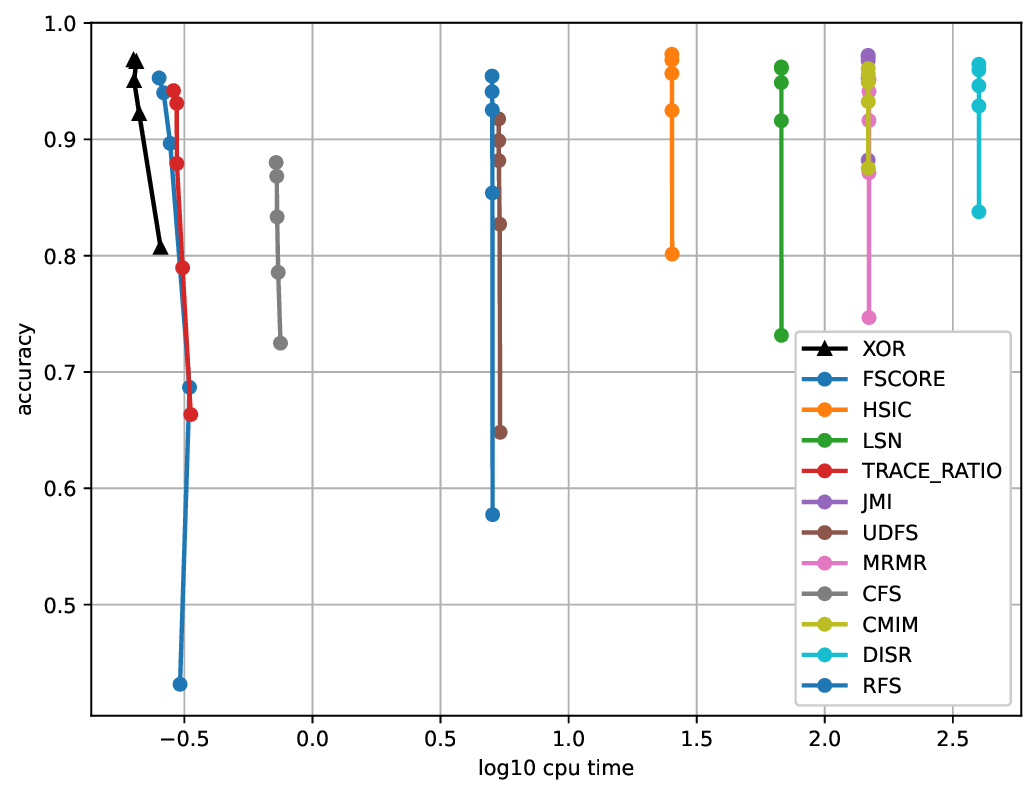}
		\caption{}
	\end{subfigure}
	
	\begin{subfigure}[b]{0.48\textwidth}	%3
		\includegraphics[width=\textwidth]{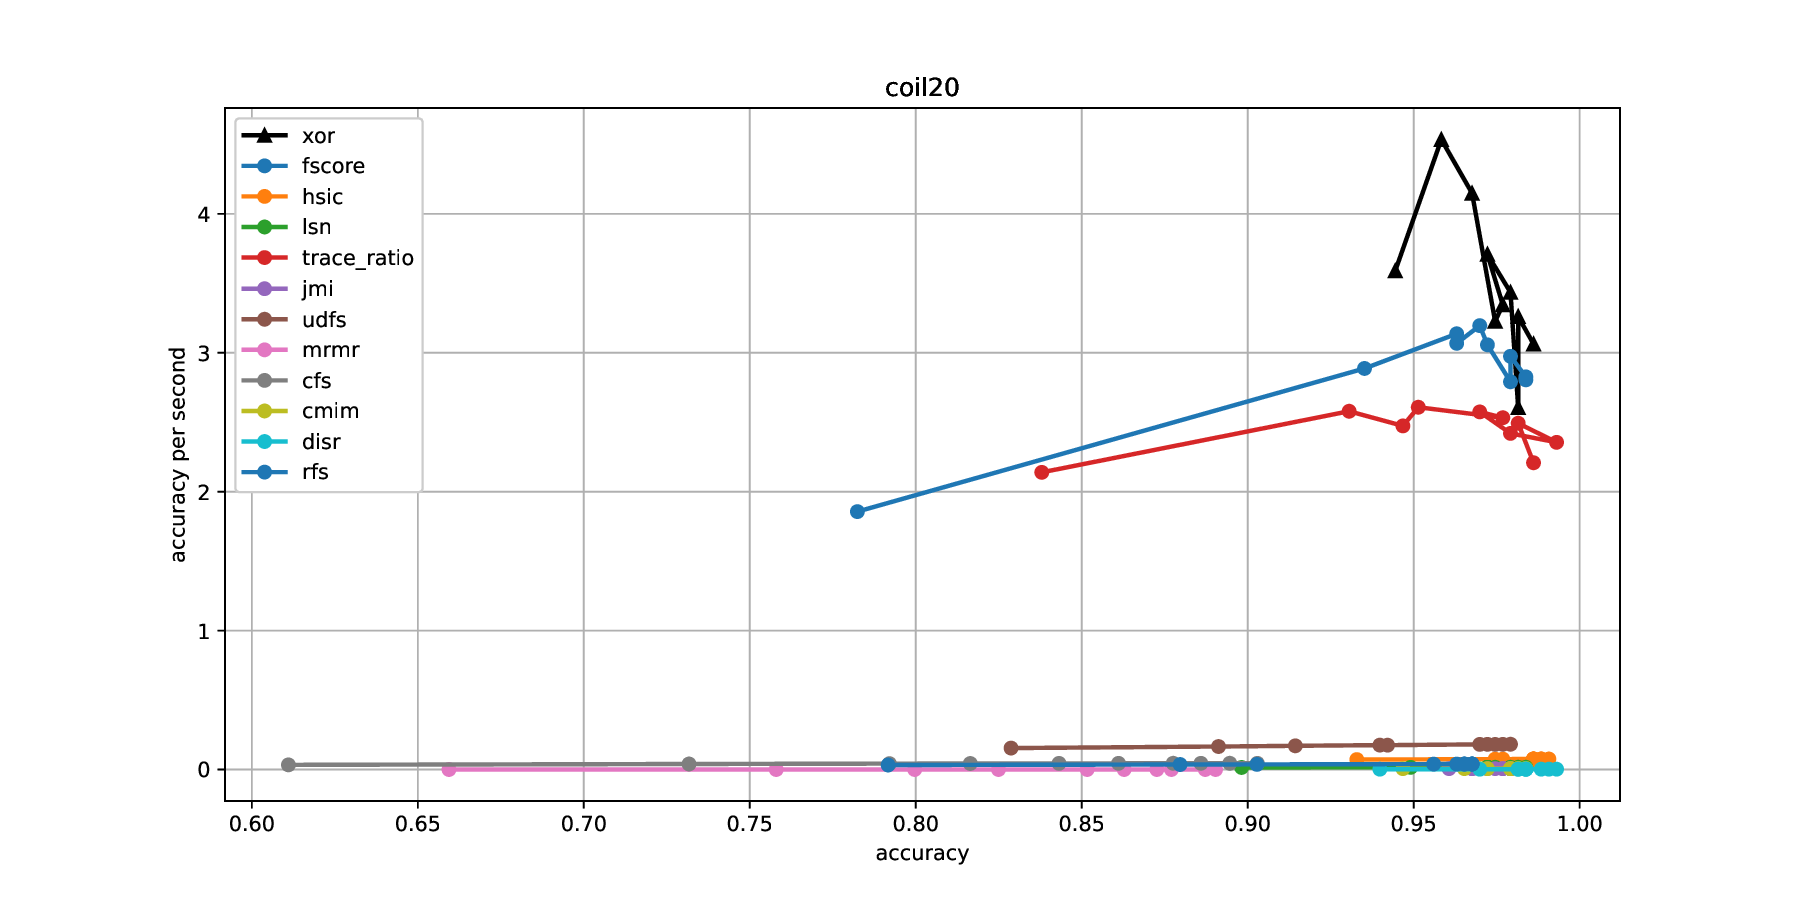}
		\caption{}
	\end{subfigure}
	\begin{subfigure}[b]{0.48\textwidth}	%4
		\includegraphics[width=\textwidth]{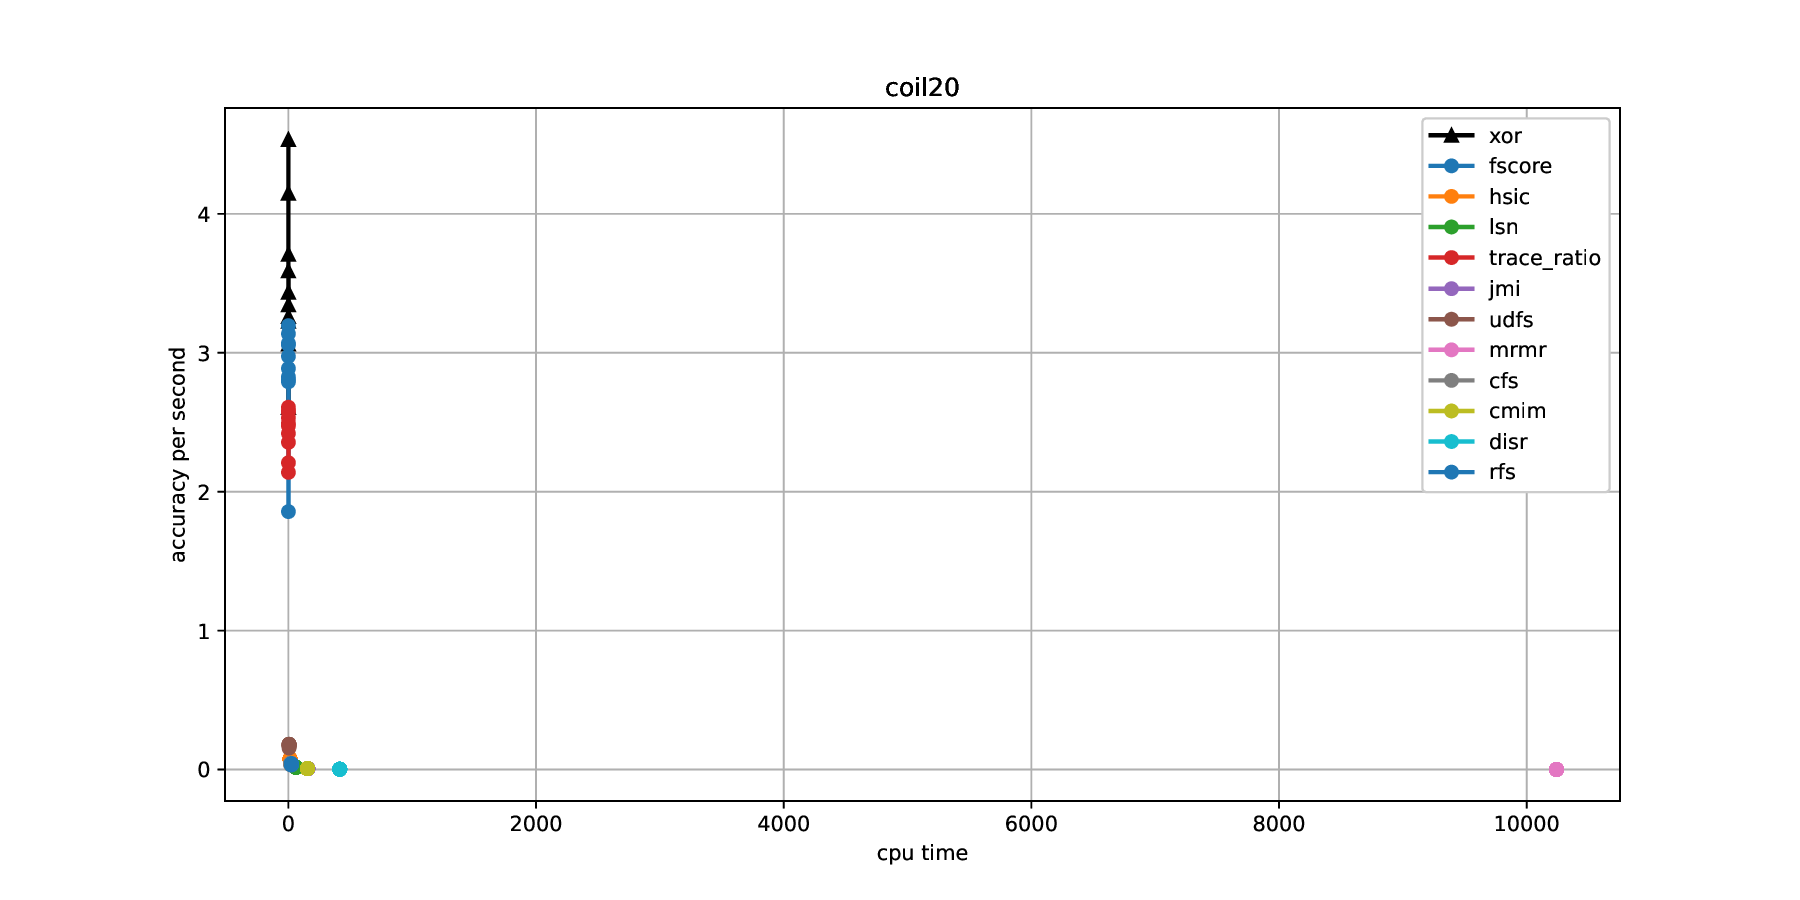}
		\caption{}
	\end{subfigure}
	
	\begin{subfigure}[b]{0.48\textwidth}%5
		\includegraphics[width=\textwidth]{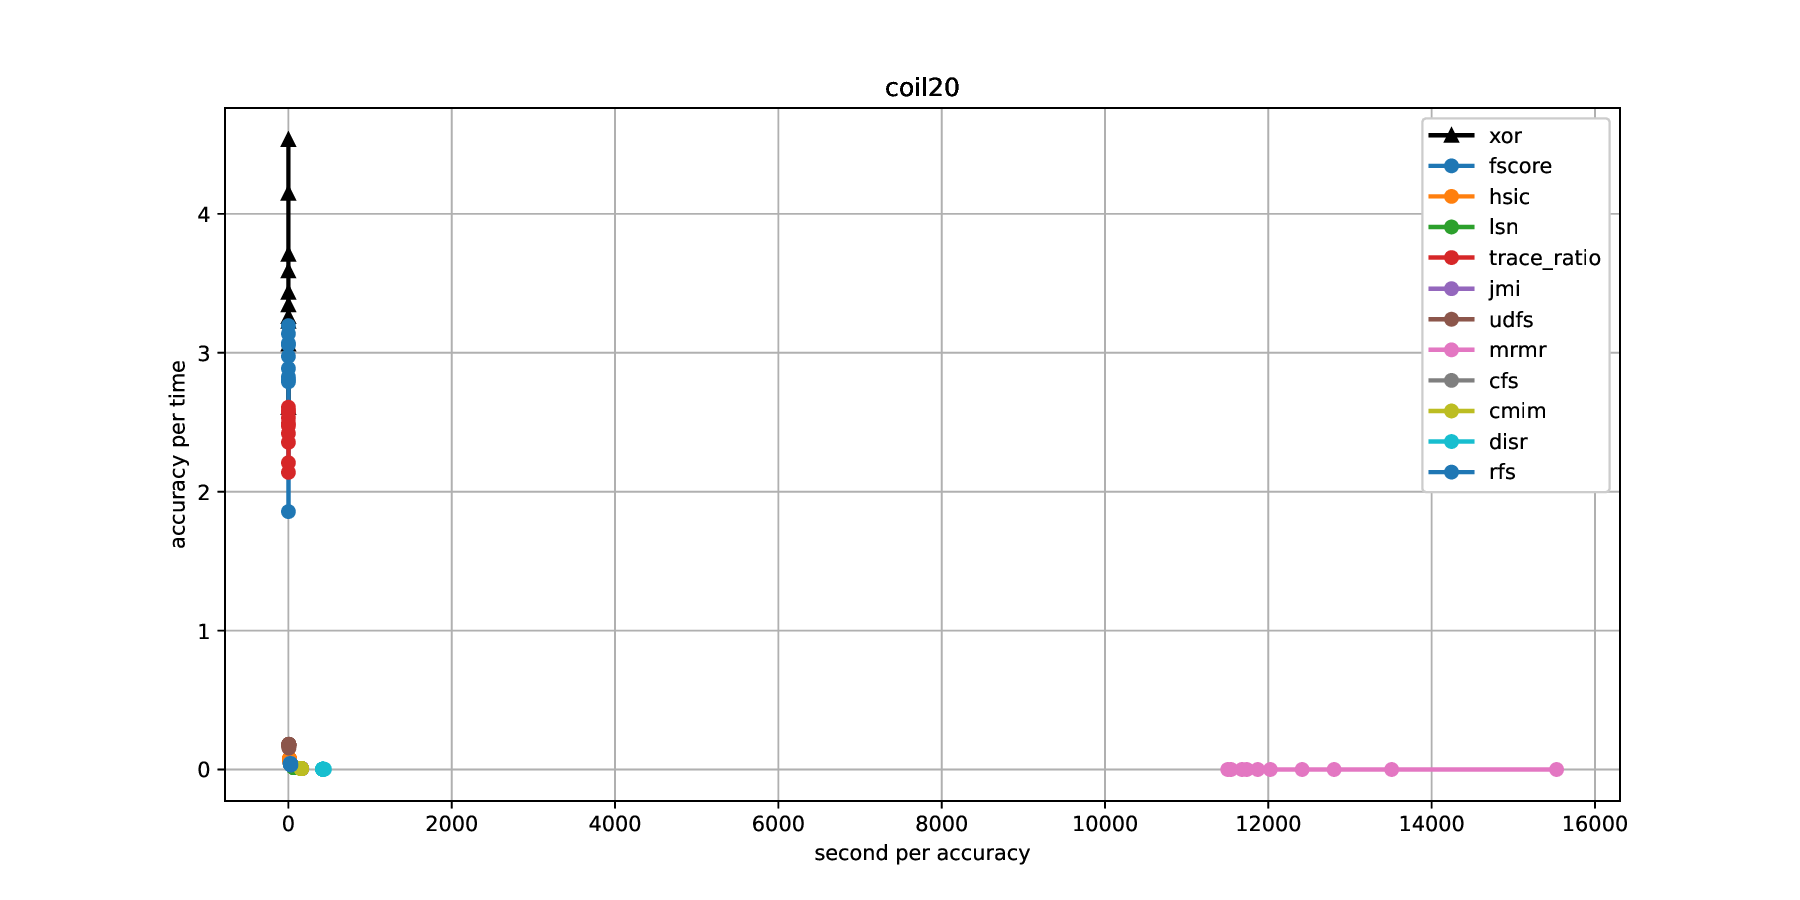}
		\caption{}
	\end{subfigure}
	\begin{subfigure}[b]{0.48\textwidth}	%6
		\includegraphics[width=\textwidth]{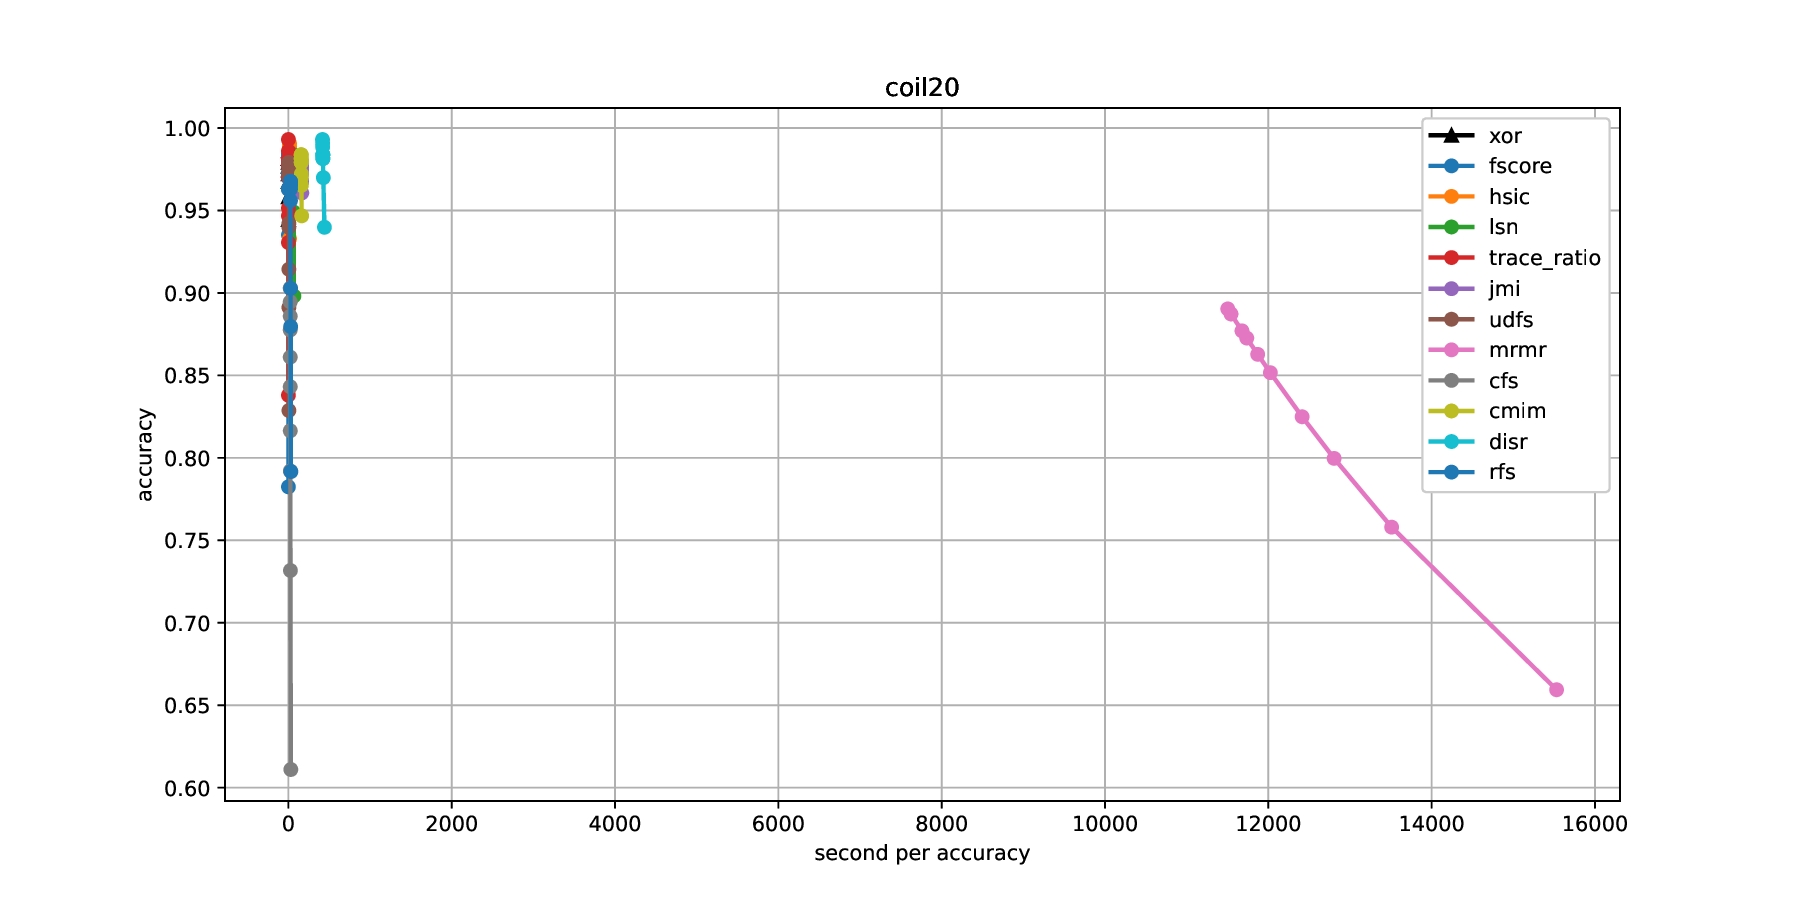}
		\caption{}	
	\end{subfigure}
	
	\begin{subfigure}[b]{0.48\textwidth}	%7
		\includegraphics[width=\textwidth]{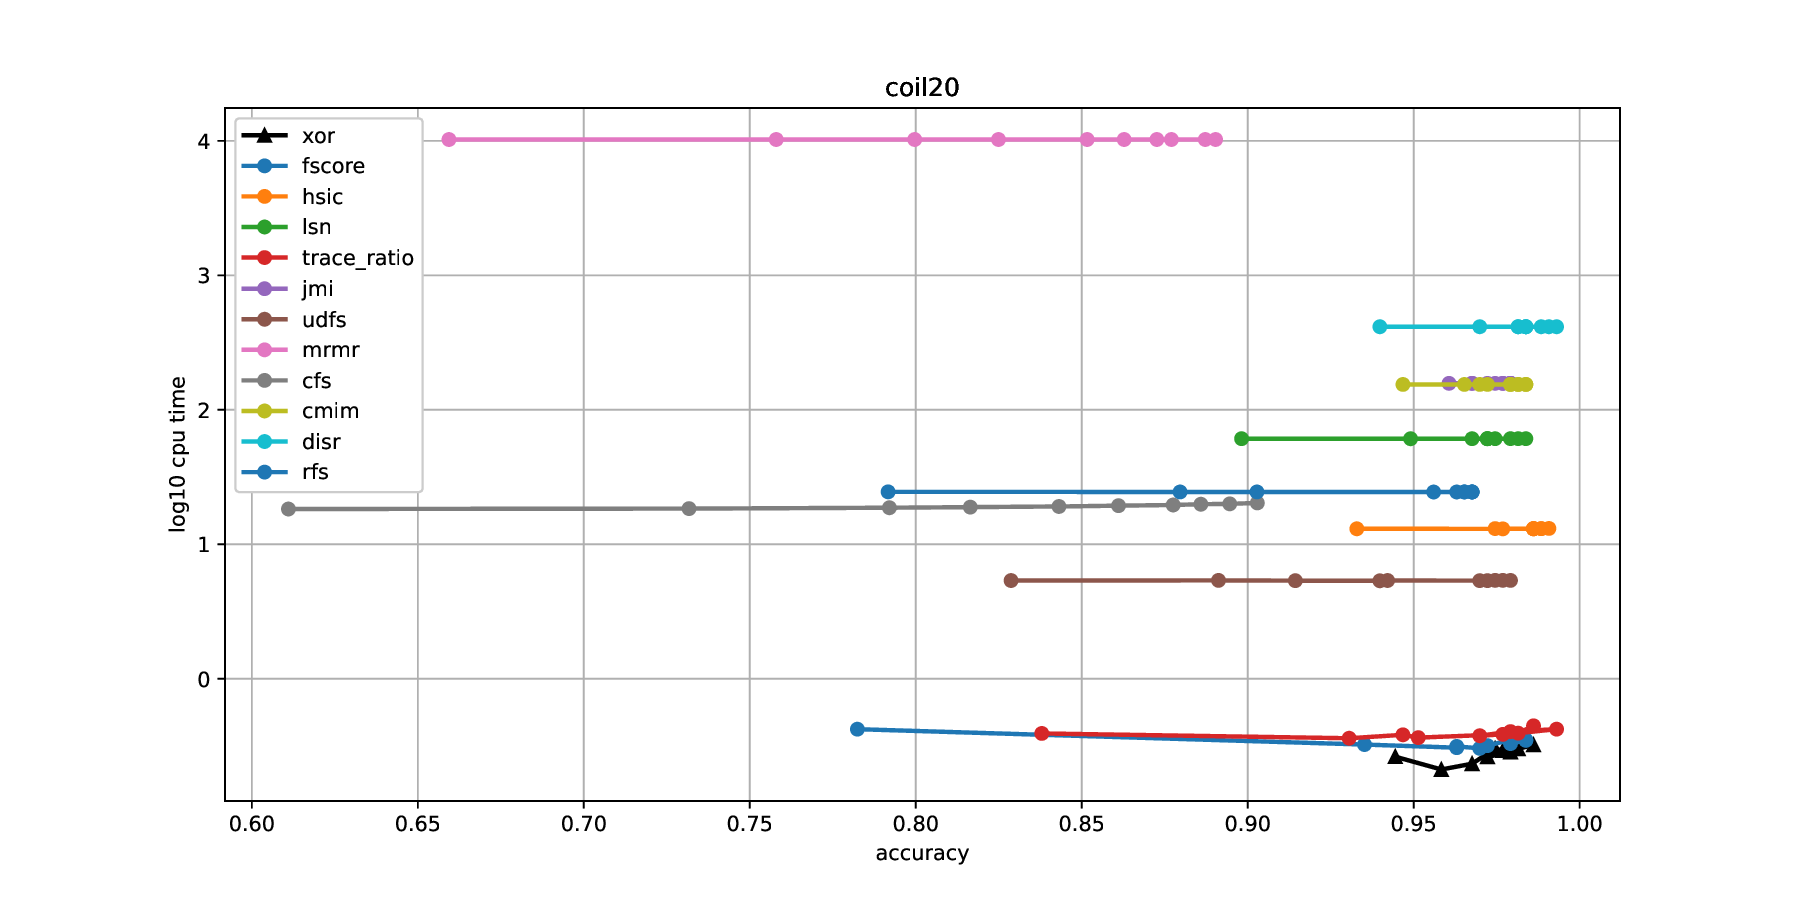}
		\caption{}
	\end{subfigure}
	\begin{subfigure}[b]{0.48\textwidth}	%8
		\includegraphics[width=\textwidth]{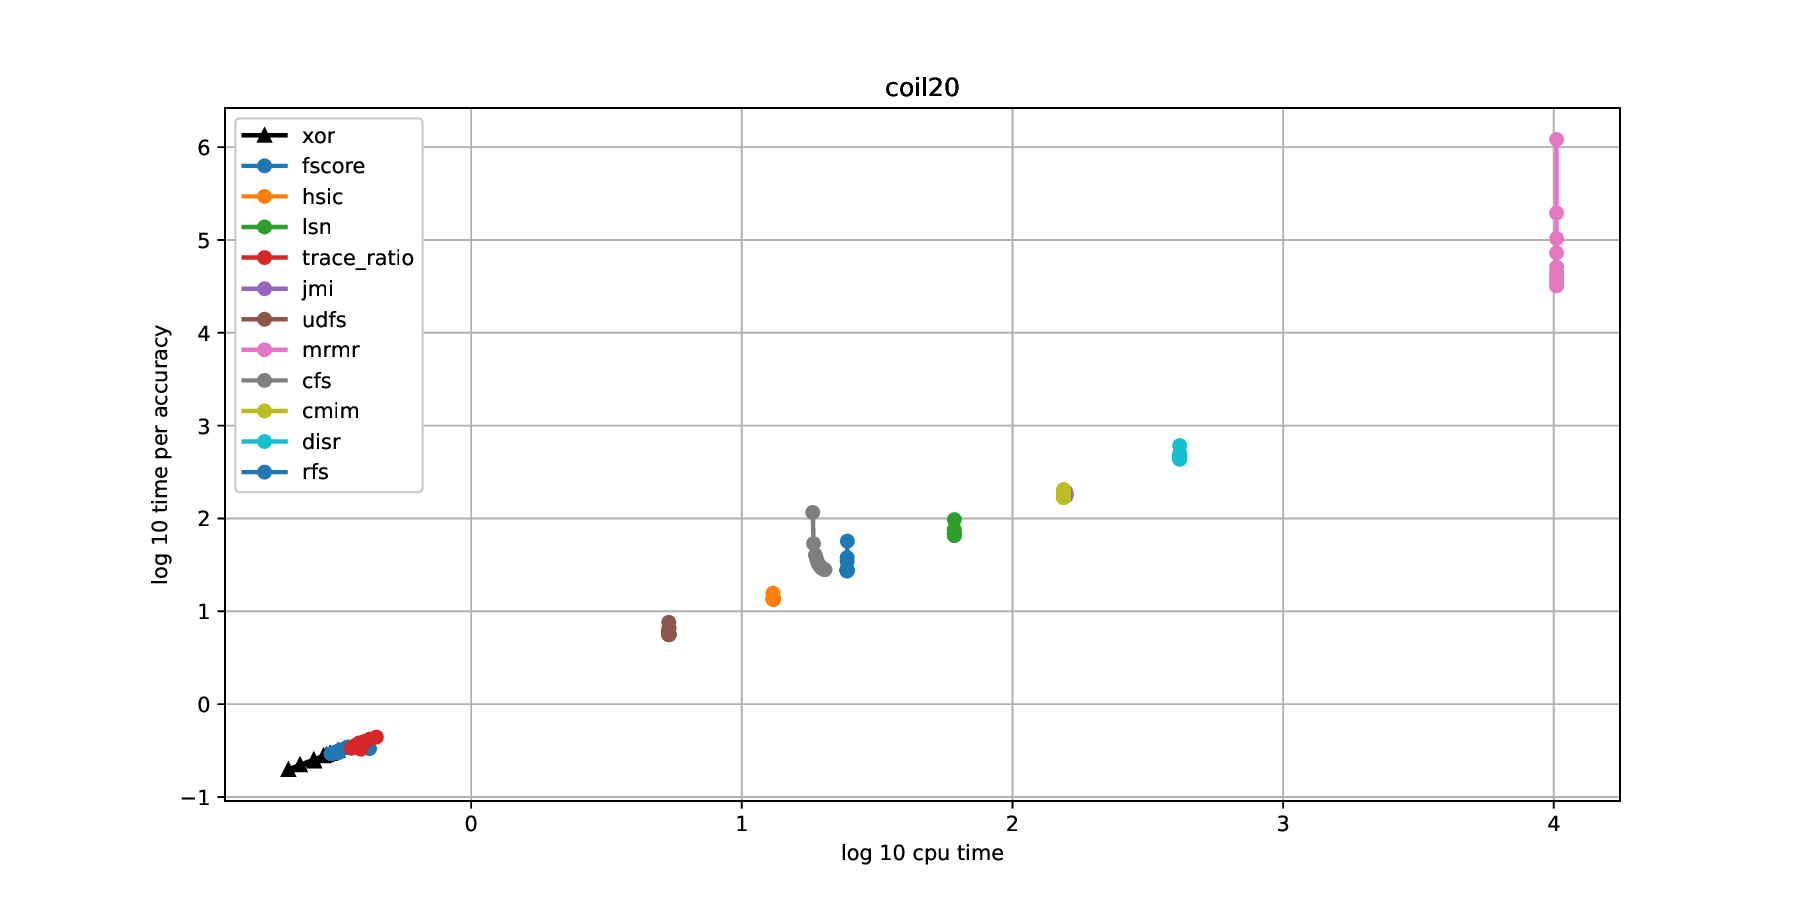}
		\caption{}
	\end{subfigure}
	
	\begin{subfigure}[b]{0.48\textwidth}	%9
		\includegraphics[width=\textwidth]{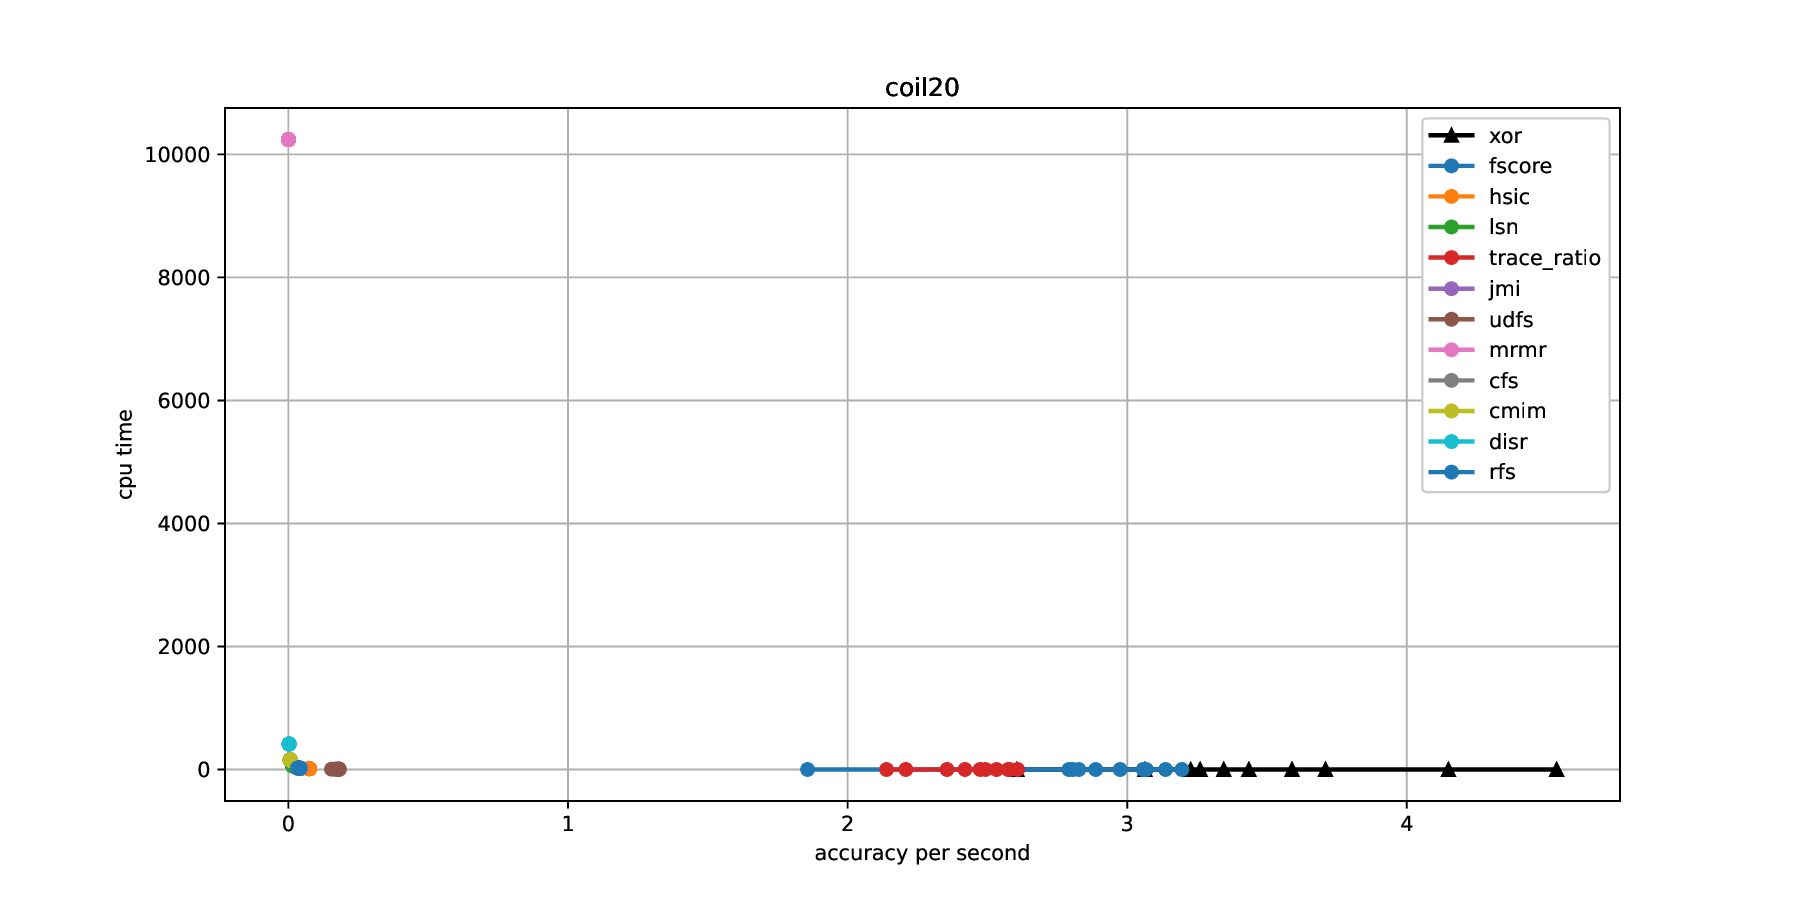}
		\caption{}
	\end{subfigure}
	\begin{subfigure}[b]{0.48\textwidth}	%10
		\includegraphics[width=\textwidth]{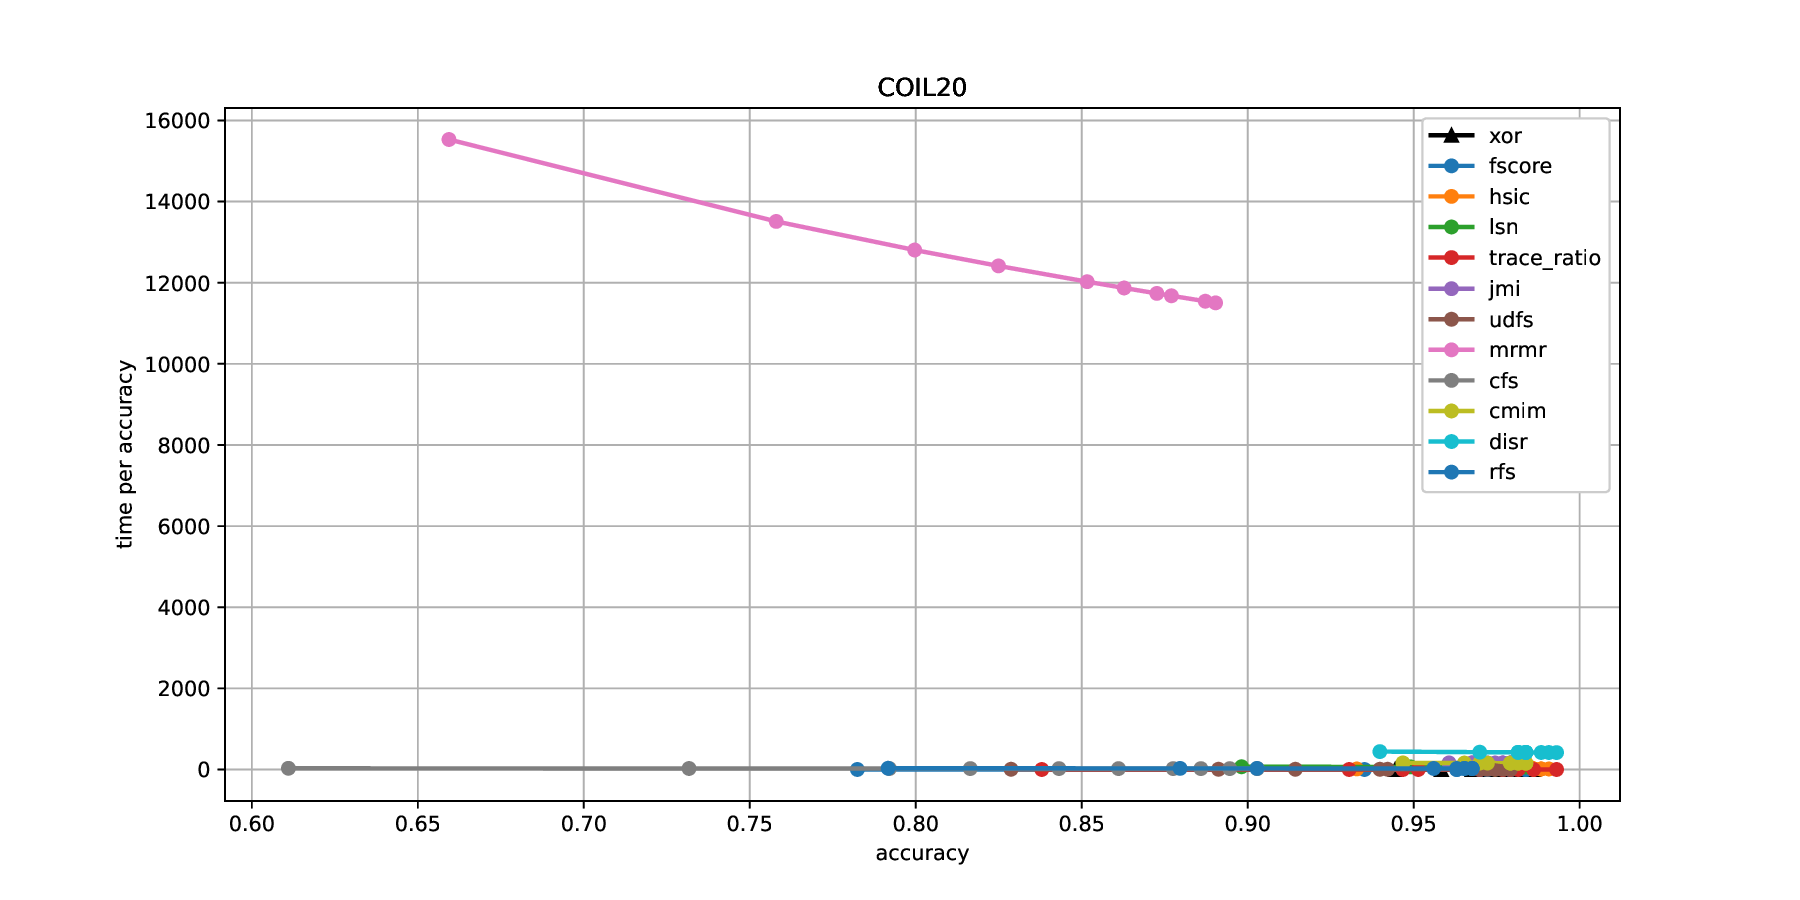}
		\caption{}
	\end{subfigure}
	
	\caption{Time consuming results on COIL-20 dataset.}
	\label{time_consuming_comparison_coil20}
\end{figure}

\begin{figure}[!h]
	\centering
	%\vspace{-2cm}
	%\hspace{-2cm}
	\begin{subfigure}[b]{0.48\textwidth}	%1
		\includegraphics[width=\textwidth]{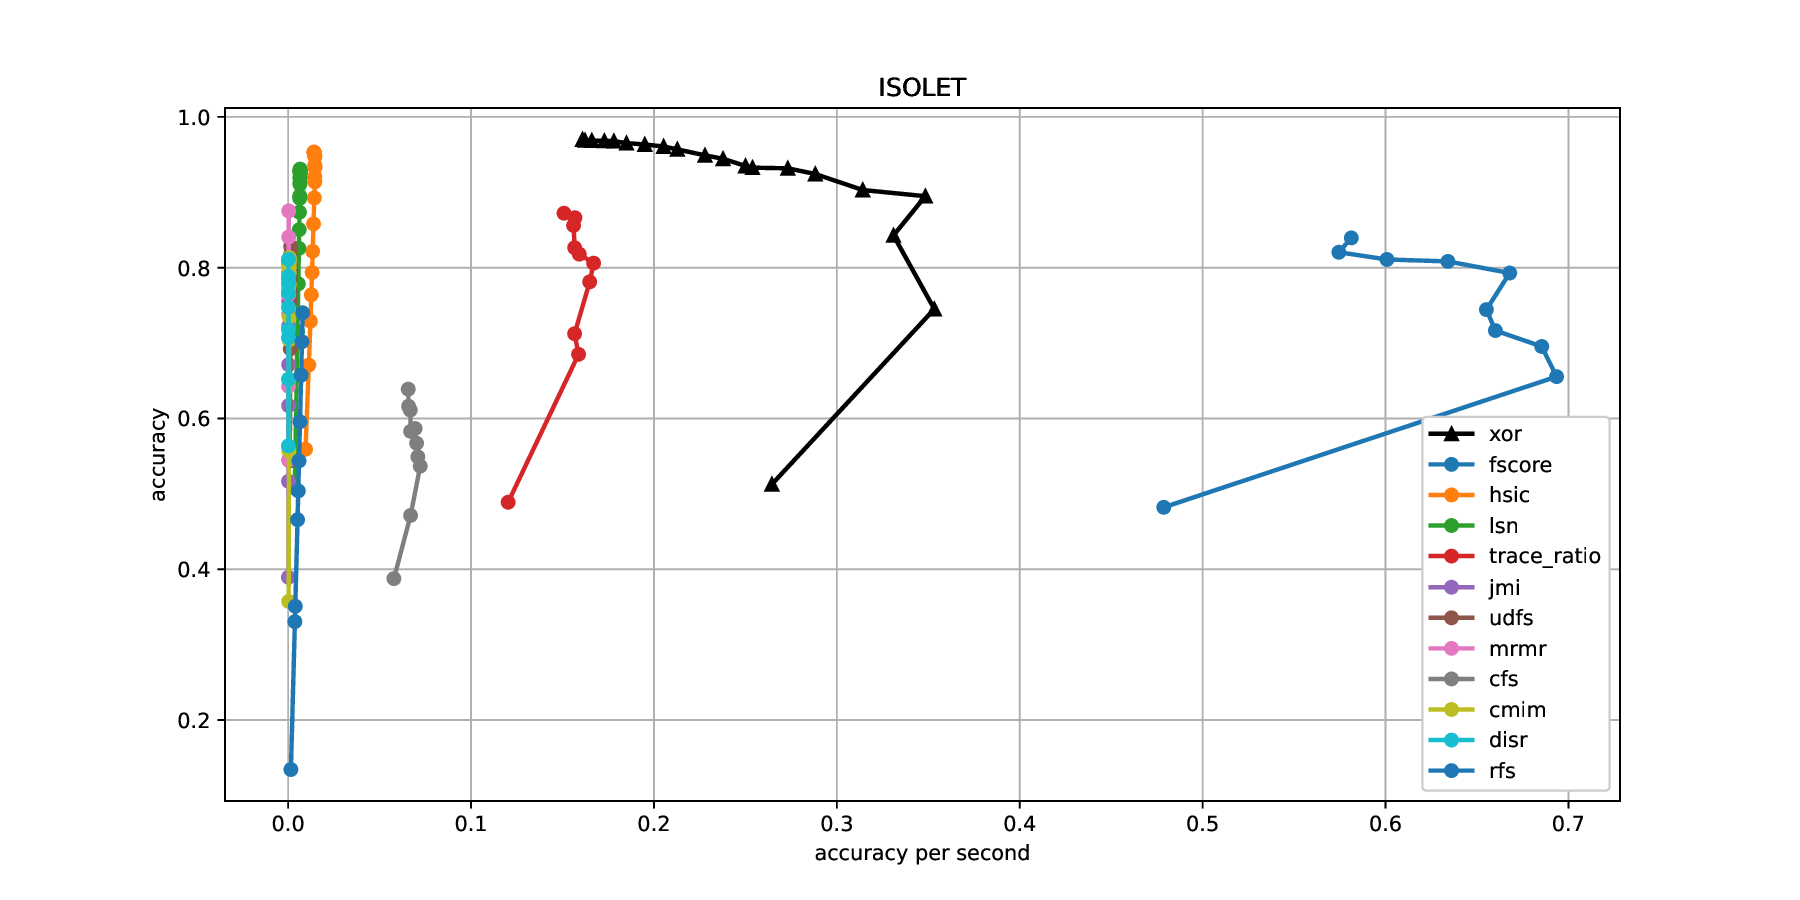} 
		\caption{}
	\end{subfigure}
	\begin{subfigure}[b]{0.48\textwidth}%2
		\includegraphics[width=\textwidth]{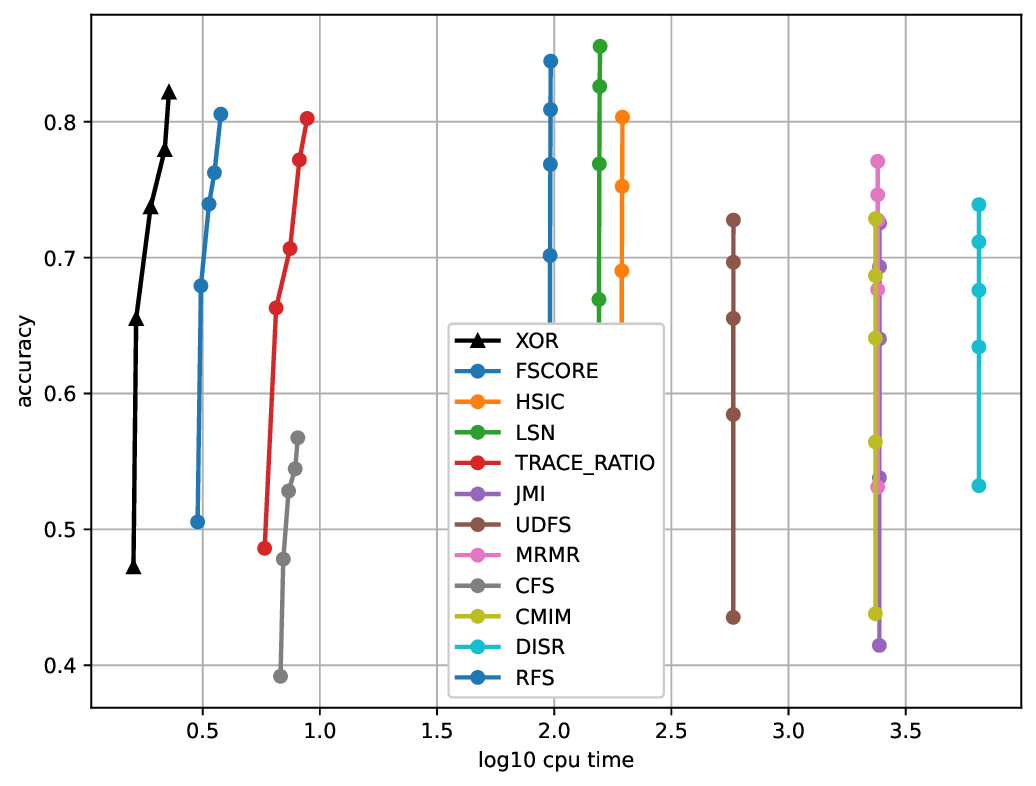}
		\caption{}
	\end{subfigure}
	
	\begin{subfigure}[b]{0.48\textwidth}	%3
		\includegraphics[width=\textwidth]{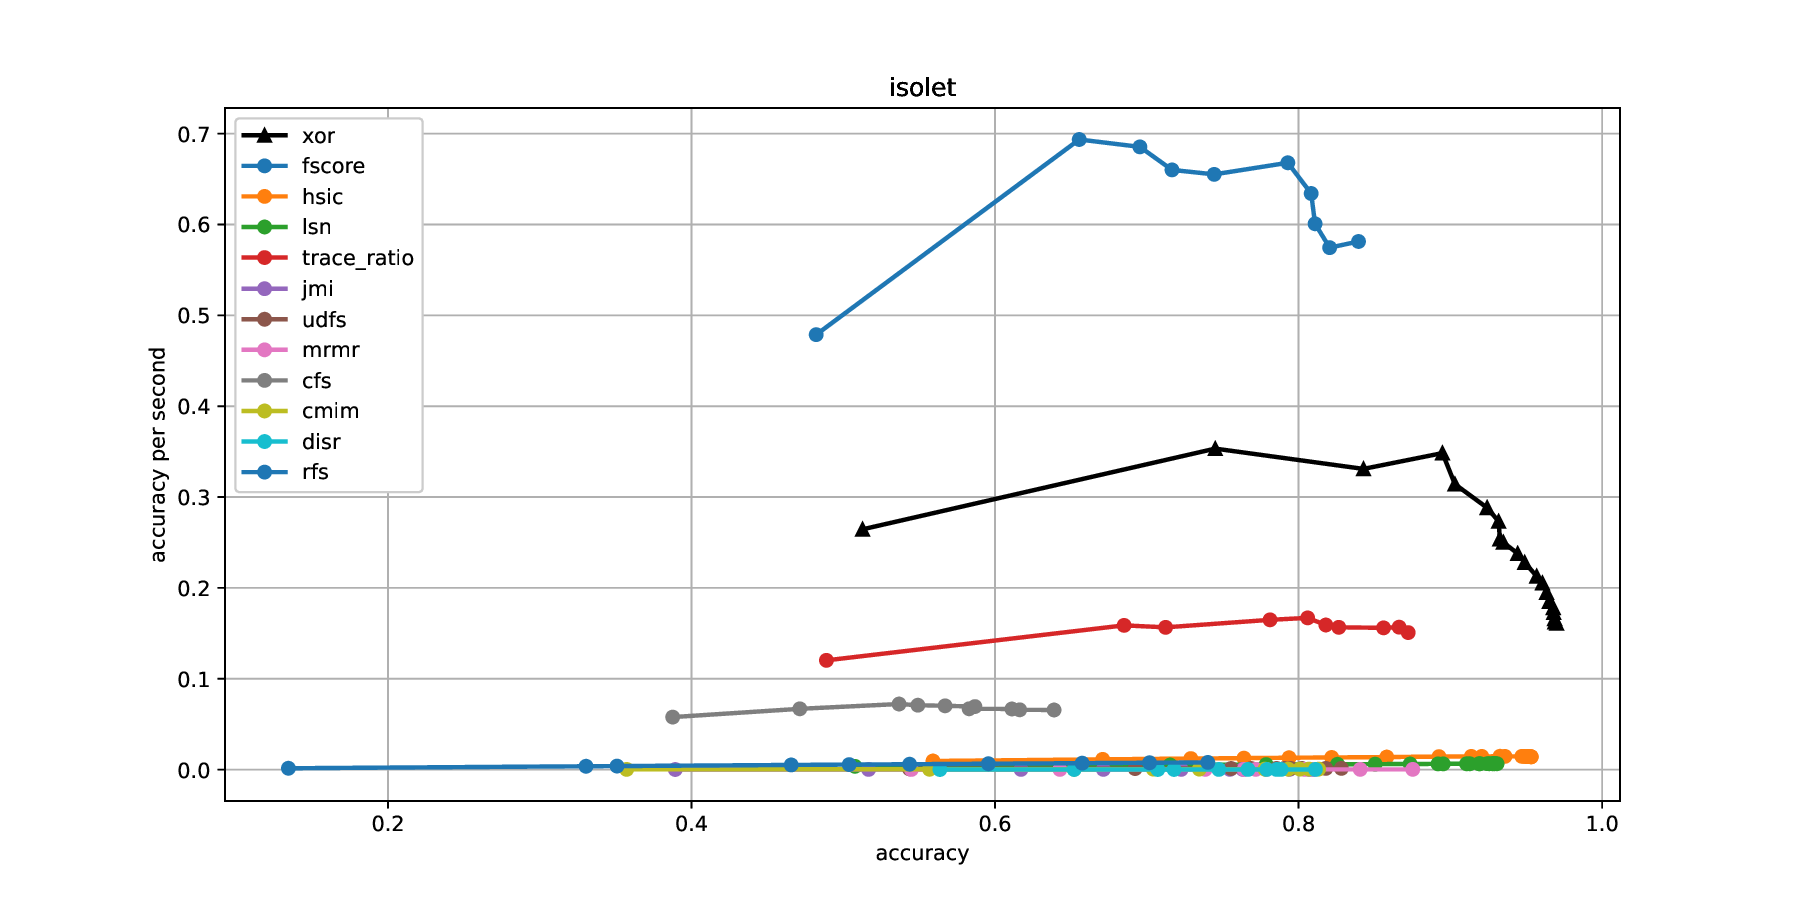}
		\caption{}
	\end{subfigure}
	\begin{subfigure}[b]{0.48\textwidth}	%4
		\includegraphics[width=\textwidth]{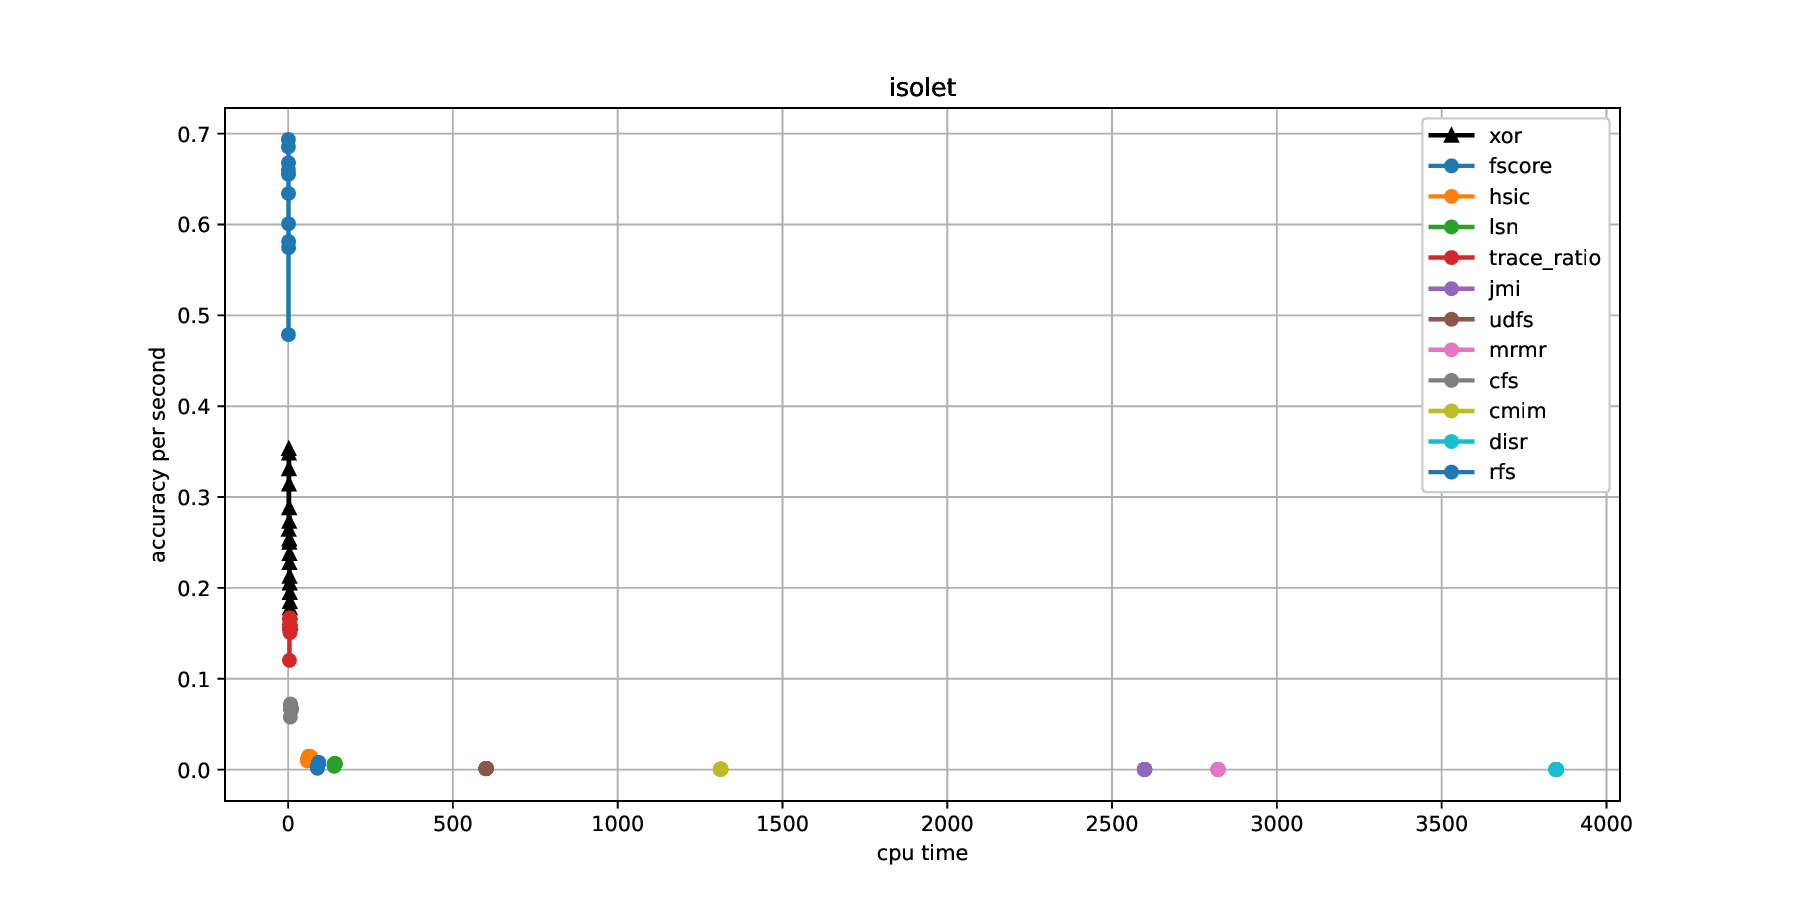}
		\caption{}
	\end{subfigure}
	
	\begin{subfigure}[b]{0.48\textwidth}%5
		\includegraphics[width=\textwidth]{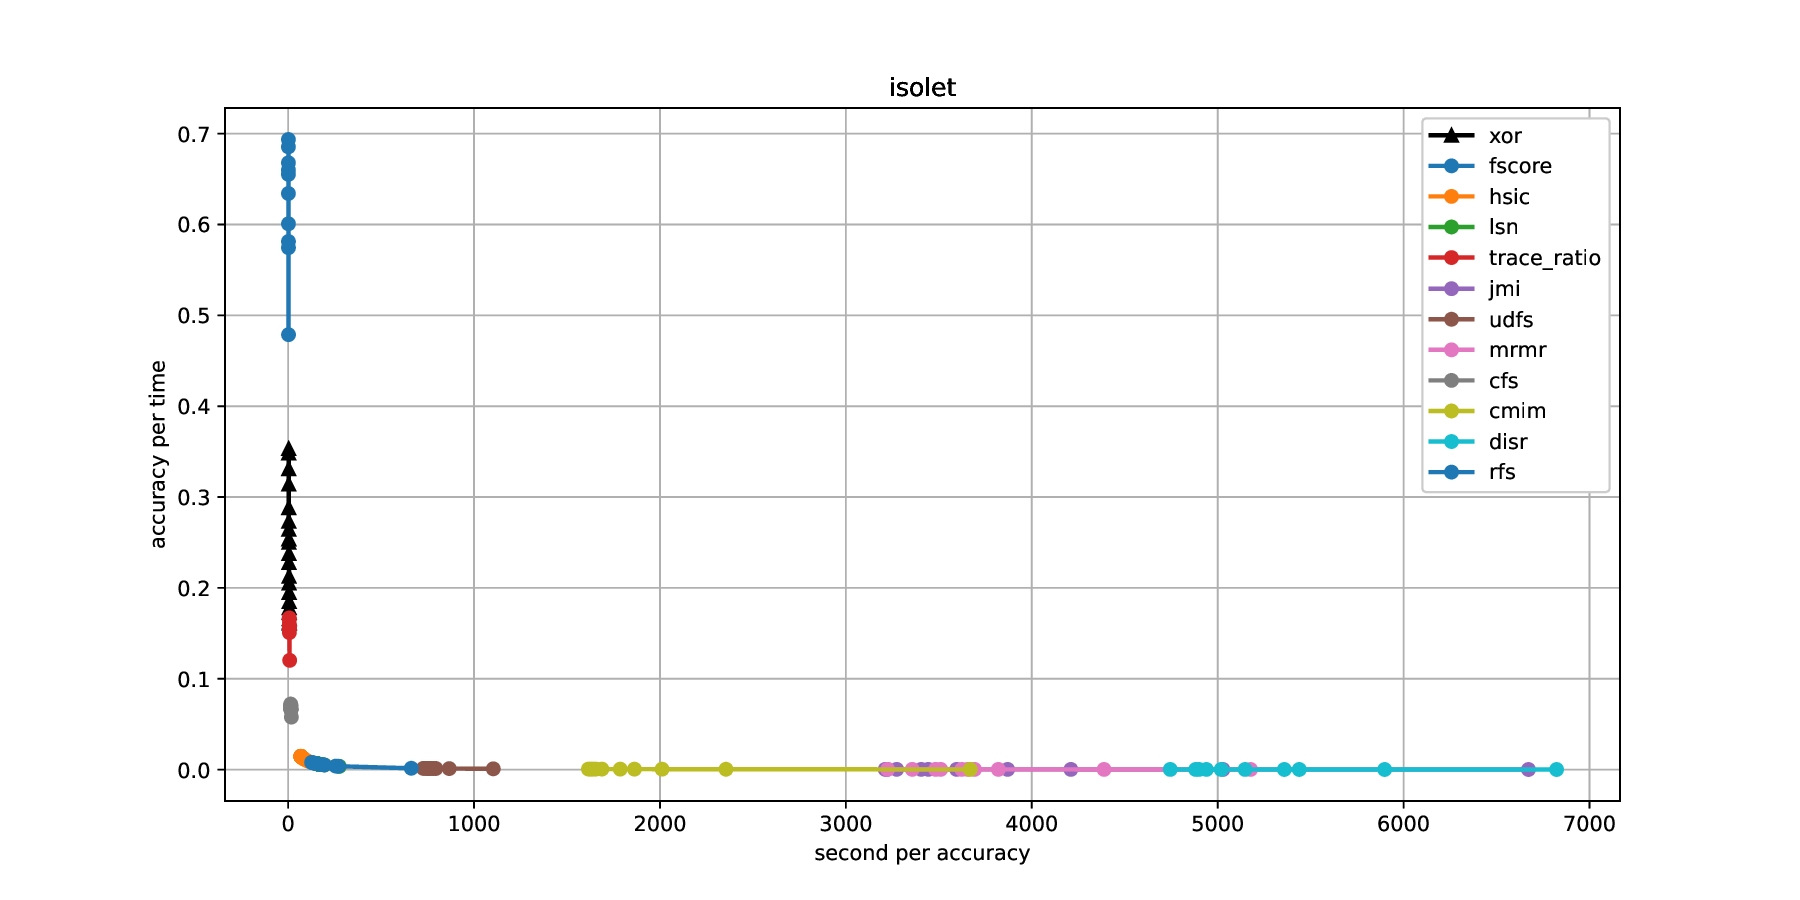}
		\caption{}
	\end{subfigure}
	\begin{subfigure}[b]{0.48\textwidth}	%6
		\includegraphics[width=\textwidth]{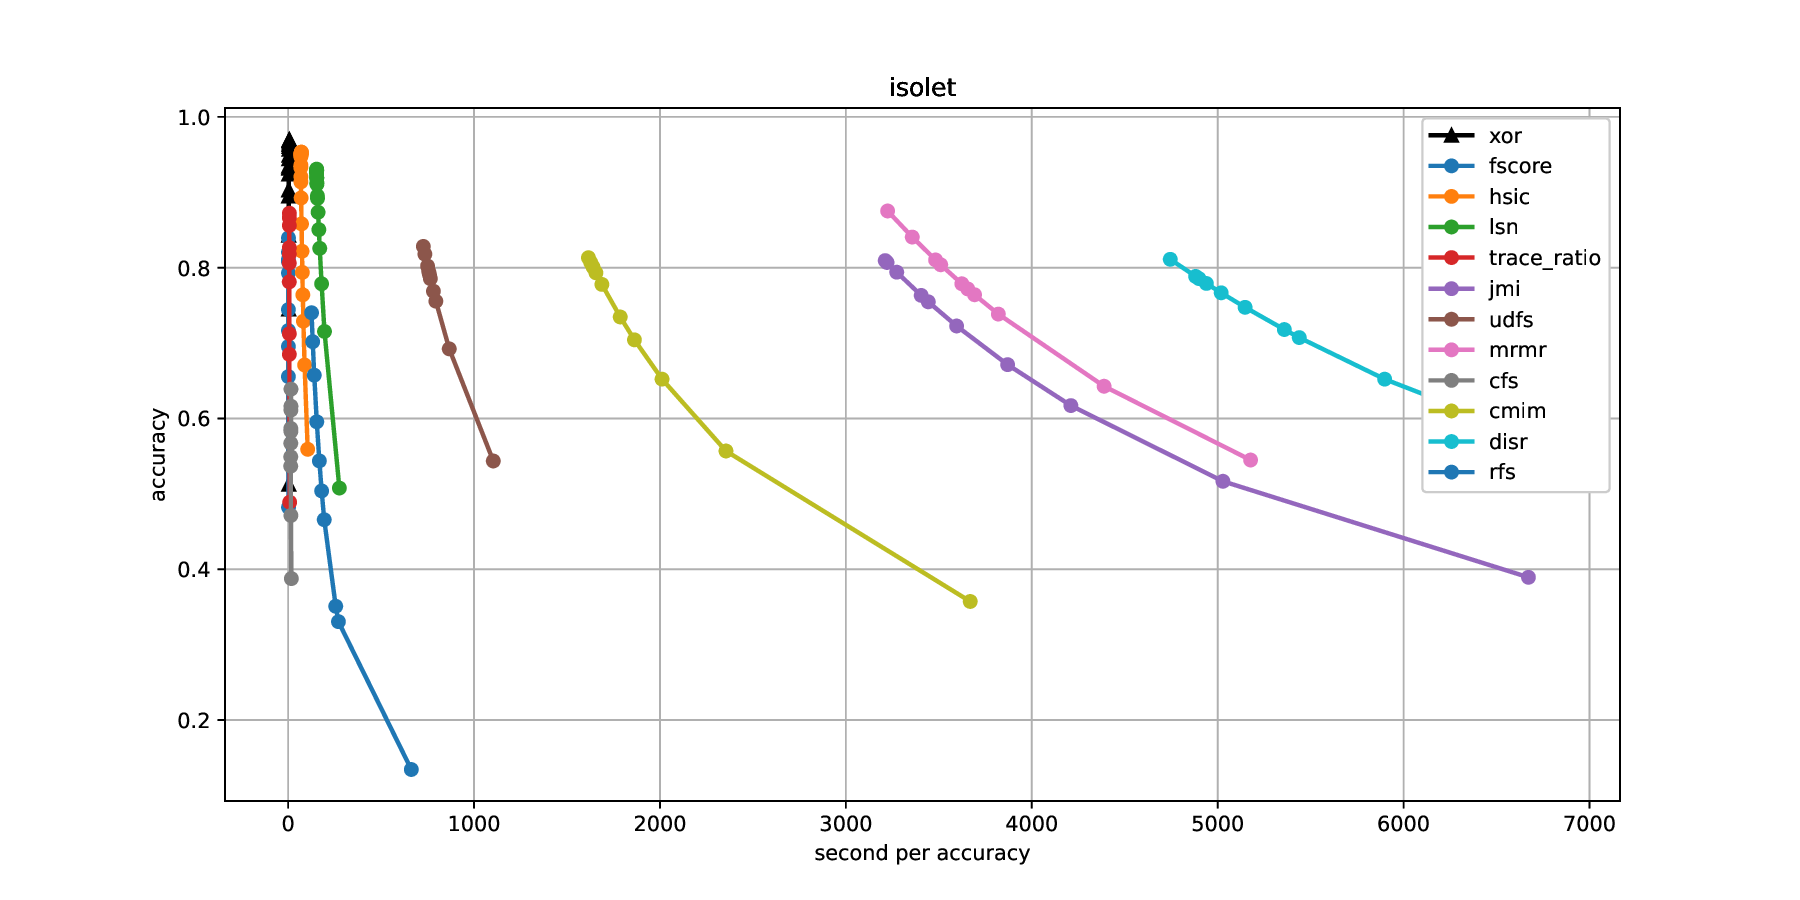}
		\caption{}	
	\end{subfigure}
	
	\begin{subfigure}[b]{0.48\textwidth}	%7
		\includegraphics[width=\textwidth]{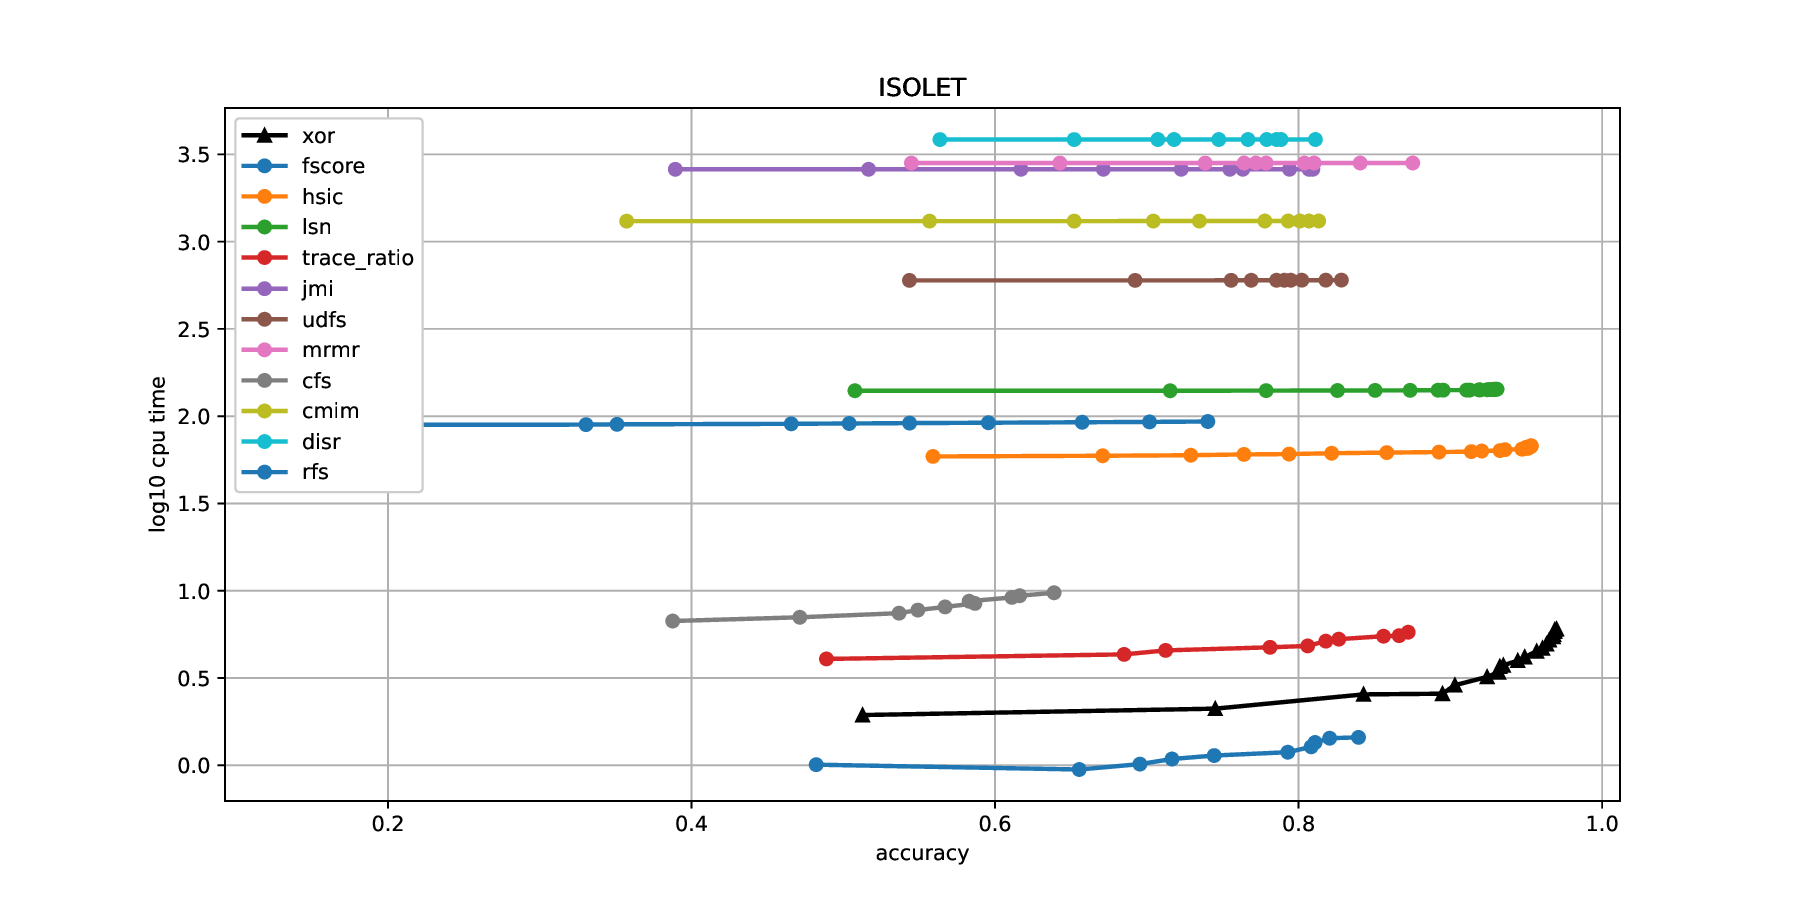}
		\caption{}
	\end{subfigure}
	\begin{subfigure}[b]{0.48\textwidth}	%8
		\includegraphics[width=\textwidth]{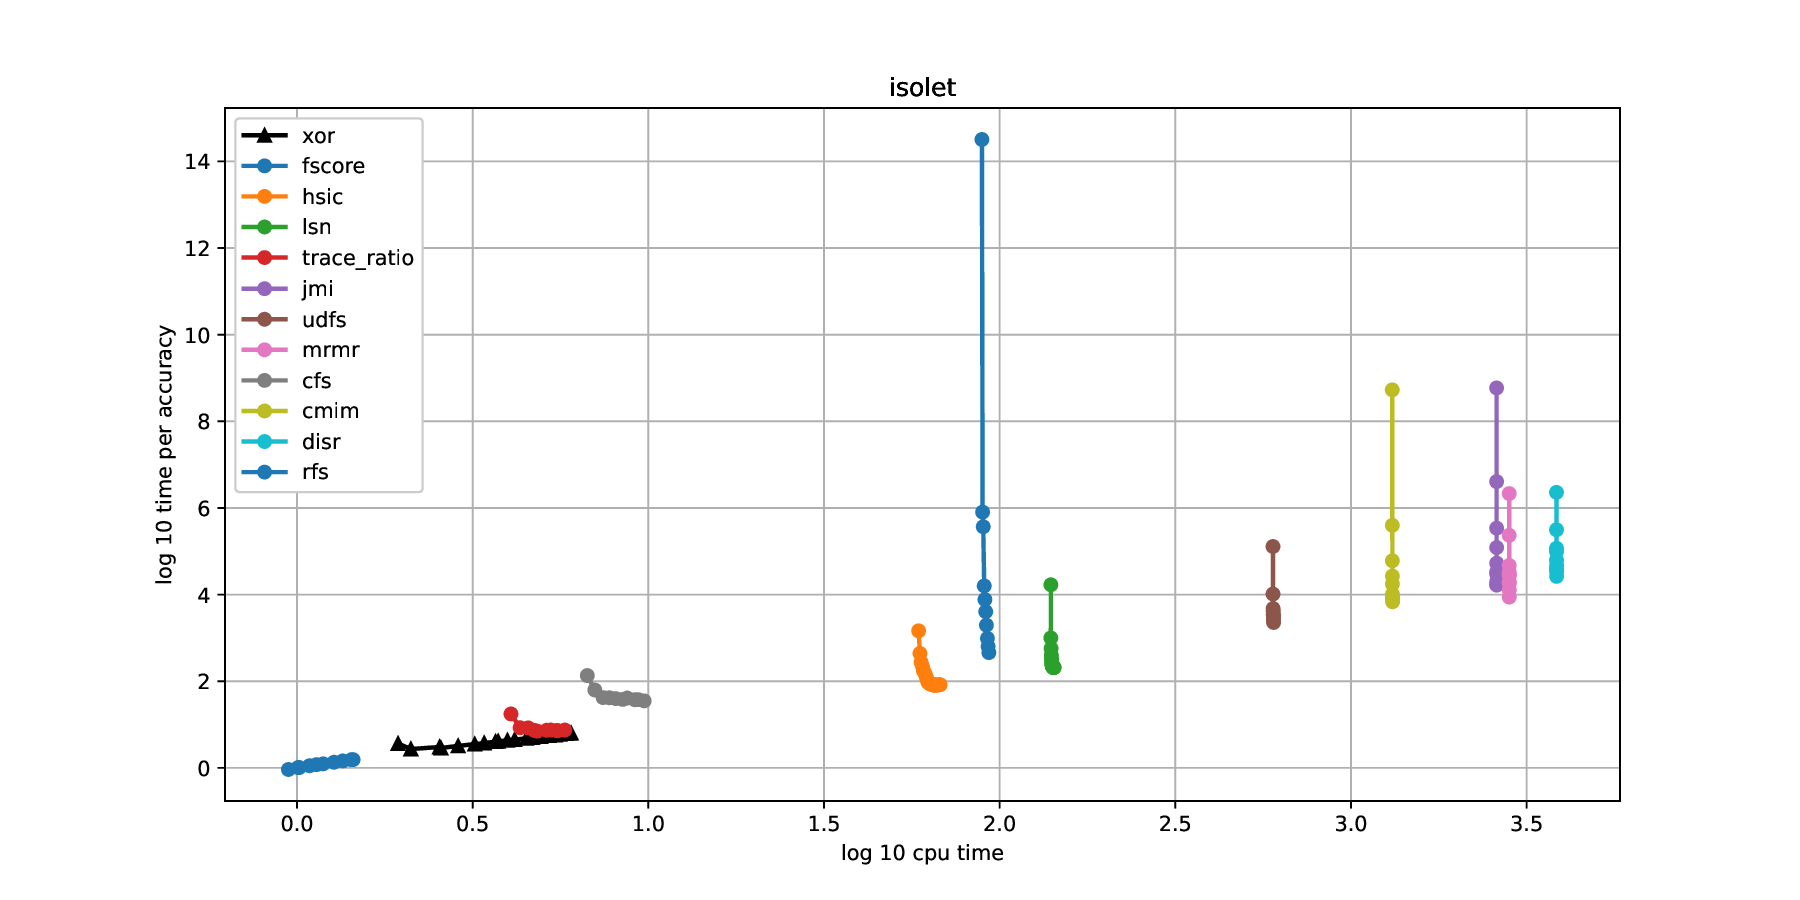}
		\caption{}
	\end{subfigure}
	
	\begin{subfigure}[b]{0.48\textwidth}	%9
		\includegraphics[width=\textwidth]{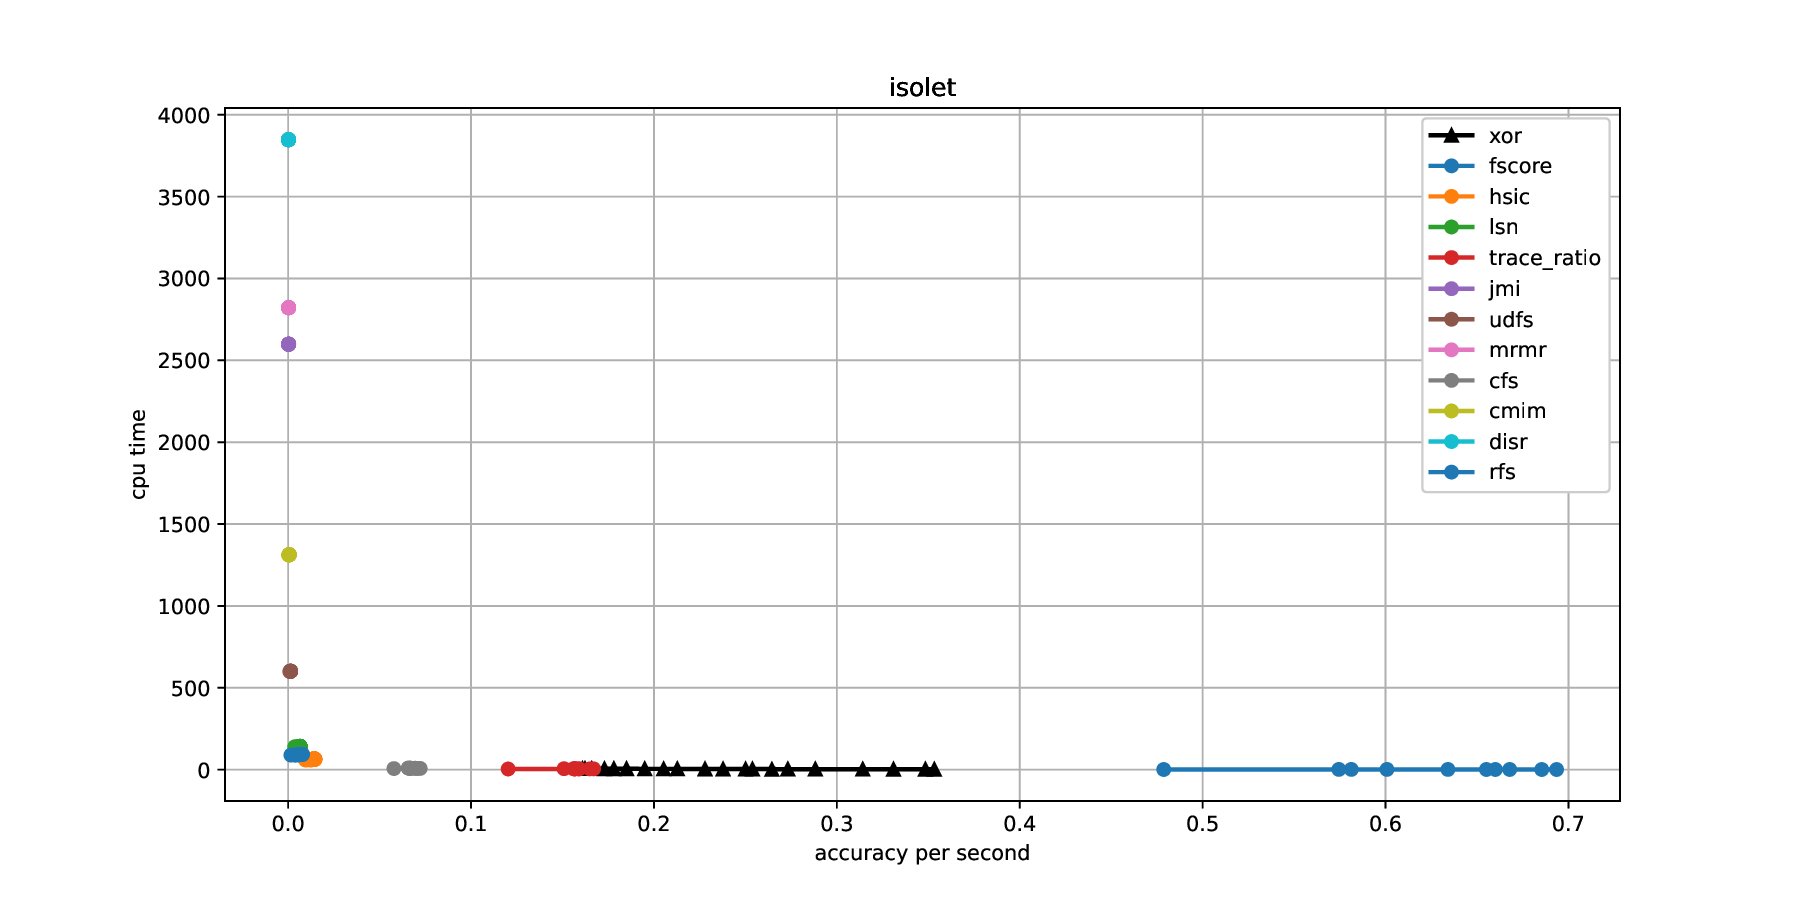}
		\caption{}
	\end{subfigure}
	\begin{subfigure}[b]{0.48\textwidth}	%10
		\includegraphics[width=\textwidth]{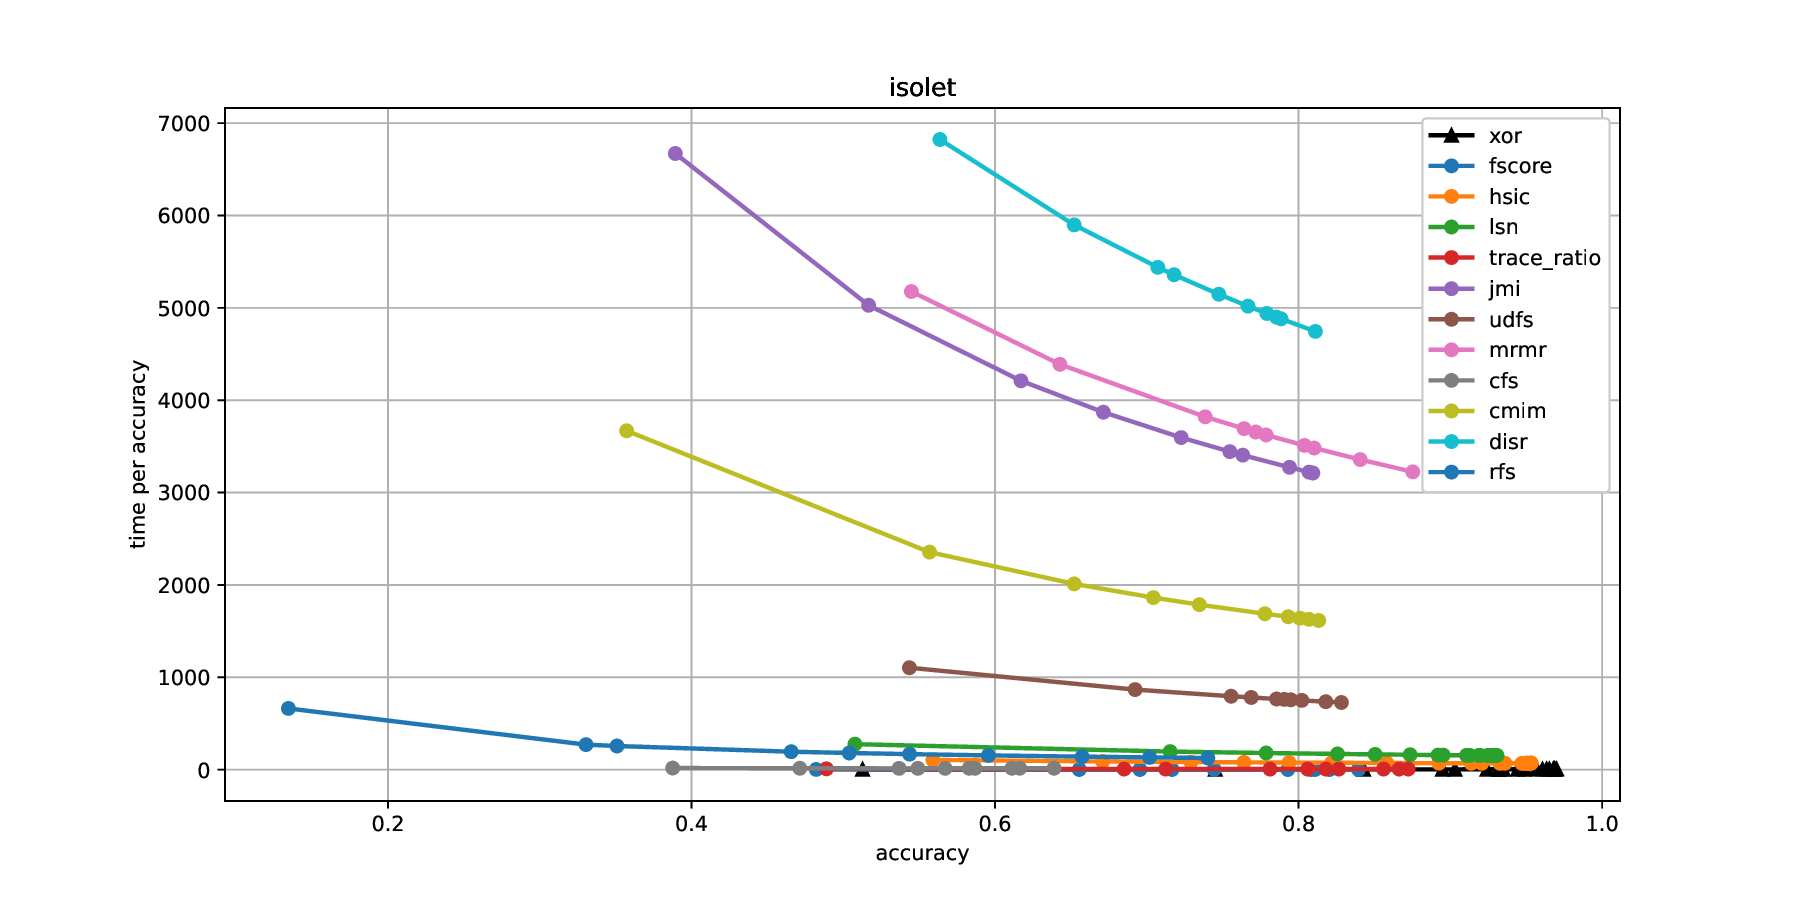}
		\caption{}
	\end{subfigure}
	
	\caption{Time consuming results on ISOLET dataset.}
	\label{time_consuming_comparison_isolet}
\end{figure}

\begin{figure}[!h]
	\centering
	%\vspace{-2cm}
	%\hspace{-2cm}
	\begin{subfigure}[b]{0.48\textwidth}	%1
		\includegraphics[width=\textwidth]{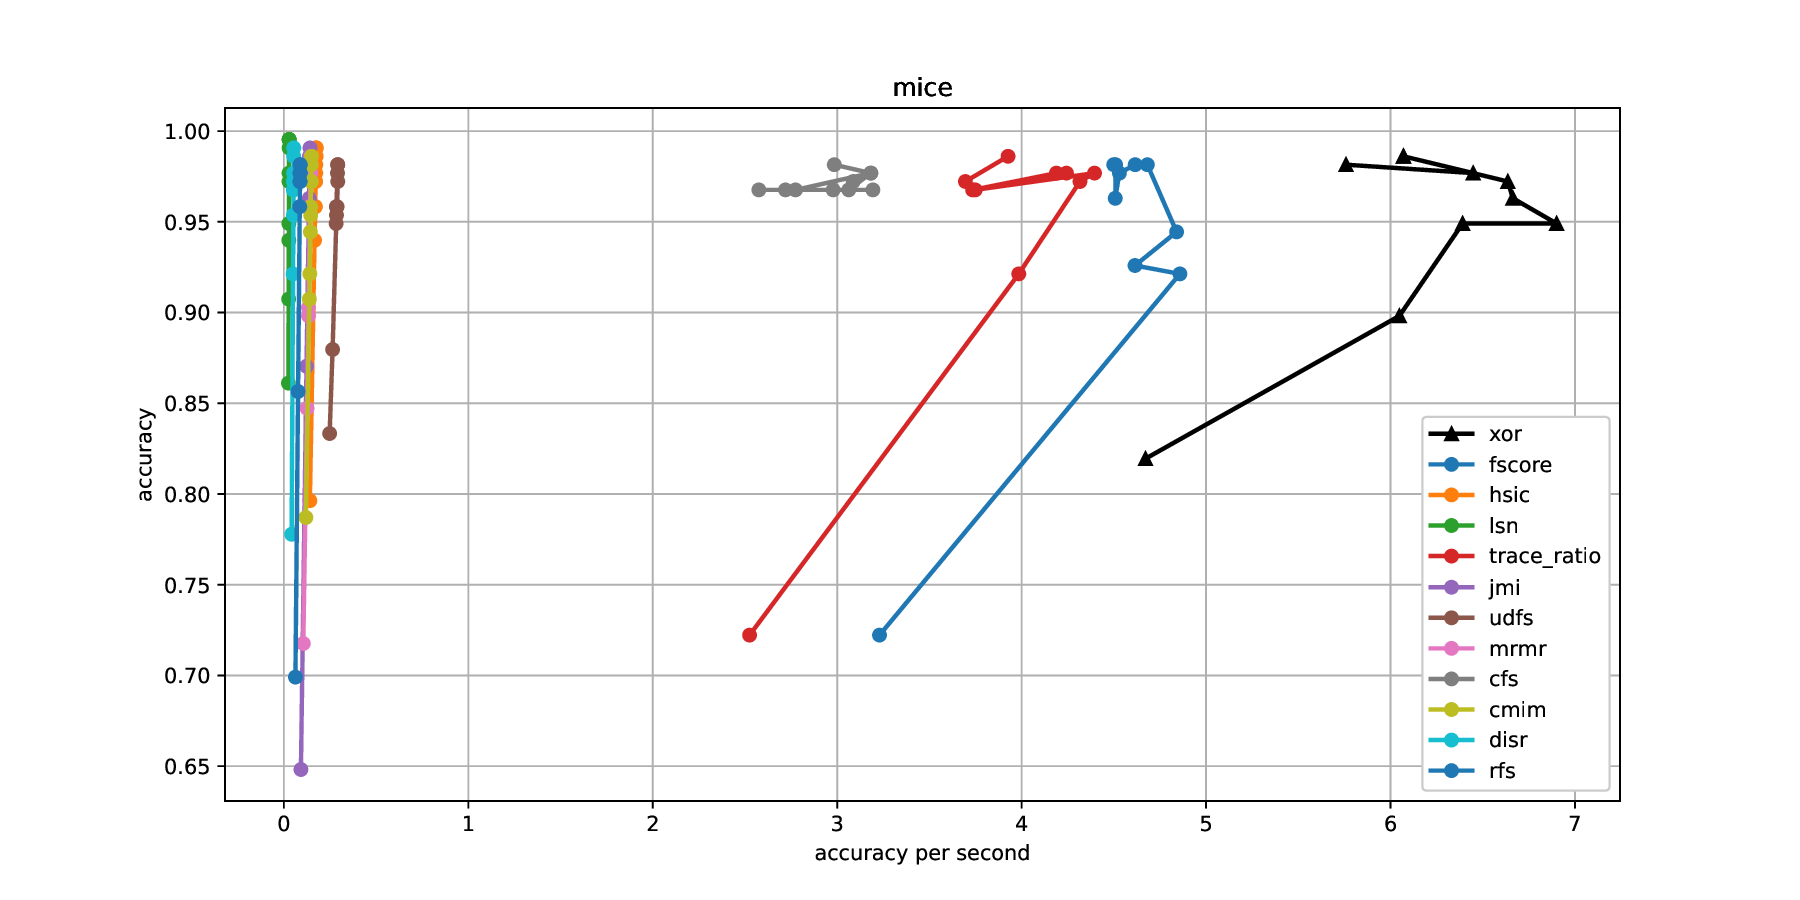} 
		\caption{}
	\end{subfigure}
	\begin{subfigure}[b]{0.48\textwidth}%2
		\includegraphics[width=\textwidth]{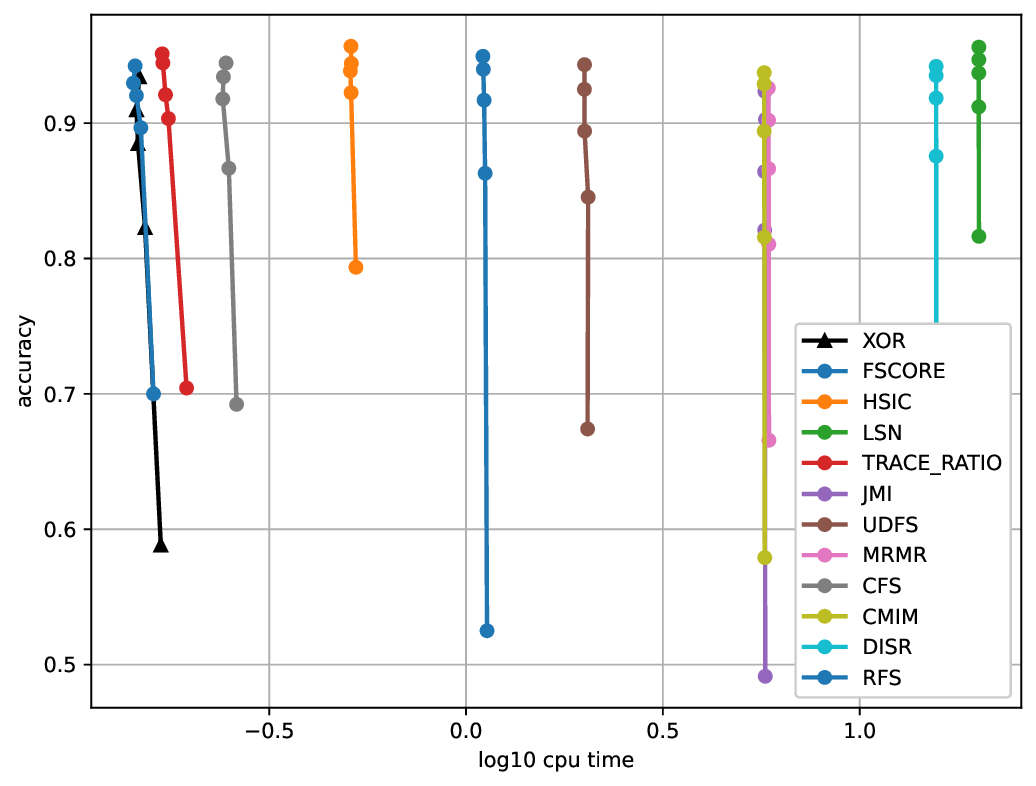}
		\caption{}
	\end{subfigure}
	
	\begin{subfigure}[b]{0.48\textwidth}	%3
		\includegraphics[width=\textwidth]{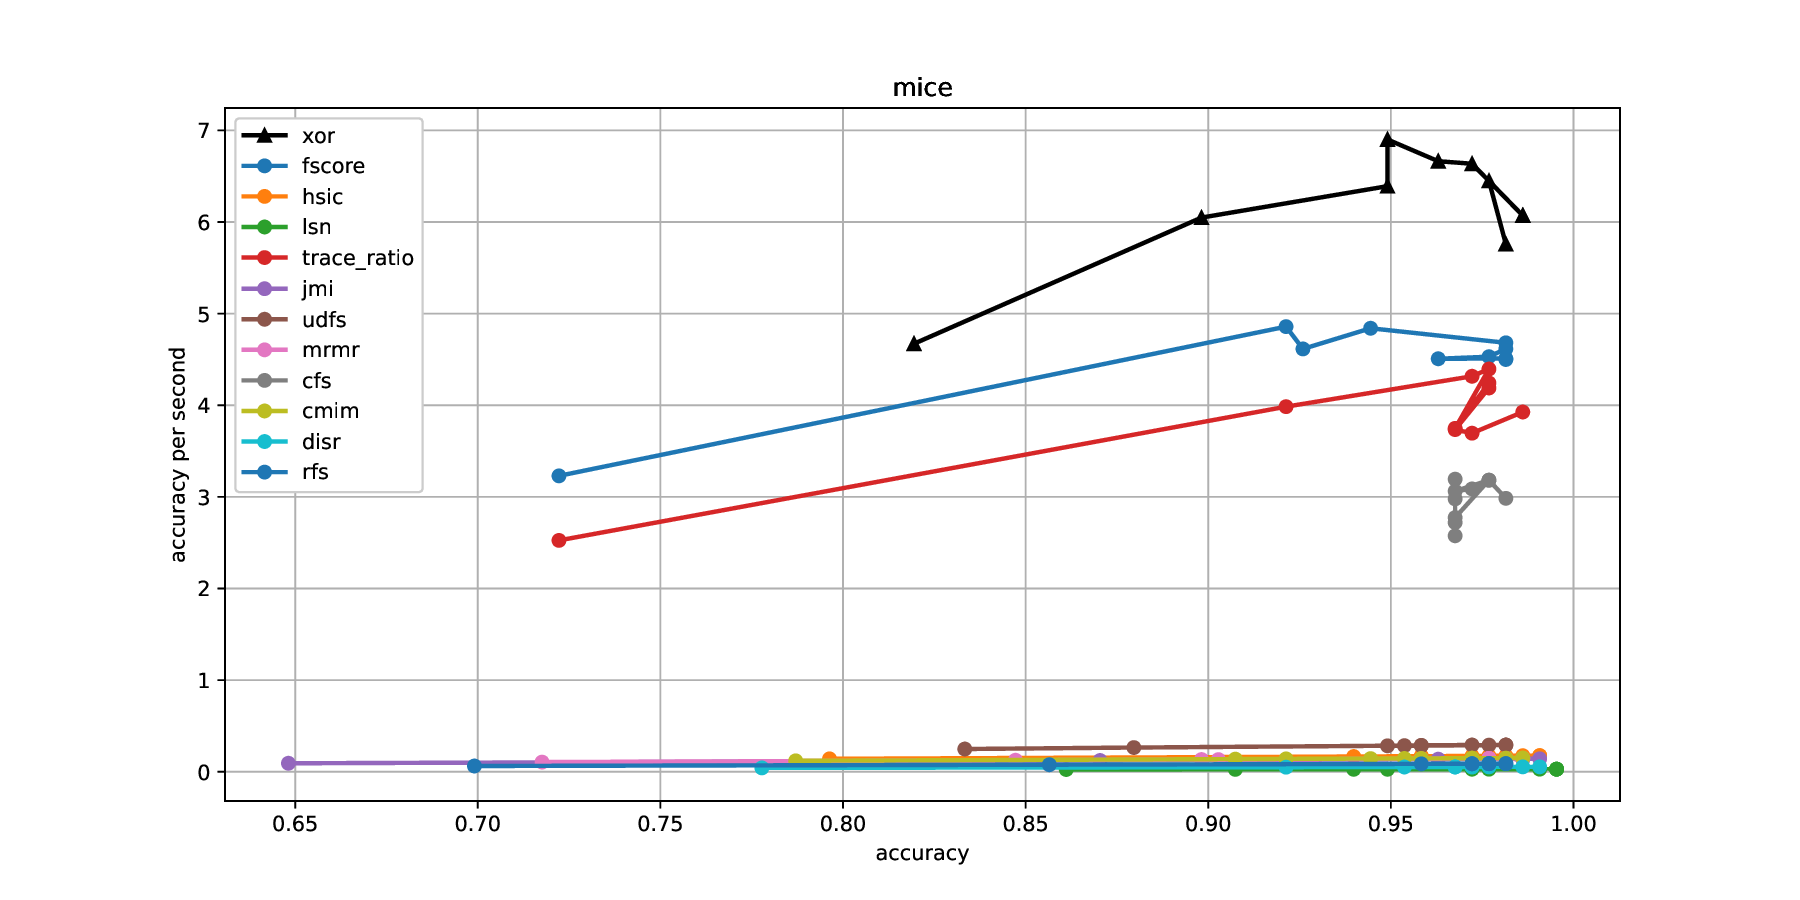}
		\caption{}
	\end{subfigure}
	\begin{subfigure}[b]{0.48\textwidth}	%4
		\includegraphics[width=\textwidth]{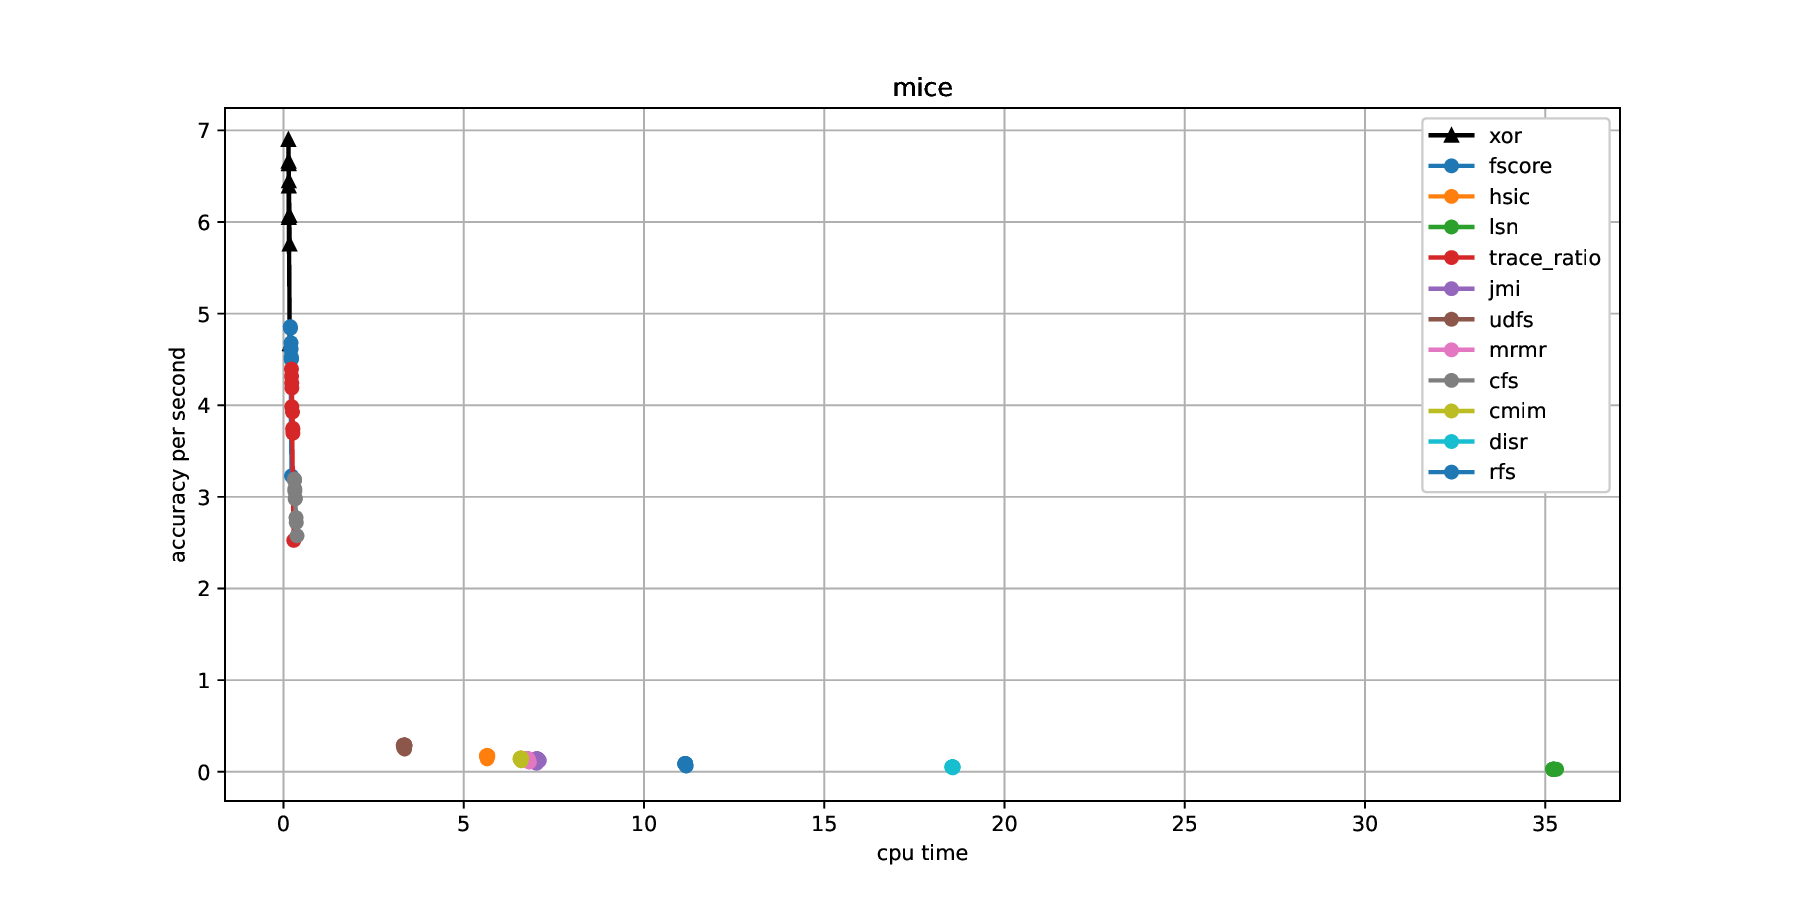}
		\caption{}
	\end{subfigure}
	
	\begin{subfigure}[b]{0.48\textwidth}%5
		\includegraphics[width=\textwidth]{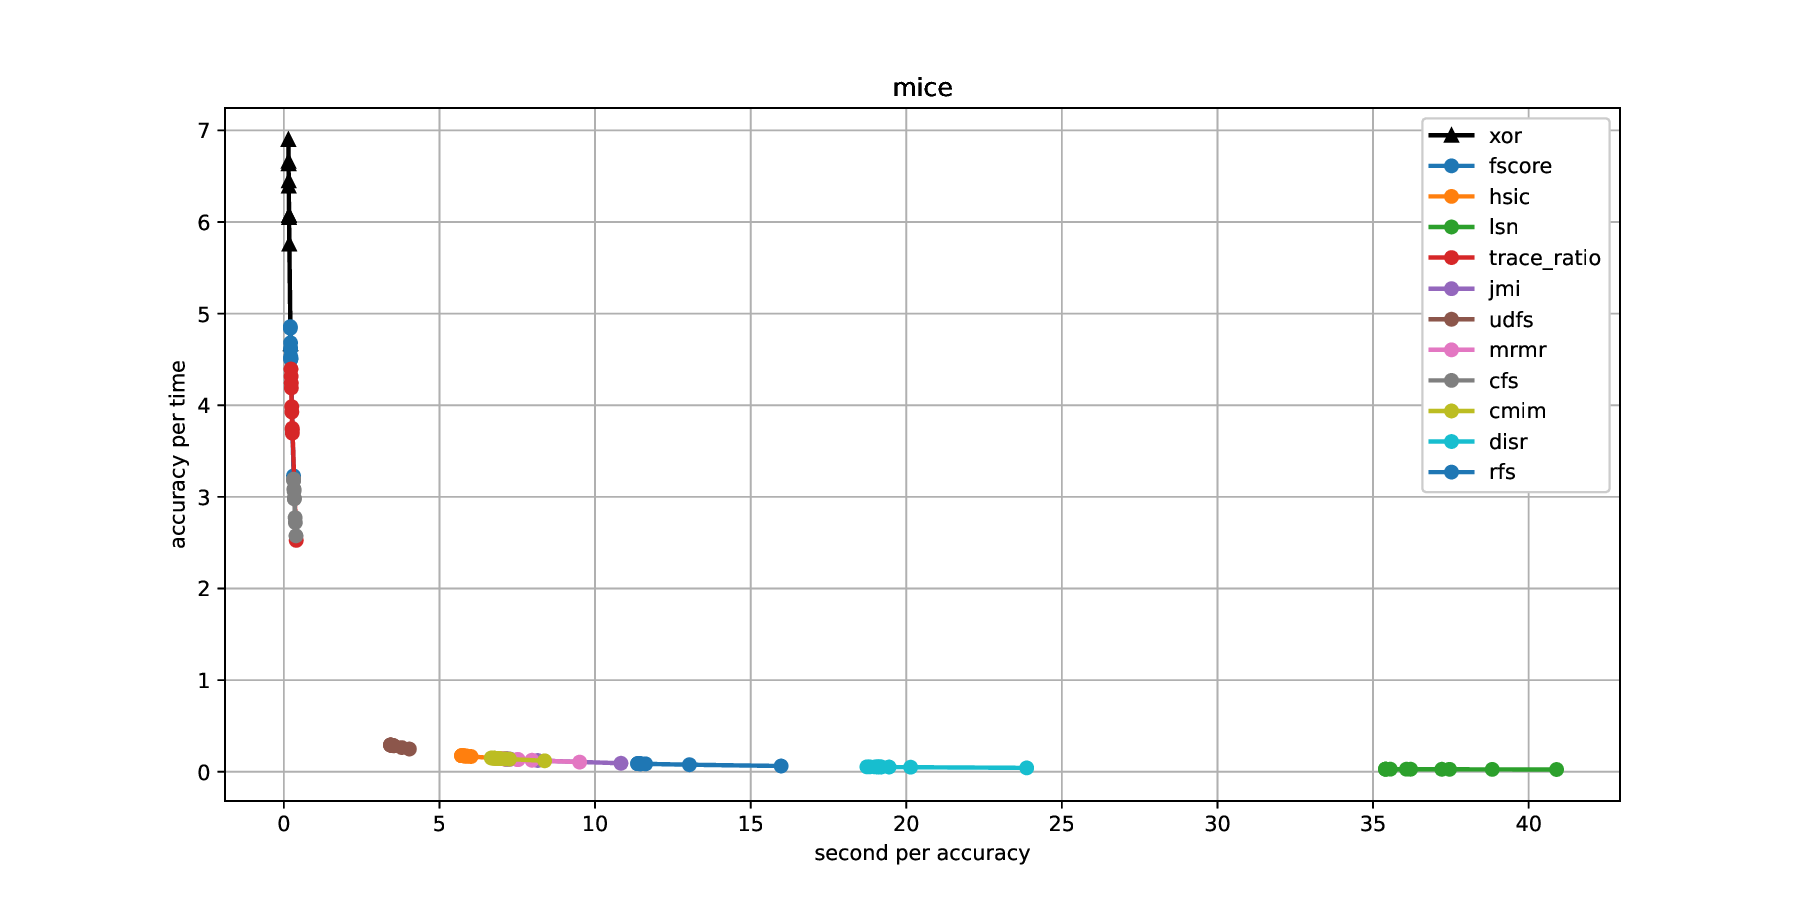}
		\caption{}
	\end{subfigure}
	\begin{subfigure}[b]{0.48\textwidth}	%6
		\includegraphics[width=\textwidth]{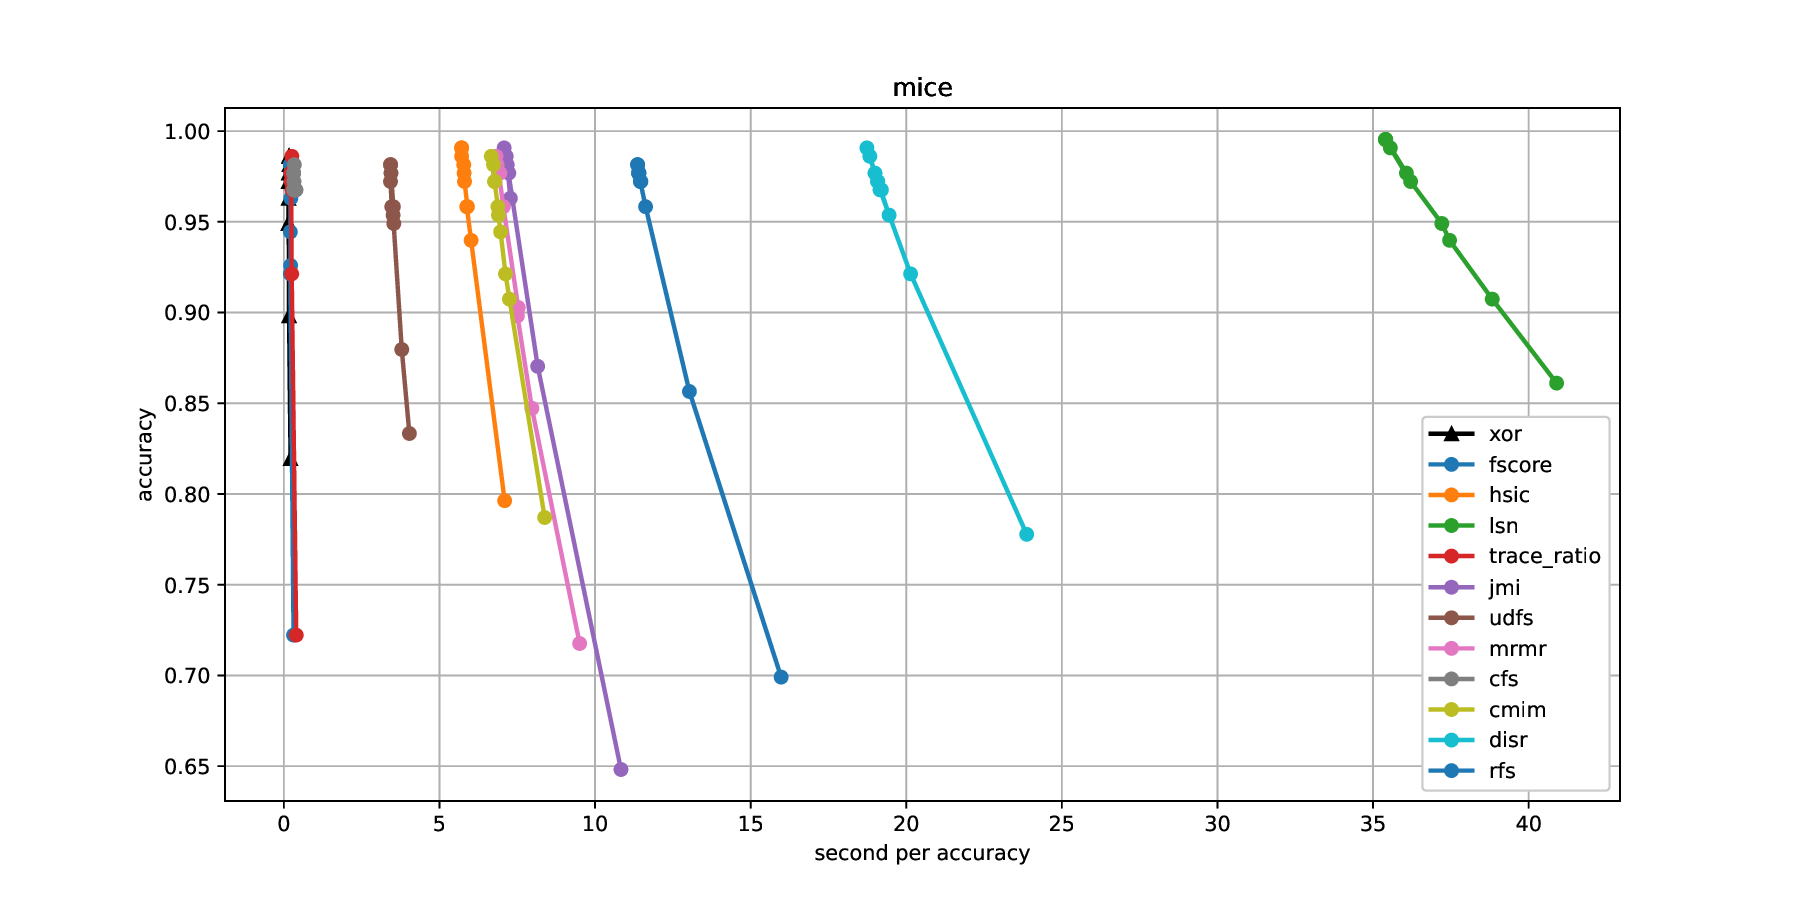}
		\caption{}	
	\end{subfigure}
	
	\begin{subfigure}[b]{0.48\textwidth}	%7
		\includegraphics[width=\textwidth]{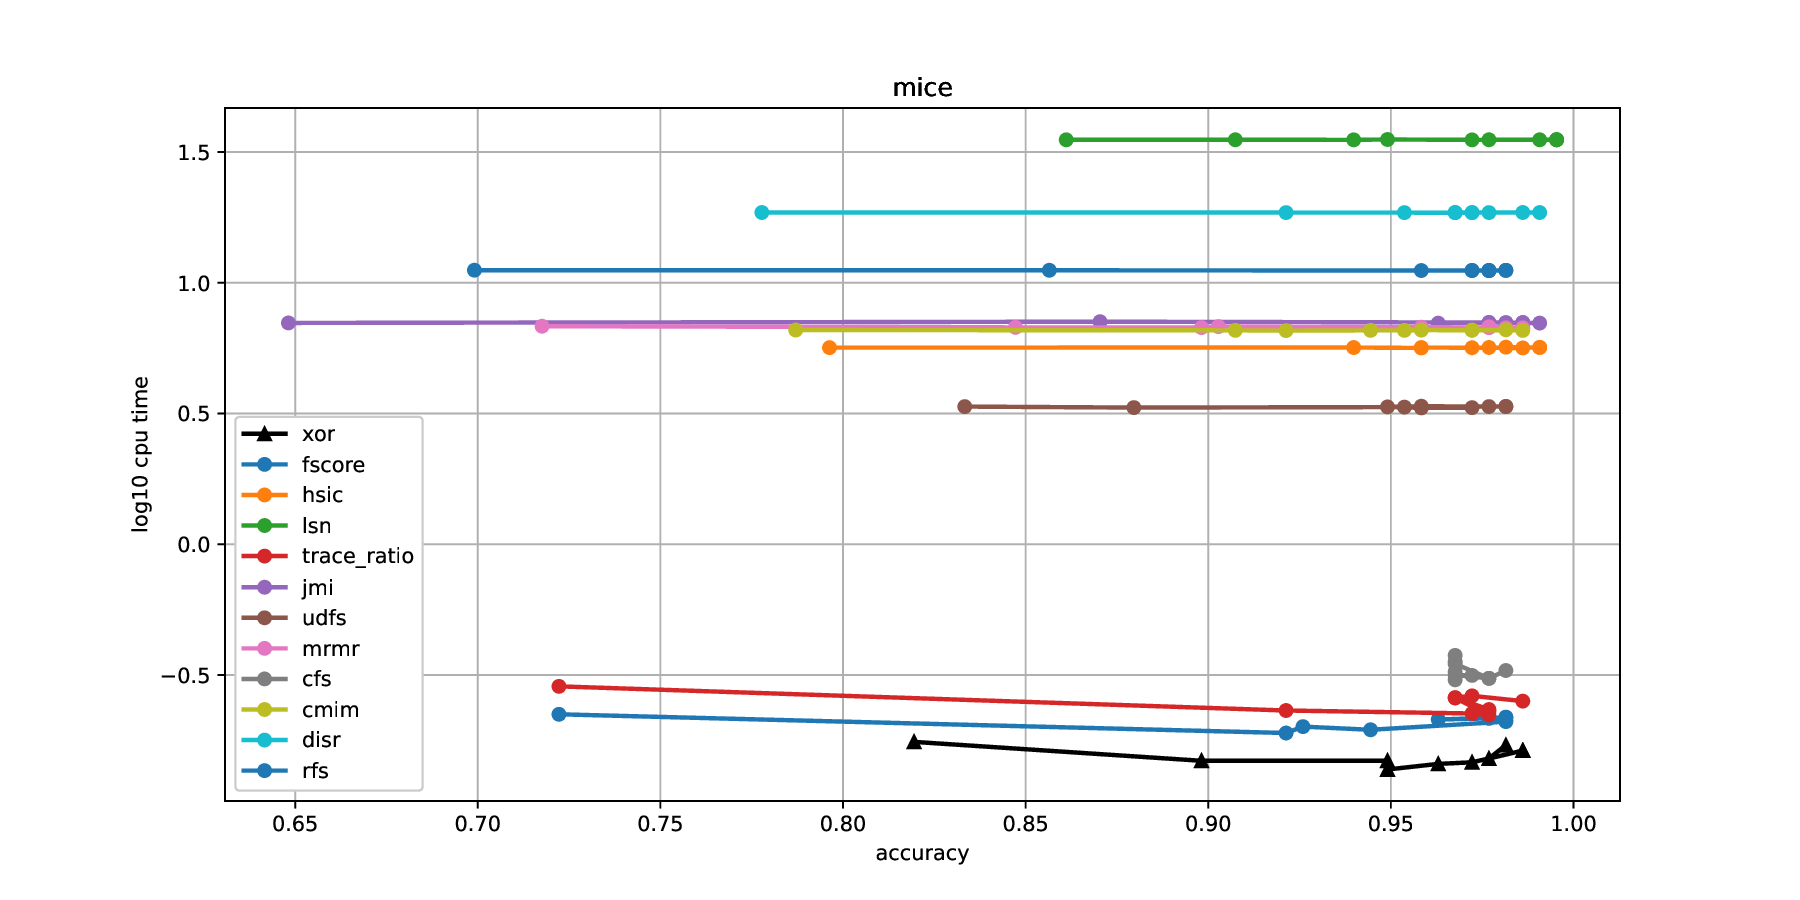}
		\caption{}
	\end{subfigure}
	\begin{subfigure}[b]{0.48\textwidth}	%8
		\includegraphics[width=\textwidth]{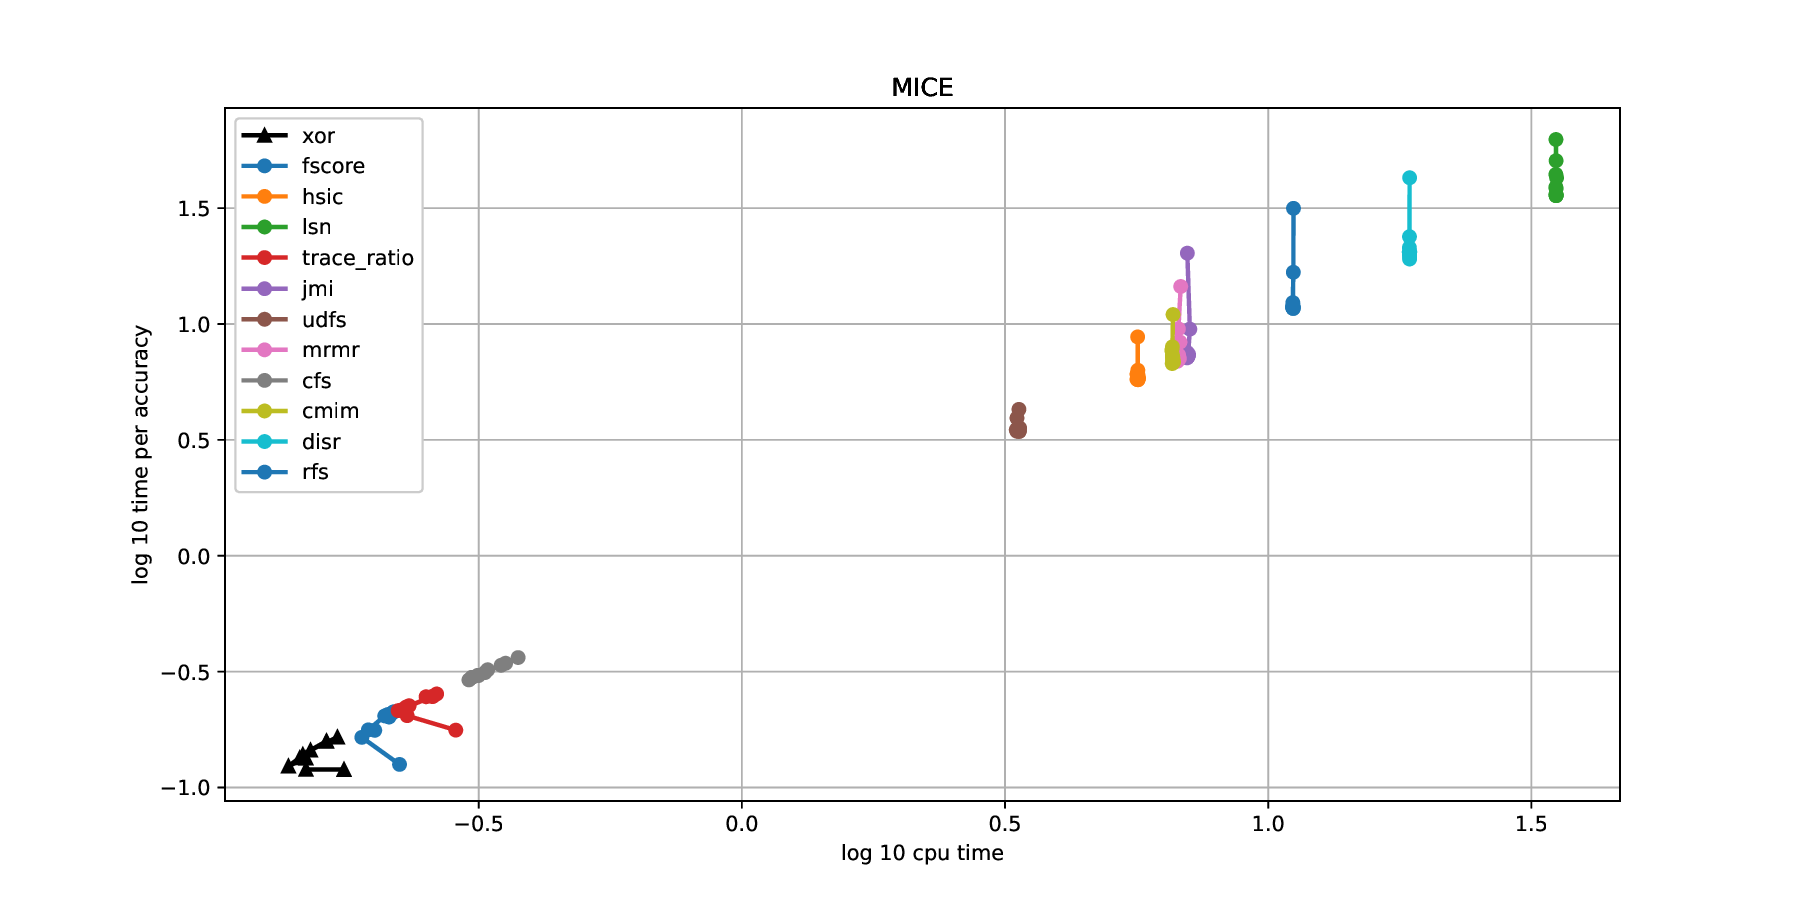}
		\caption{}
	\end{subfigure}
	
	\begin{subfigure}[b]{0.48\textwidth}	%9
		\includegraphics[width=\textwidth]{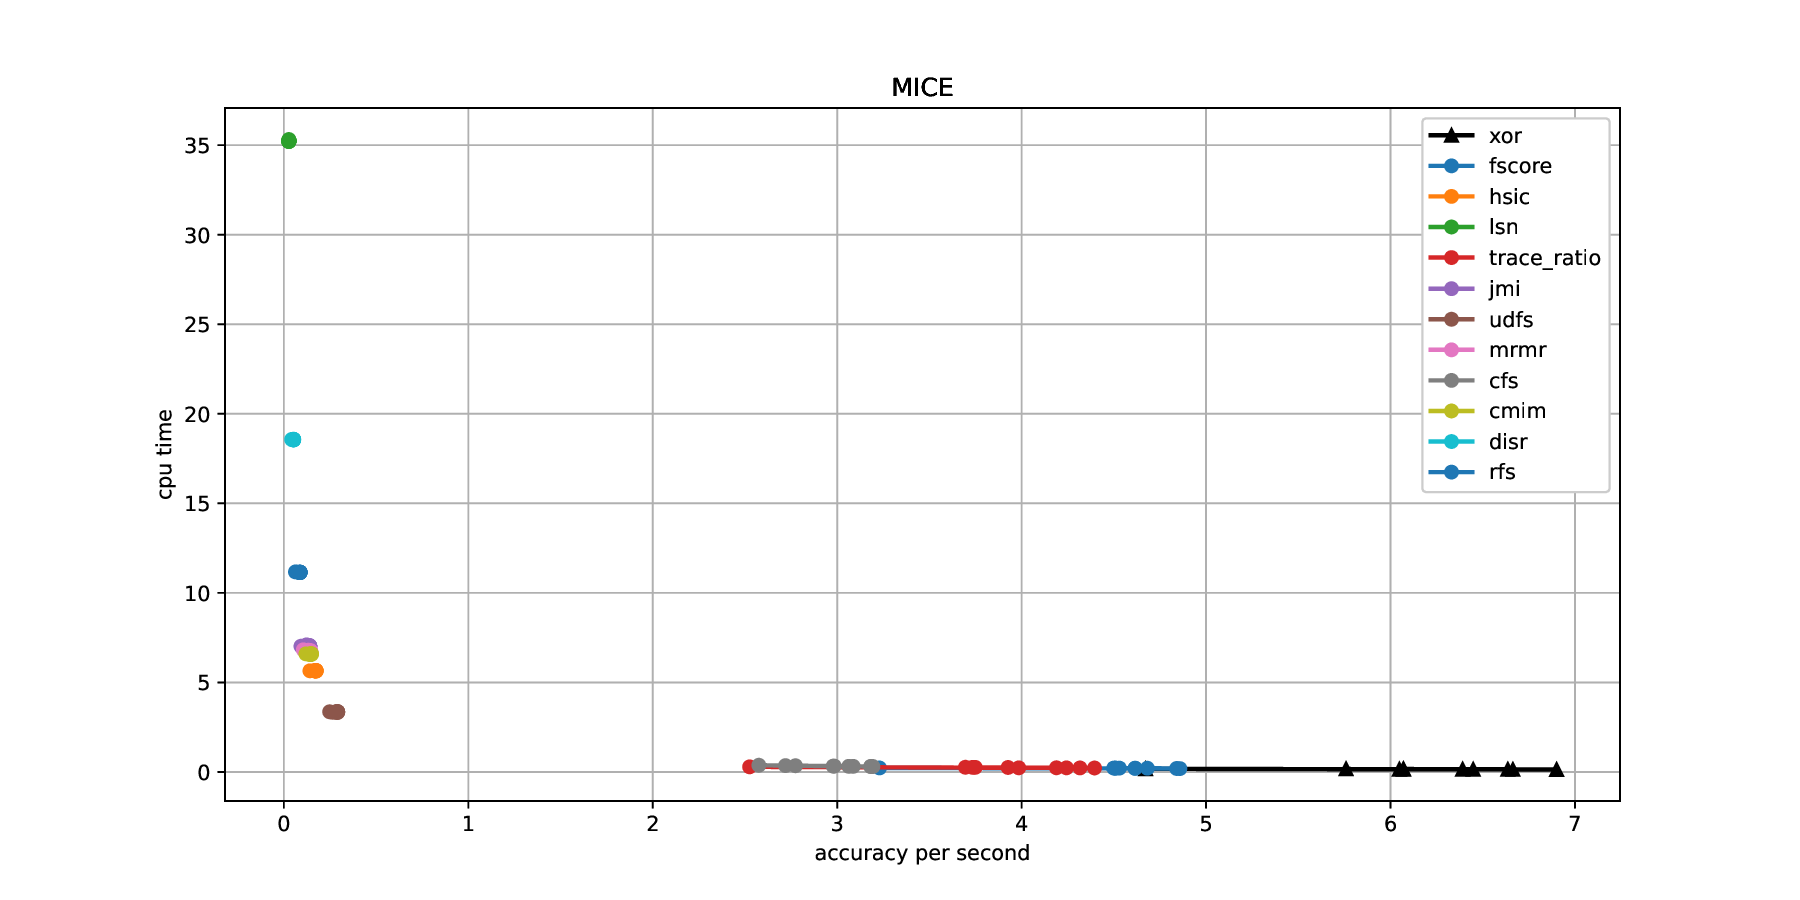}
		\caption{}
	\end{subfigure}
	\begin{subfigure}[b]{0.48\textwidth}	%10
		\includegraphics[width=\textwidth]{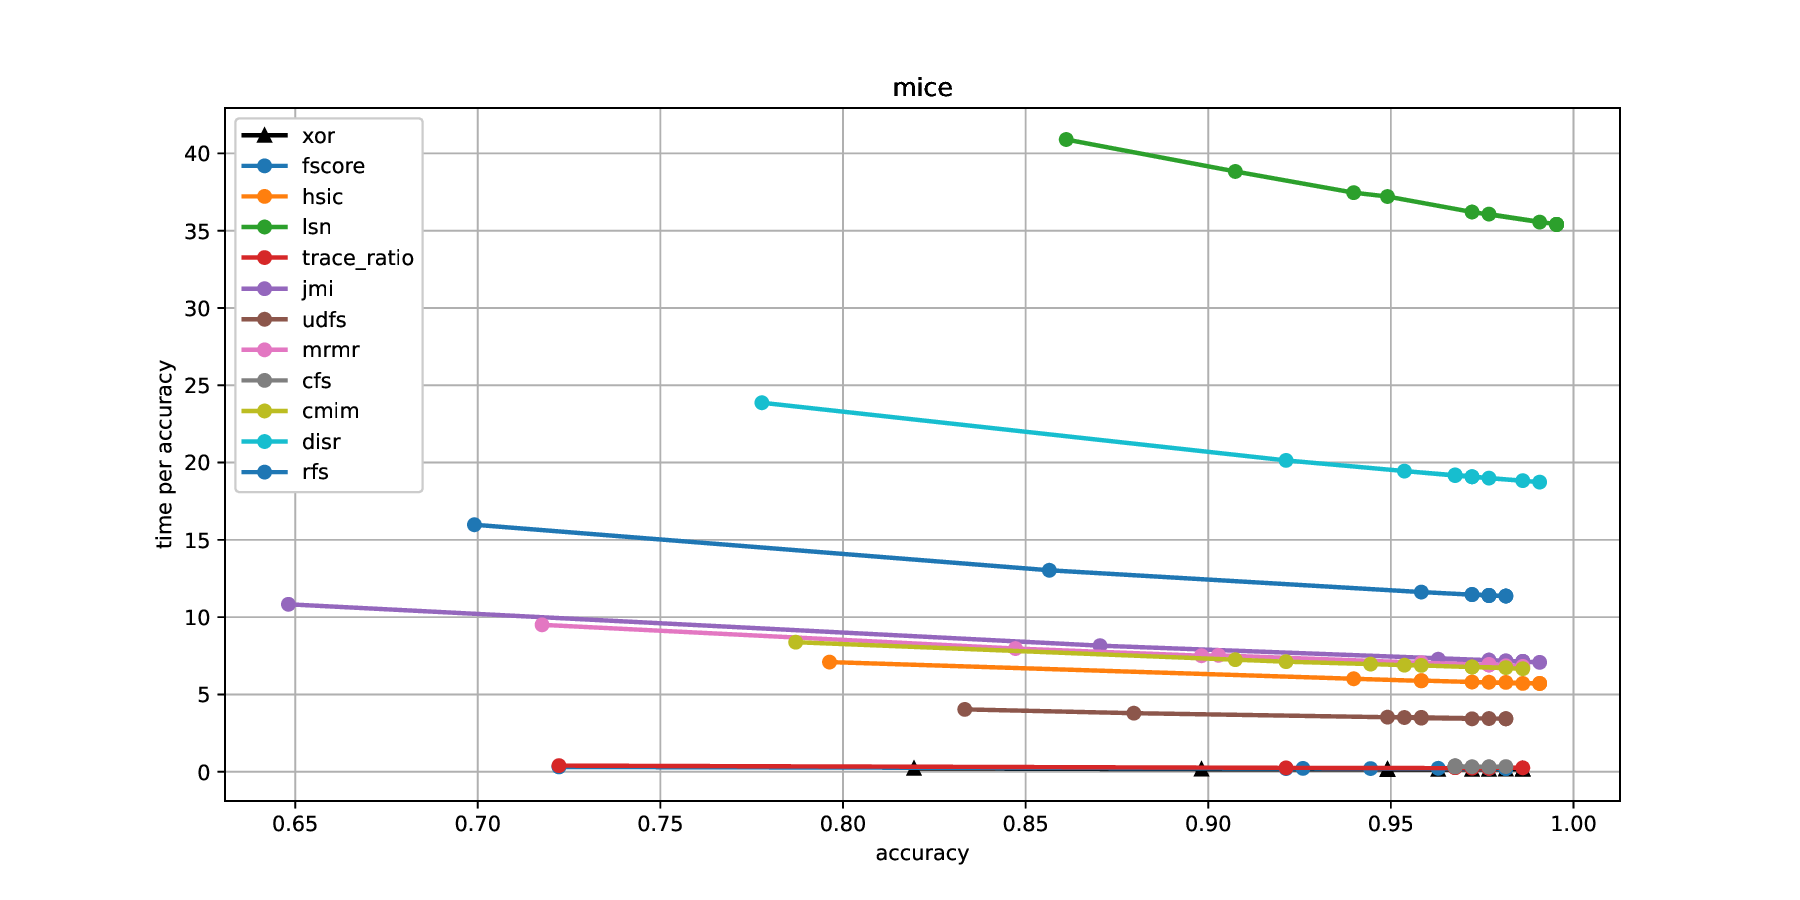}
		\caption{}
	\end{subfigure}
	
	\caption{Time consuming results on MICE dataset.}
	\label{time_consuming_comparison_mice}
\end{figure}

\begin{figure}[!h]
	\centering
	%\vspace{-2cm}
	%\hspace{-2cm}
	\begin{subfigure}[b]{0.48\textwidth}	%1
		\includegraphics[width=\textwidth]{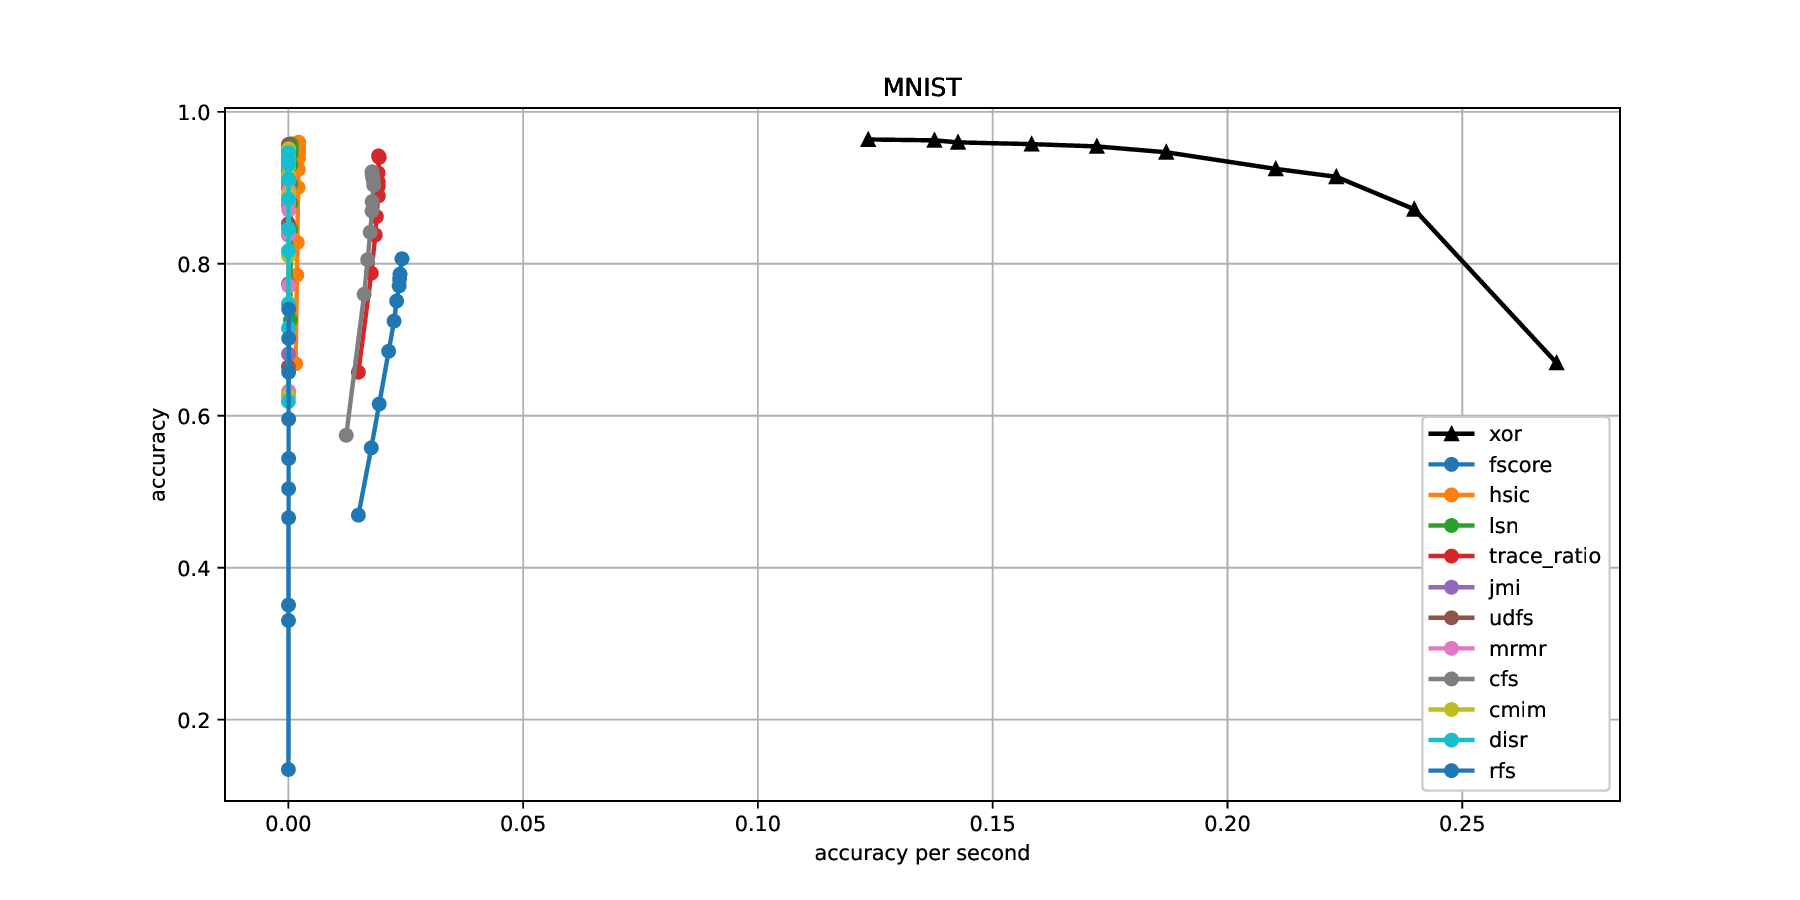} 
		\caption{}
	\end{subfigure}
	\begin{subfigure}[b]{0.48\textwidth}%2
		\includegraphics[width=\textwidth]{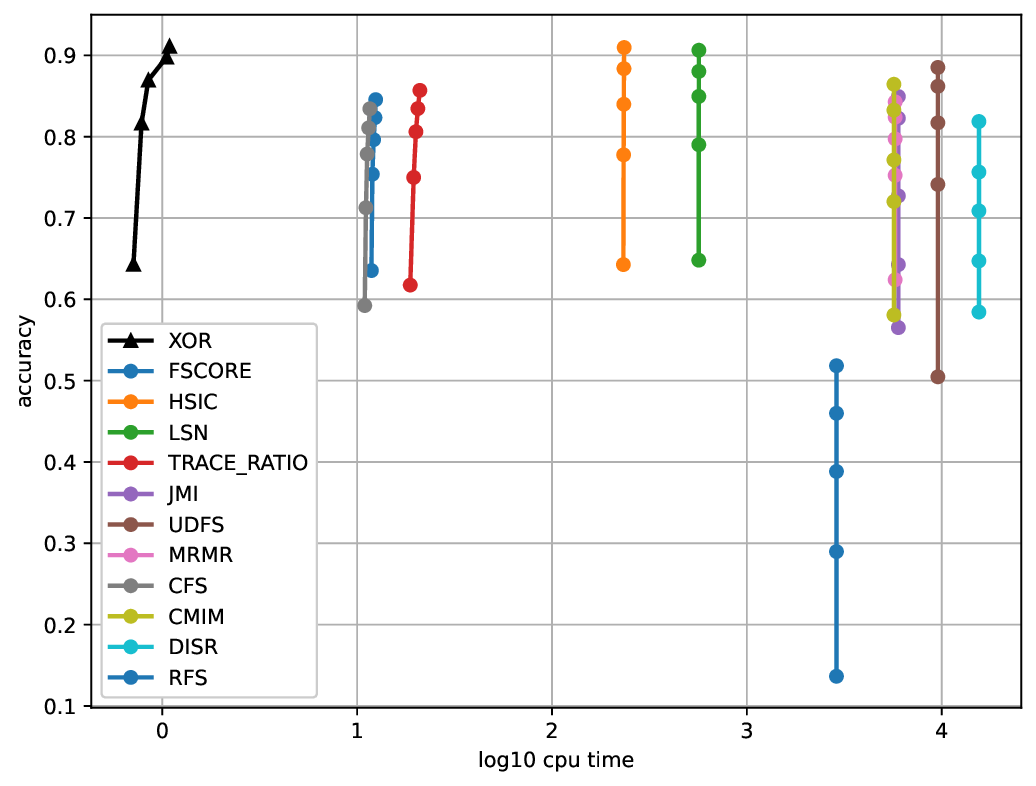}
		\caption{}
	\end{subfigure}
	
	\begin{subfigure}[b]{0.48\textwidth}	%3
		\includegraphics[width=\textwidth]{pic/mnist_acc_per_time_acc.eps}
		\caption{}
	\end{subfigure}
	\begin{subfigure}[b]{0.48\textwidth}	%4
		\includegraphics[width=\textwidth]{pic/mnist_acc_per_time_time.eps}
		\caption{}
	\end{subfigure}
	
	\begin{subfigure}[b]{0.48\textwidth}%5
		\includegraphics[width=\textwidth]{pic/mnist_acc_per_time_time_per_acc.eps}
		\caption{}
	\end{subfigure}
	\begin{subfigure}[b]{0.48\textwidth}	%6
		\includegraphics[width=\textwidth]{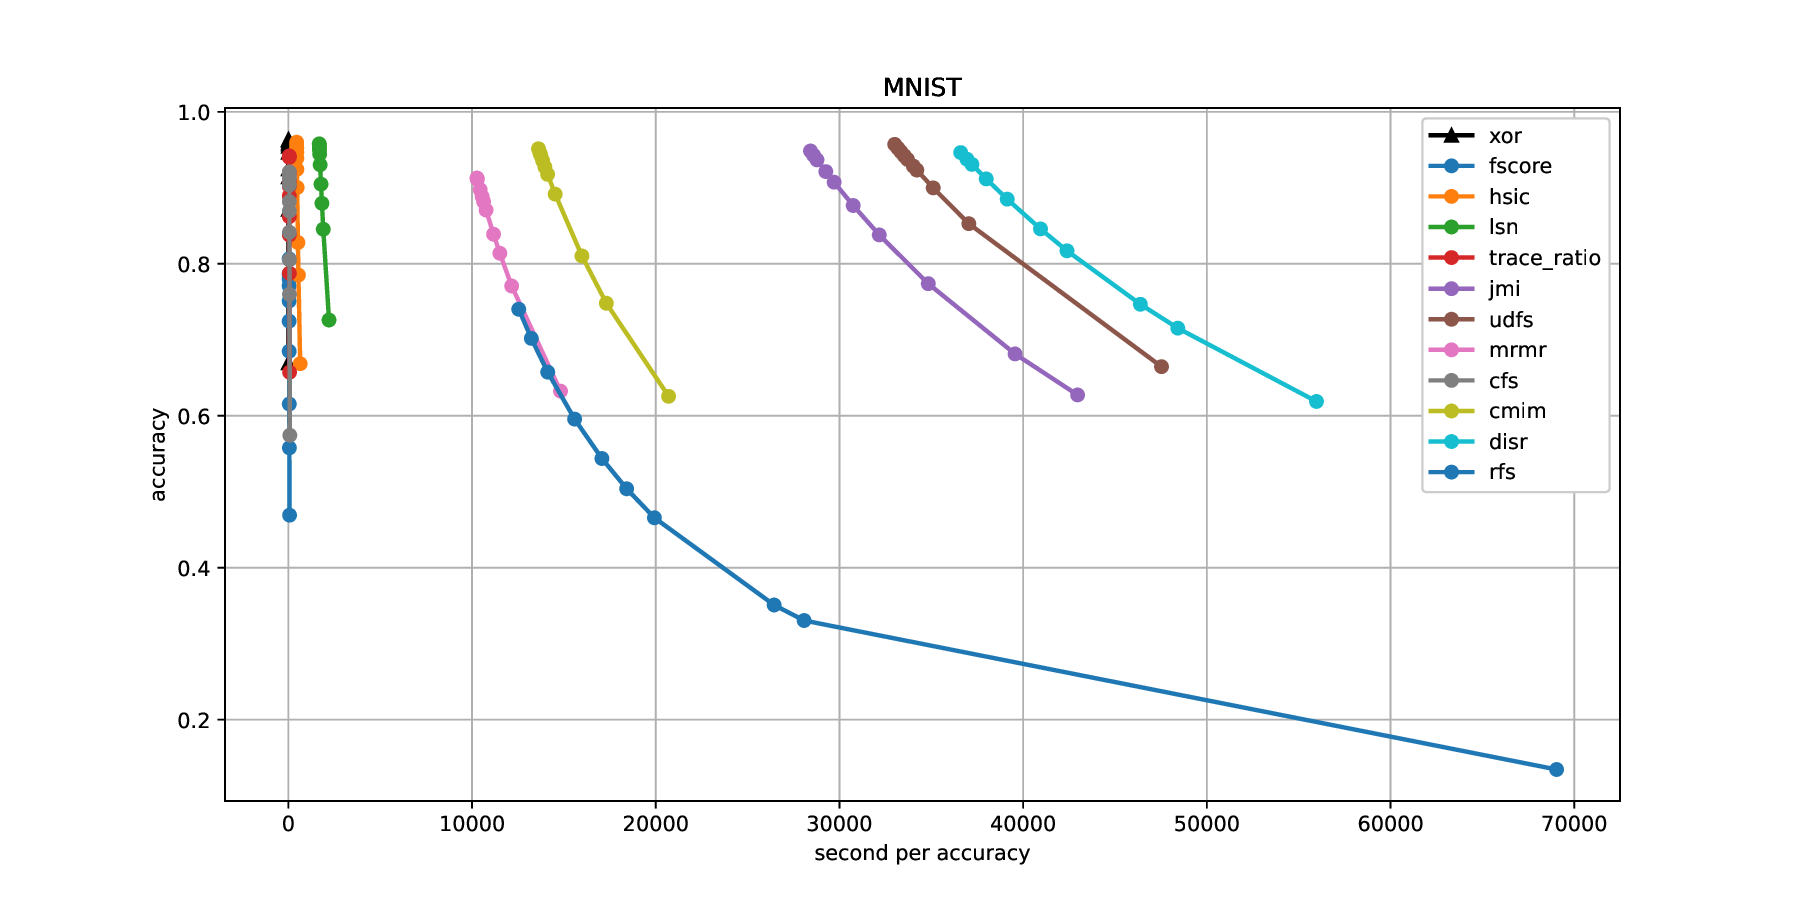}
		\caption{}	
	\end{subfigure}
	
	\begin{subfigure}[b]{0.48\textwidth}	%7
		\includegraphics[width=\textwidth]{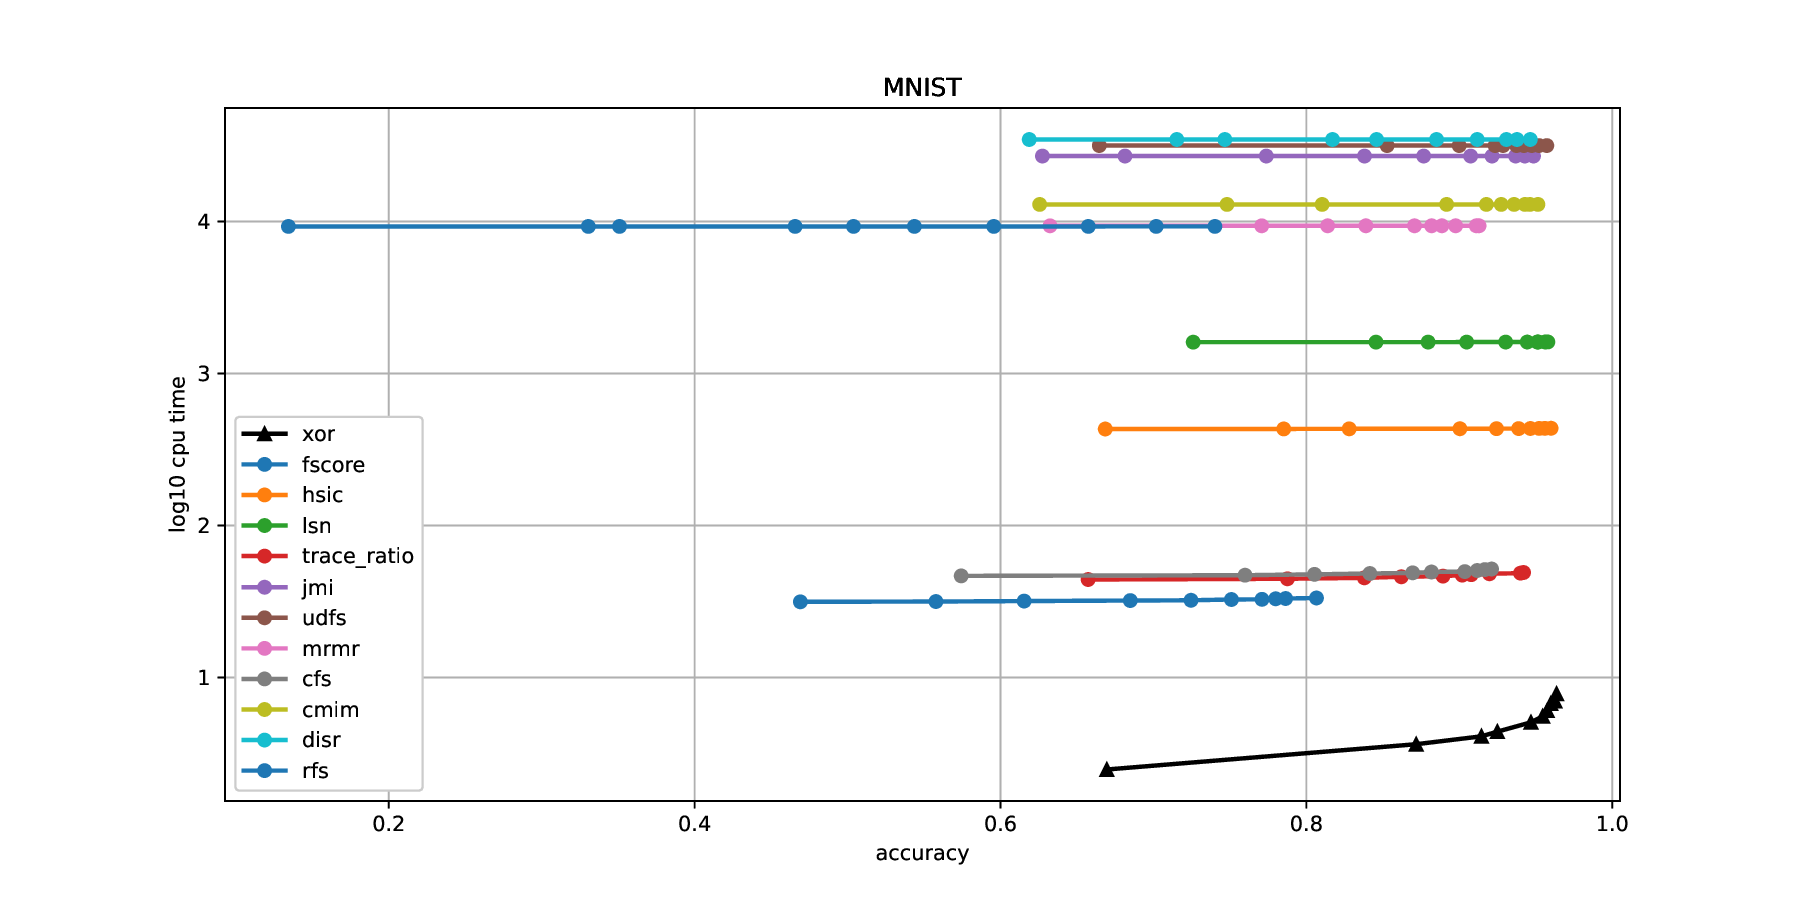}
		\caption{}
	\end{subfigure}
	\begin{subfigure}[b]{0.48\textwidth}	%8
		\includegraphics[width=\textwidth]{pic/mnist_log10_time_per_acc_log10_time.eps}
		\caption{}
	\end{subfigure}
	
	\begin{subfigure}[b]{0.48\textwidth}	%9
		\includegraphics[width=\textwidth]{pic/mnist_time_acc_per_time.eps}
		\caption{}
	\end{subfigure}
	\begin{subfigure}[b]{0.48\textwidth}	%10
		\includegraphics[width=\textwidth]{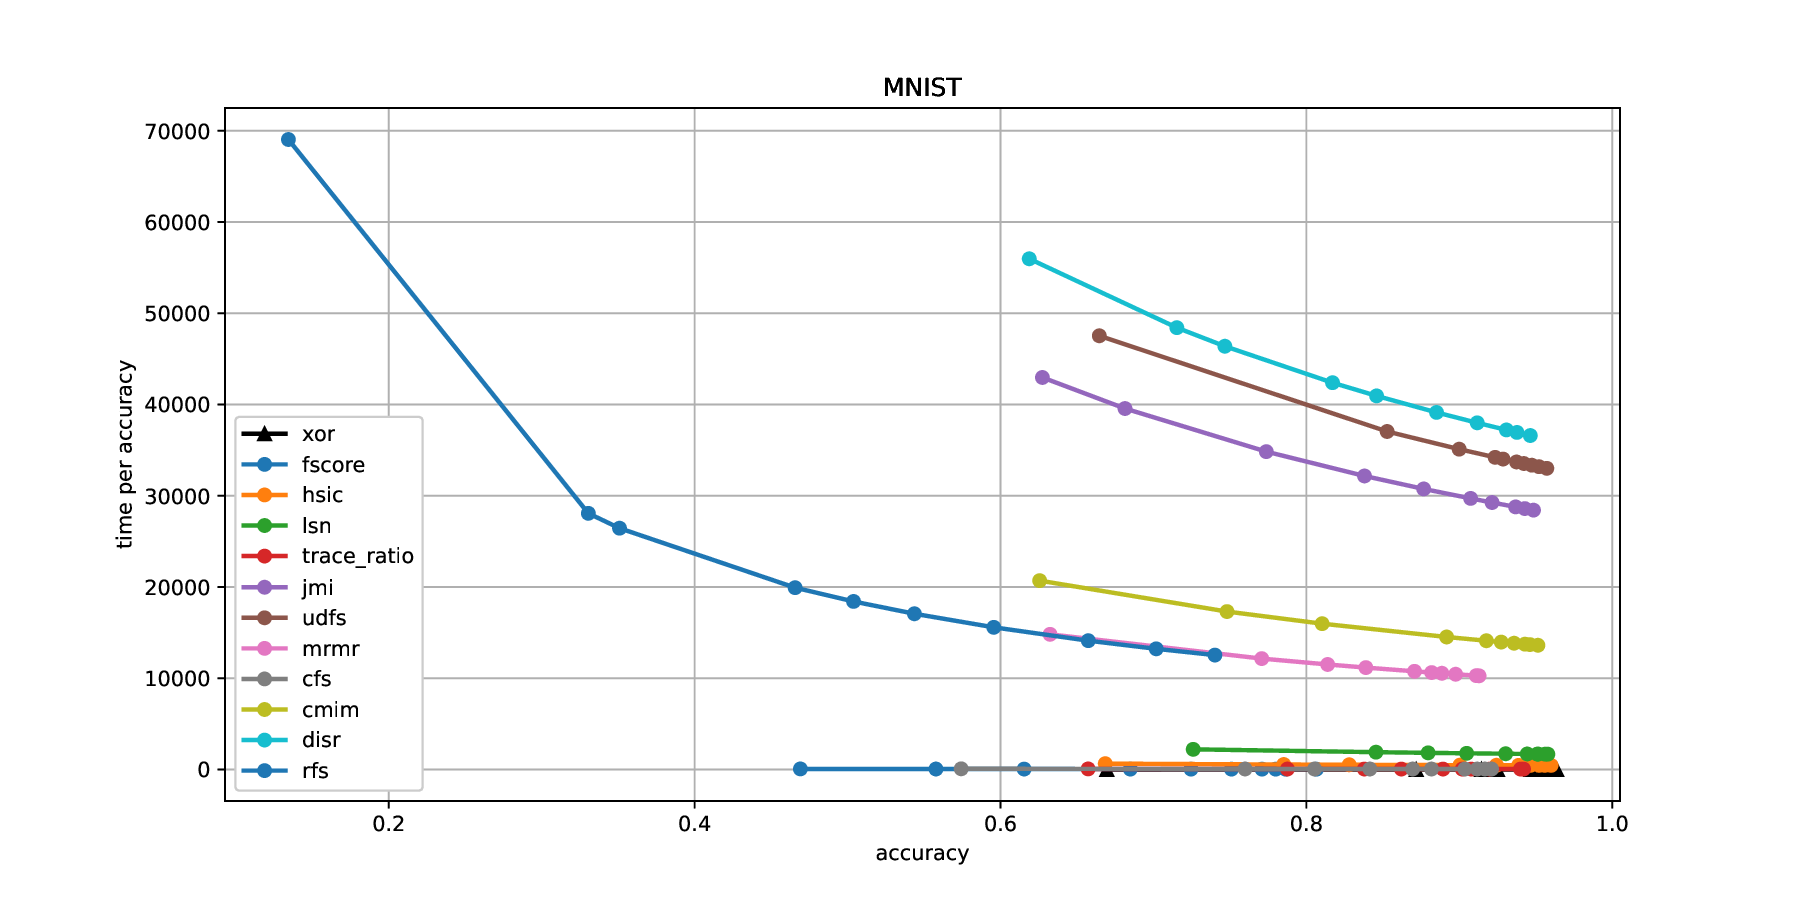}
		\caption{}
	\end{subfigure}
	
	\caption{Time consuming results on MNIST dataset.}
	\label{time_consuming_comparison_mnist}
\end{figure}

\begin{figure}[!h]
	\centering
	%\vspace{-2cm}
	%\hspace{-2cm}
	\begin{subfigure}[b]{0.48\textwidth}	%1
		\includegraphics[width=\textwidth]{pic/fashion_mnist_acc_acc_per_time.eps} 
		\caption{}
	\end{subfigure}
	\begin{subfigure}[b]{0.48\textwidth}%2
		\includegraphics[width=\textwidth]{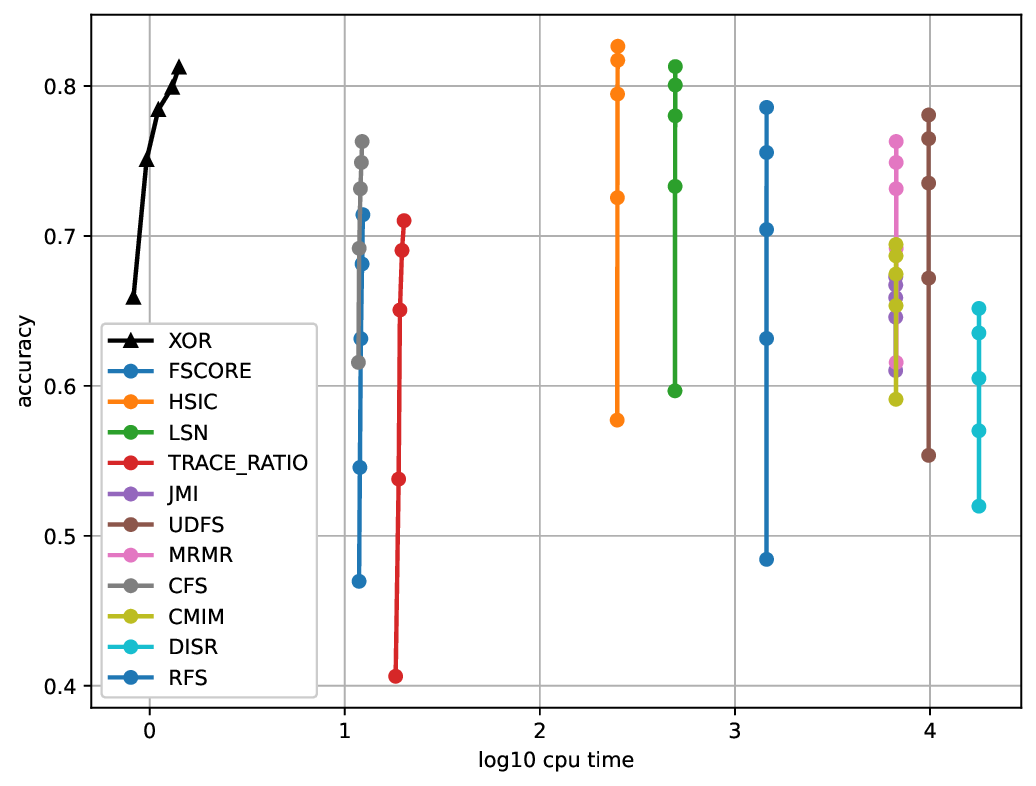}
		\caption{}
	\end{subfigure}
	
	\begin{subfigure}[b]{0.48\textwidth}	%3
		\includegraphics[width=\textwidth]{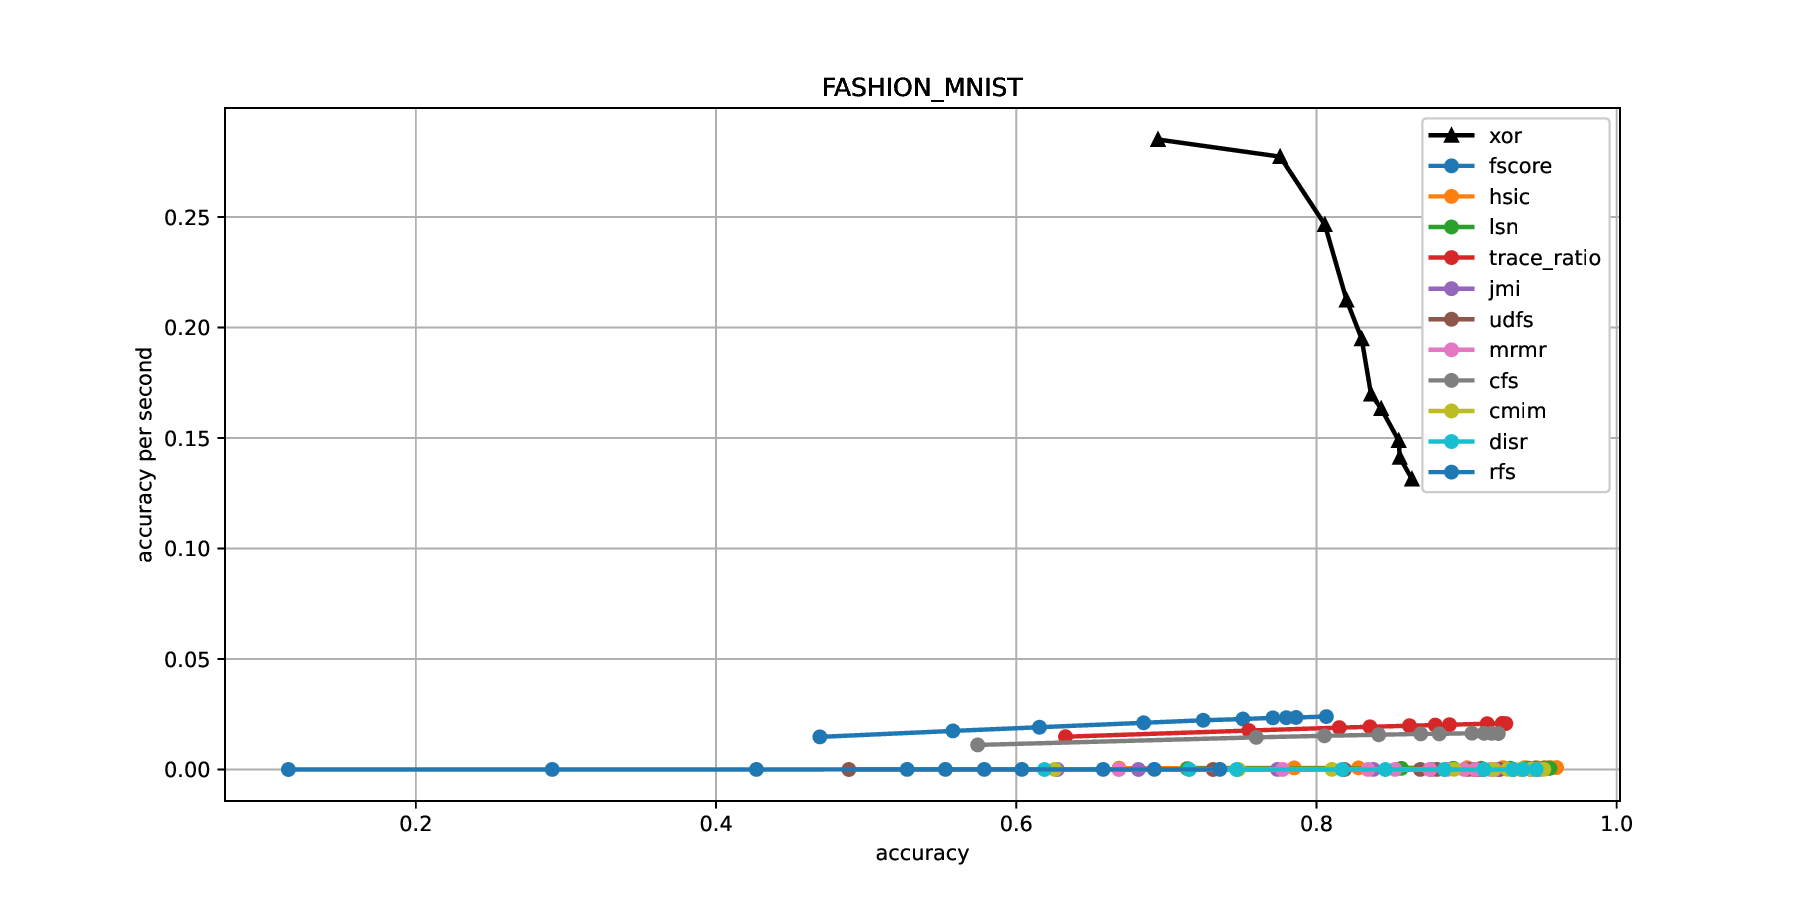}
		\caption{}
	\end{subfigure}
	\begin{subfigure}[b]{0.48\textwidth}	%4
		\includegraphics[width=\textwidth]{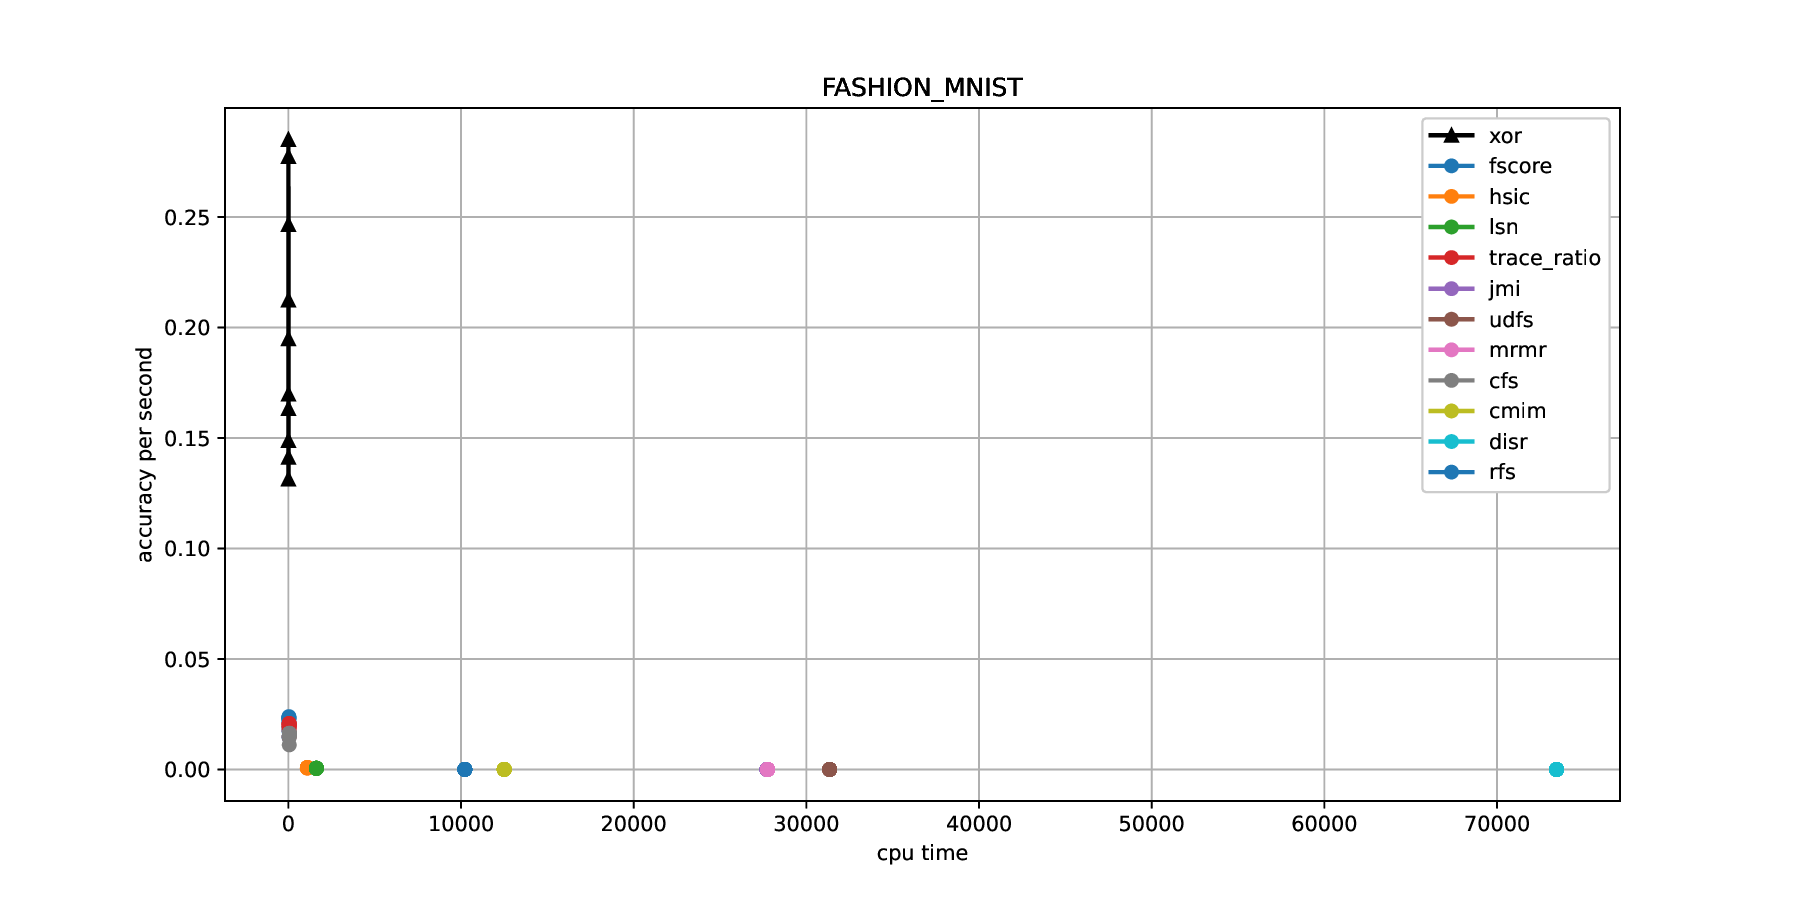}
		\caption{}
	\end{subfigure}
	
	\begin{subfigure}[b]{0.48\textwidth}%5
		\includegraphics[width=\textwidth]{pic/fashion_mnist_acc_per_time_time_per_acc.eps}
		\caption{}
	\end{subfigure}
	\begin{subfigure}[b]{0.48\textwidth}	%6
		\includegraphics[width=\textwidth]{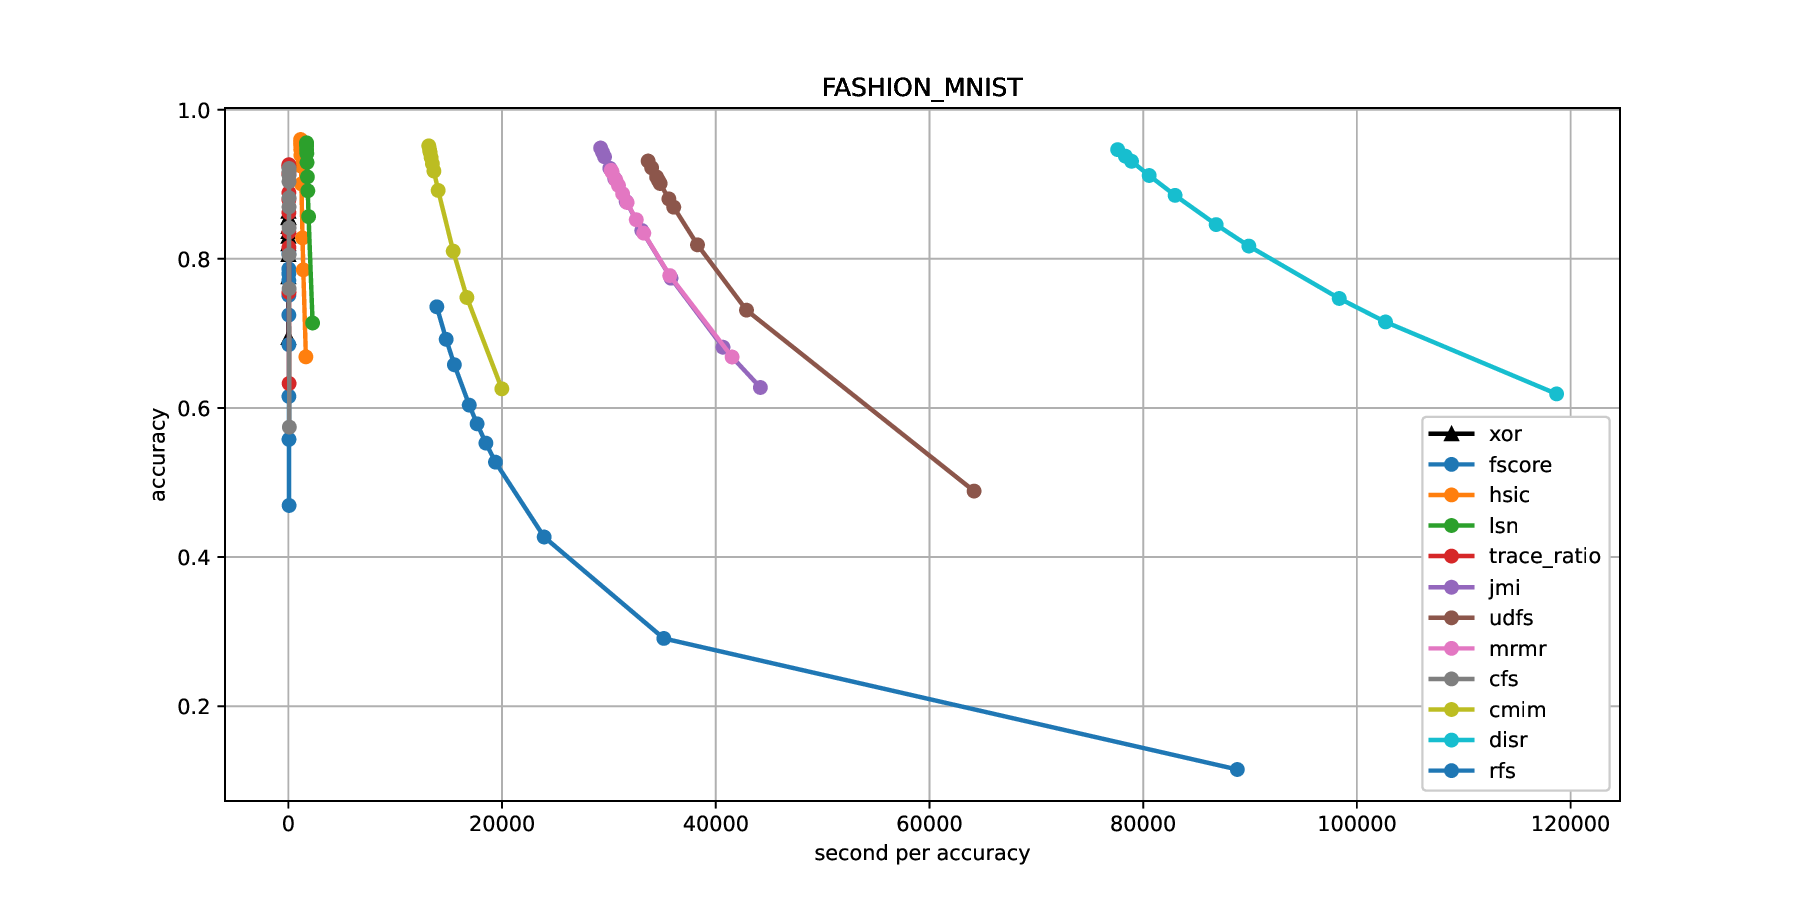}
		\caption{}	
	\end{subfigure}
	
	\begin{subfigure}[b]{0.48\textwidth}	%7
		\includegraphics[width=\textwidth]{pic/fashion_mnist_log10_time_acc.eps}
		\caption{}
	\end{subfigure}
	\begin{subfigure}[b]{0.48\textwidth}	%8
		\includegraphics[width=\textwidth]{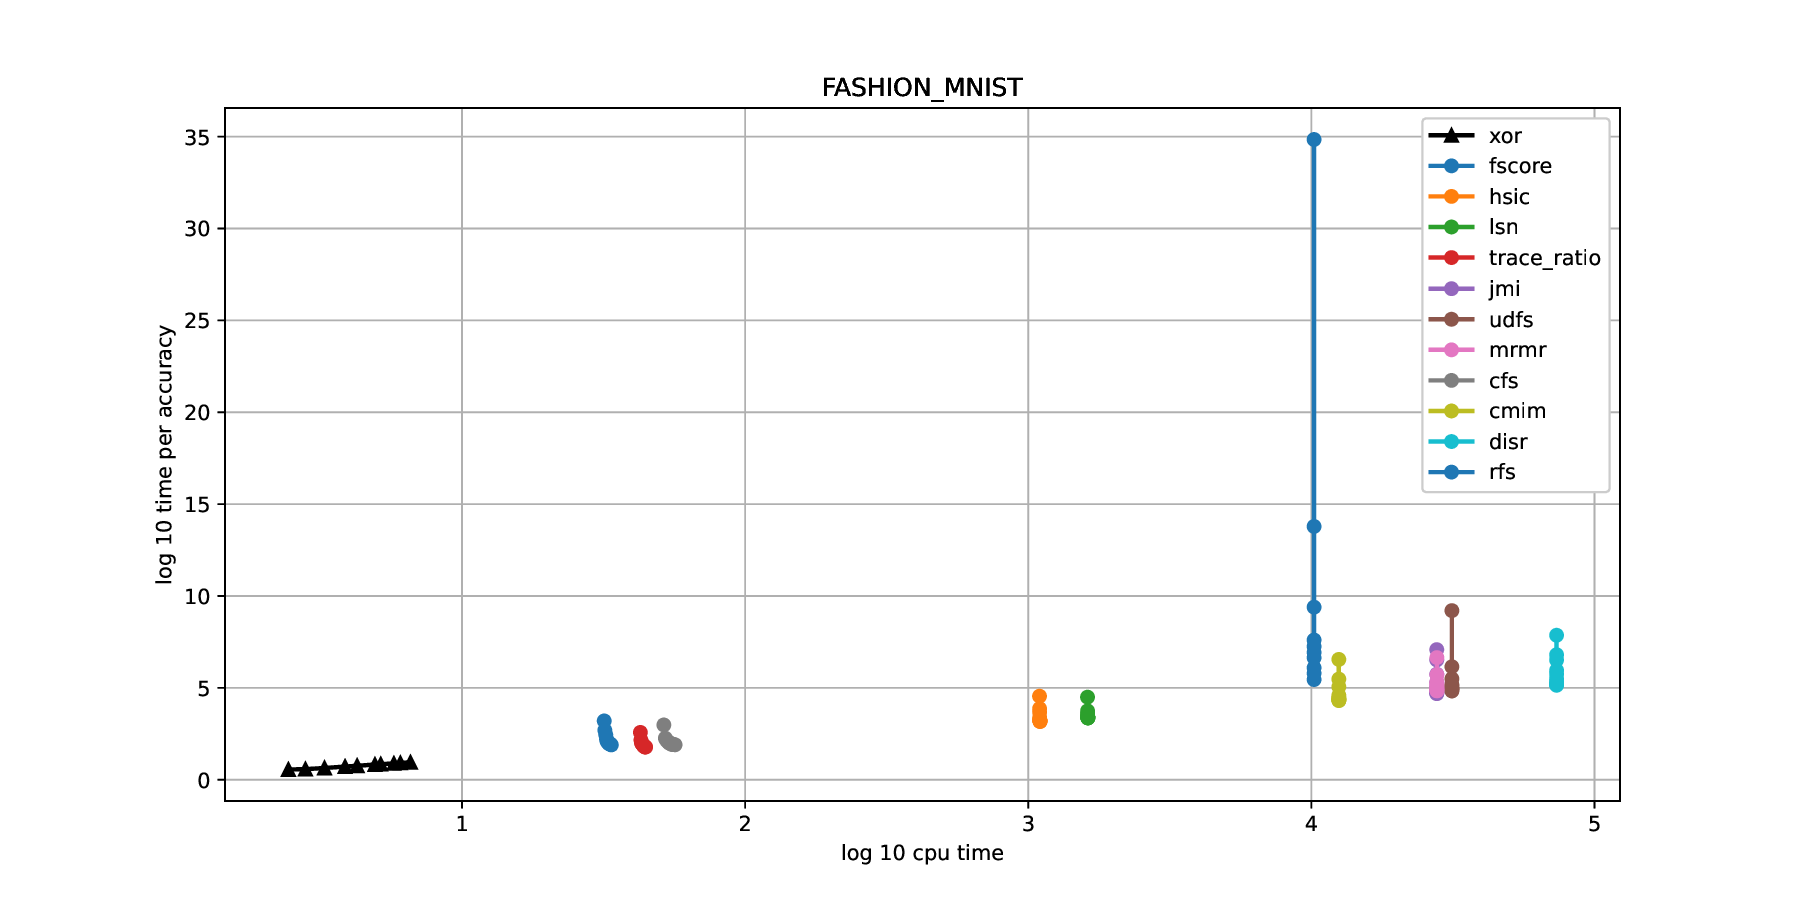}
		\caption{}
	\end{subfigure}
	
	\begin{subfigure}[b]{0.48\textwidth}	%9
		\includegraphics[width=\textwidth]{pic/fashion_mnist_time_acc_per_time.eps}
		\caption{}
	\end{subfigure}
	\begin{subfigure}[b]{0.48\textwidth}	%10
		\includegraphics[width=\textwidth]{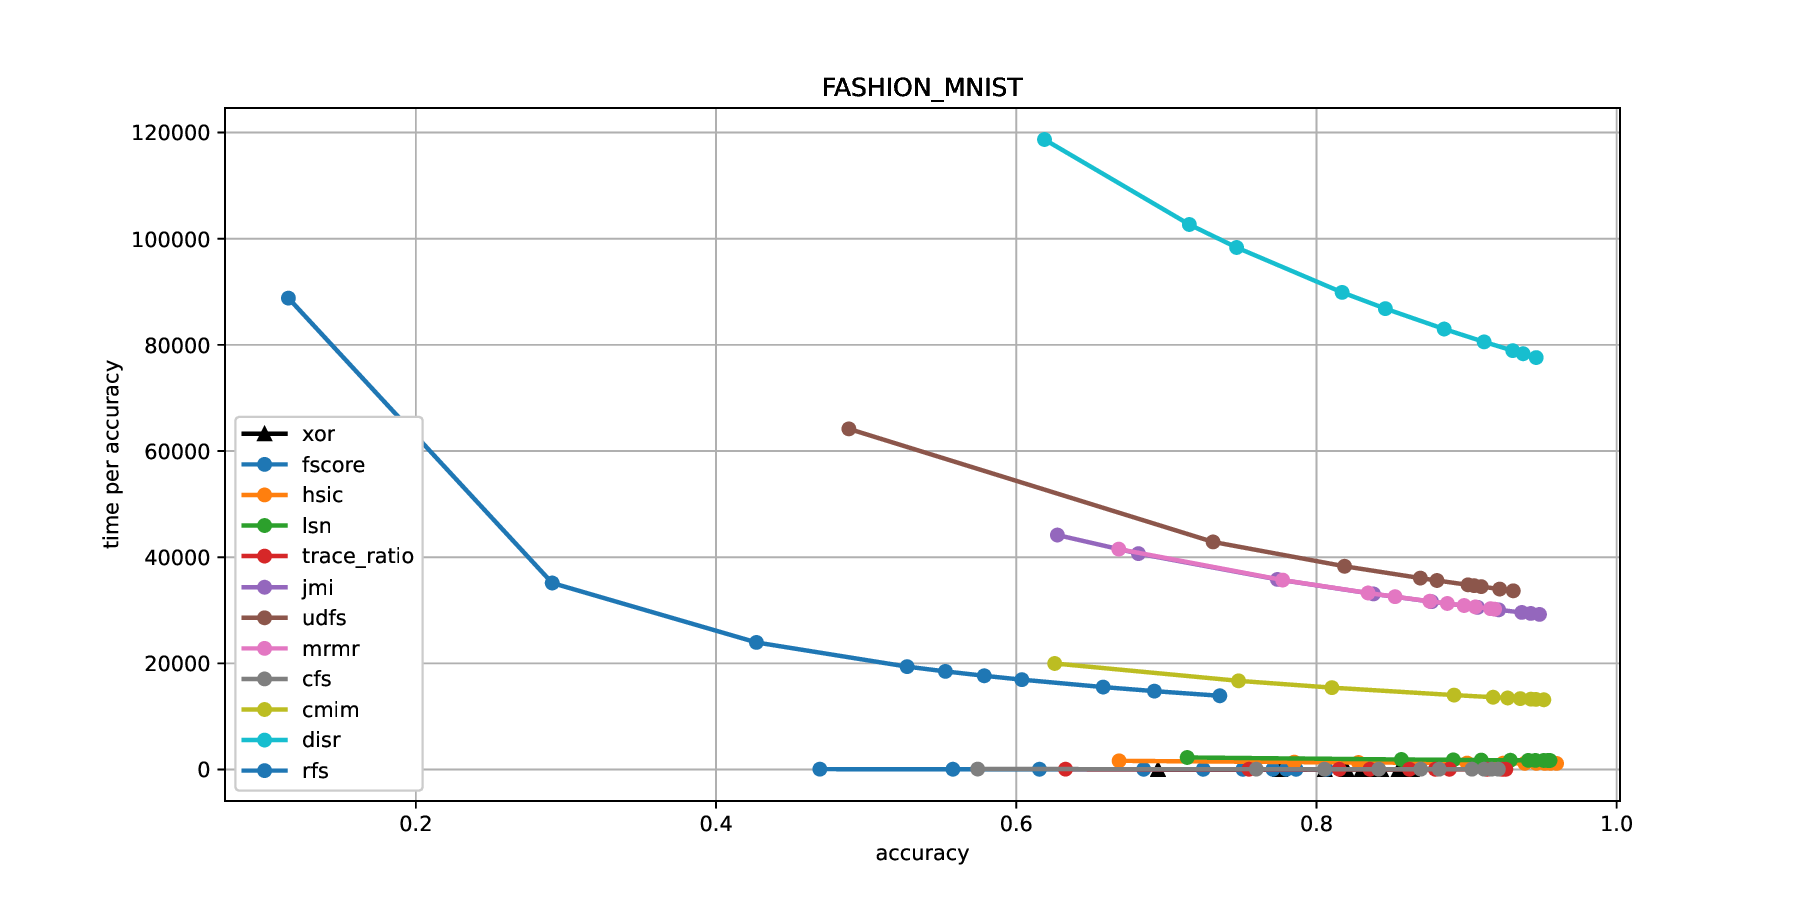}
		\caption{}
	\end{subfigure}
	
	\caption{Time consuming results on Fashion-MNIST dataset.}
	\label{time_consuming_comparison_fashion_mnist}
\end{figure}
